# Supplementary material for: Born-Oppenheimer potentials for $\Pi$, $\Delta$, and $\Phi$ states of the hydrogen molecule
Source: arXiv:2203.12080 ancillary file (2022-03-22)
Supplement: Supplementary file 1 [file supplement.pdf]

**SUPPLEMENTARY MATERIAL**

# Supplementary material to *Born-Oppenheimer potentials for $\Pi$, $\Delta$, and $\Phi$ states of the hydrogen molecule*

Michał Siłkowski[a] and Krzysztof Pachucki

*Faculty of Physics, University of Warsaw, Pasteura 5, 02-093 Warsaw, Poland*

(Version 0.2 dated: March 22, 2022)

Contents:
Tables S1 to S38 are 5 column wide, where the columns contain (in order): $R$, $E$, $\langle V\rangle$, $\langle\nabla_1\cdot\nabla_2\rangle$, $\mathrm{d}E/\mathrm{d}R$. All the quantities are given in atomic units. Each state is presented in a separate table,
Tables S1 to S16: $1-4\,\Pi$ states,
Tables S17 to S28: $1-3\,\Delta$ states,
Tables S29 to S38: $1-2\,\Phi$, $3\,{}^1\Phi_\mathrm{u}$, and $3\,{}^3\Phi_\mathrm{u}$ states.

[a] michal.silkowski@fuw.edu.pl

TABLE S1. Calculated BO energies, expectation value of potential, $\langle\nabla_1 \cdot \nabla_2\rangle$, and $\mathrm{d}E/\mathrm{d}R$ of the $1^1\Pi_g$ state in atomic units (hartree). Uncertainties originate purely from extrapolation to the complete basis set limit. United atom values at $R = 0$ are taken from Ref. [1].

| $1^1\Pi_g$ | | | | |
|---|---|---|---|---|
| $R$ | $E$ | $\langle V\rangle$ | $10^6 \cdot \langle\nabla_1 \cdot \nabla_2\rangle$ | $\mathrm{d}E/\mathrm{d}R$ |
| 0.0 | −2.055620732852246(6) | – | 249.3999921(1) | – |
| 0.01 | 97.94464058640(2) | 95.8897985410(2) | 249.523(3) | −9999.948263184(8) |
| 0.05 | 17.9504116140(3) | 15.912232428(3) | 252.367(2) | −399.77141603(5) |
| 0.1 | 7.96614323261(8) | 5.971361504(3) | 260.412(2) | −99.60904962(2) |
| 0.15 | 4.6553158497(2) | 2.719322944(2) | 272.618(3) | −43.942058368(5) |
| 0.2 | 3.015754379264(7) | 1.1467034992(4) | 288.425(3) | −24.423926297(2) |
| 0.3 | 1.4109876731(2) | −0.31676629408(5) | 329.669(3) | −10.46240546760(10) |
| 0.4 | 0.6435828674310(2) | −0.947599026340(5) | 382.980(4) | −5.586861903004(9) |
| 0.5 | 0.209322338243(4) | −1.2572025107527(7) | 448.376(5) | −3.351654374485(2) |
| 0.6 | −0.060539402480564(4) | −1.4160157732823(2) | 526.515(5) | −2.1581949472019(3) |
| 0.7 | −0.238393084120199(3) | −1.495929863340(4) | 618.474(6) | −1.455948135860(7) |
| 0.8 | −0.360290592374370(4) | −1.531757474788(9) | 725.6747(10) | −1.013995362548(9) |
| 0.9 | −0.4461288093169766(2) | −1.541950211832(2) | 849.8240(10) | −0.721902881331(2) |
| 1.0 | −0.507698297532046(3) | −1.536925637121(7) | 992.9701(6) | −0.521549042057(5) |
| 1.1 | −0.552383677344524(2) | −1.522842016503(6) | 1157.4989(7) | −0.380086056195(4) |
| 1.2 | −0.585012709686148(3) | −1.503465896063(6) | 1346.1899(2) | −0.277883730575(4) |
| 1.3 | −0.608852186979388(2) | −1.481159682383(6) | 1562.2711(3) | −0.202673314172(4) |
| 1.4 | −0.626176016107194(4) | −1.457431948840(6) | 1809.5006(3) | −0.146499940447(4) |
| 1.5 | −0.638604793189250(2) | −1.433257320895(2) | 2092.2591(5) | −0.1040451563444(10) |
| 1.6 | −0.647316835137268(4) | −1.409269013823(2) | 2415.6695(5) | −0.0716595897179(9) |
| 1.7 | −0.653183706517060(2) | −1.385878159319(9) | 2785.74210(9) | −0.046782791932(5) |
| 1.8 | −0.656859740520023(5) | −1.363349631624(9) | 3209.55351(10) | −0.027583416991(5) |
| 1.9 | −0.658842632362324(2) | −1.341851299313(9) | 3695.4727(2) | −0.012729491888(4) |
| 2.0 | −0.659515340754017(6) | −1.32148666268(2) | 4253.4349(2) | −0.001237990588(5) |
| 2.1 | −0.659175620023221(3) | −1.30231690829(2) | 4895.2844(2) | 0.007625872265(5) |
| 2.2 | −0.658057193711391(7) | −1.28437613052(2) | 5635.1985(2) | 0.014417389502(5) |
| 2.3 | −0.656345175033174(3) | −1.26768211147(2) | 6490.2105(2) | 0.019560103737(5) |
| 2.4 | −0.654187463248630(8) | −1.252244223916(5) | 7480.8527(2) | 0.023379459409(2) |
| 2.5 | −0.651703286081417(4) | −1.238069509824(5) | 8631.9361(2) | 0.026126824936(2) |
| 2.6 | −0.648989694529758(9) | −1.225167661976(5) | 9973.4782(2) | 0.027996818109(2) |
| 2.7 | −0.646126575090967(4) | −1.213555419303(5) | 11541.7719(2) | 0.029139900326(2) |
| 2.8 | −0.643180581113649(10) | −1.20326072123(2) | 13380.5435(2) | 0.029671586070(6) |
| 2.9 | −0.640208271512076(5) | −1.19432679988(2) | 15542.0631(2) | 0.029679221775(6) |
| 3.0 | −0.637258662449248(10) | −1.186816158137(9) | 18087.9179(2) | 0.029233722254(2) |
| 3.1 | −0.634375331677092(4) | −1.18081399722(3) | 21088.8795(2) | 0.028360214883(6) |
| 3.2 | −0.631598153855495(10) | −1.17642999892(3) | 24622.8721(2) | 0.027108221499(6) |
| 3.3 | −0.628964676764191(4) | −1.17379631274(3) | 28769.4551(2) | 0.025488800238(6) |
| 3.4 | −0.626511063061438(8) | −1.1730581475890(7) | 33598.6320(7) | 0.02351293486300(2) |
| 3.5 | −0.6242724190517674(3) | −1.1743519801153(7) | 39151.7171(5) | 0.021192245139593(9) |
| 3.6 | −0.622282235211503(7) | −1.1777665431815(6) | 45413.5353(4) | 0.018549424233847(9) |
| 3.7 | −0.6205706474226789(2) | −1.1832862801634(6) | 52279.9757(3) | 0.01563108504926(2) |
| 3.8 | −0.6191514231607989(2) | −1.1907285798419(6) | 59533.0434(3) | 0.01251954381048(2) |
| 3.9 | −0.61806809151767972(9) | −1.1997023807010(9) | 66842.8232(2) | 0.00933687239350(9) |
| 4.0 | −0.6172903557001000(2) | −1.209623294356(2) | 73812.1075(2) | 0.0062343542611(3) |
| 4.1 | −0.61680236035624(2) | −1.2198014186189(3) | 80058.06987(8) | 0.00336665904723(5) |
| 4.2 | −0.61659394644281(2) | −1.2295749041901(4) | 85297.92785(4) | 0.00086023540369(7) |
| 4.3 | −0.61661473822808(6) | −1.2384300938752(10) | 89398.53653(2) | −0.00120944591128(9) |
| 4.4 | −0.61681964617742(5) | −1.2460600263929(8) | 92373.1491(7) | −0.0028228940996(2) |
| 4.5 | −0.6171740315935651(2) | −1.252354957700(4) | 94339.90681(2) | −0.0040059765584(6) |
| 4.6 | −0.61760738504809(5) | −1.2573517874(2) | 95469.695(3) | −0.00481239510(7) |
| 4.7 | −0.61811525621423(2) | −1.261174570033(4) | 95943.811062(4) | −0.0053072462988(7) |
| 4.8 | −0.618659769917686(6) | −1.2639857852(2) | 95928.1752(10) | −0.00555546777(2) |
| 4.9 | −0.61921925170919(2) | −1.2659541495(3) | 95562.0306(8) | −0.00561543796(3) |
| 5.0 | −0.6197874182528645(4) | −1.267236867755(3) | 94955.857480(7) | −0.0055364062499(5) |

| $1^1\Pi_g$ continued | | | | |
|---|---|---|---|---|
| $R$ | $E$ | $\langle V\rangle$ | $10^6 \cdot \langle\nabla_1 \cdot \nabla_2\rangle$ | $\mathrm{d}E/\mathrm{d}R$ |
| 5.1 | −0.620322437421447(4) | −1.2679718288(4) | 94194.0423(6) | −0.00535822624(5) |
| 5.2 | −0.620846026668478(6) | −1.2682756671(5) | 93339.2962(6) | −0.00511223339(6) |
| 5.3 | −0.62134266489907(8) | −1.2682448430(6) | 92437.2239(6) | −0.00482254964(7) |
| 5.4 | −0.621808939076557(7) | −1.2679580036(6) | 91520.3617(7) | −0.00450743061(9) |
| 5.5 | −0.6222530198410015(3) | −1.2674786869(7) | 90611.4664(8) | −0.00418048129(10) |
| 5.6 | −0.62264424934149(8) | −1.2668579106046(8) | 89726.0792249(6) | −0.00385168070028(2) |
| 5.7 | −0.623012821742175(9) | −1.2661364598(10) | 88874.4681(10) | −0.0035282133(2) |
| 5.8 | −0.62334953797260(4) | −1.265346811(2) | 88063.085(2) | −0.0032151266(2) |
| 5.9 | −0.623655618866059(10) | −1.2645147281691(8) | 87295.6319896(6) | −0.00291584583674(10) |
| 6.0 | −0.6239425636994983(7) | −1.26366056309(3) | 86573.85020(4) | −0.002632572615(3) |
| 6.5 | −0.624950855257195(9) | −1.259507401581(5) | 83634.613639(8) | −0.0014808755486(5) |
| 7.0 | −0.625488515522114(3) | −1.2561045375371(8) | 81649.1164813(4) | −0.0007325009277(3) |
| 7.5 | −0.625733432092477(3) | −1.25362710222(3) | 80354.852163(6) | −0.000288031739(5) |
| 8.0 | −0.625809393436053(2) | −1.2519515441(2) | 79530.17202(9) | −0.00004159466(3) |
| 8.5 | −0.625795151273442(2) | −1.25088281746(2) | 79013.262197(2) | 0.000083233539(2) |
| 9.0 | −0.6257378199140553(8) | −1.250238427949(5) | 78692.8532201(6) | 0.0001374679863(8) |
| 9.5 | −0.6256640568552325(9) | −1.249874263060(5) | 78495.2236093(2) | 0.0001530369104(6) |
| 10.0 | −0.6255880139309715(6) | −1.2496864991391(6) | 78372.9286996(5) | 0.00014895287227(7) |
| 11.0 | −0.62545247254346736(9) | −1.249583860023(2) | 78246.7110450(7) | 0.0001200986421(2) |
| 12.0 | −0.62534812481753221(8) | −1.2496228004782(7) | 78189.9762572(5) | 0.00008945409639(7) |
| 13.0 | −0.62527125012850115(4) | −1.2496907379325(3) | 78158.4589808(5) | 0.00006552017880(3) |
| 14.0 | −0.625214829096054525(9) | −1.24975327550001(8) | 78137.1353153(3) | 0.000048313049432(9) |
| 15.0 | −0.625172937458233213(4) | −1.24980326081155(2) | 78120.9282186(3) | 0.000036174273659(4) |
| 16.0 | −0.625141309348841379(2) | −1.24984159110974(2) | 78107.9681790(3) | 0.0000275642242459(2) |
| 17.0 | −0.6251170092209620277(10) | −1.24987080184524(3) | 78097.3996064(2) | 0.0000213656821592(2) |
| 18.0 | −0.6250980286814565856(5) | −1.24989323672651(4) | 78088.7079192(2) | 0.0000168233686904(3) |
| 19.0 | −0.6250829796118870796(3) | −1.24991069220359(4) | 78081.52089339(6) | 0.0000134351063269(3) |
| 20.0 | −0.6250708868292175202(2) | −1.24992446796585(5) | 78075.54818409(2) | 0.0000108652846306(5) |

TABLE S2. Calculated BO energies, expectation value of potential, $\langle\nabla_1\cdot\nabla_2\rangle$, and $\mathrm{d}E/\mathrm{d}R$ of the $2^1\Pi_g$ state in atomic units (hartree). Uncertainties originate purely from extrapolation to the complete basis set limit. United atom values at $R=0$ are taken from Ref. [1].

| $2^1\Pi_\mathrm{g}$ | | | | |
|---|---|---|---|---|
| $R$ | $E$ | $\langle V\rangle$ | $10^6\cdot\langle\nabla_1\cdot\nabla_2\rangle$ | $\mathrm{d}E/\mathrm{d}R$ |
| 0.0 | −2.031279846178687(7) | – | 129.1751887(8) | – |
| 0.01 | 97.96898149748(5) | 95.9384804119(4) | 129.20(2) | −9999.94825831(3) |
| 0.05 | 17.974743084(3) | 15.96091651(2) | 130.67(2) | −399.7713932(3) |
| 0.1 | 7.990476325(4) | 6.02005190(3) | 134.80(3) | −99.6090075(2) |
| 0.15 | 4.679661482(3) | 2.76802313(2) | 141.07(3) | −43.94199892(8) |
| 0.2 | 3.040093391(2) | 1.195416640(9) | 149.17(3) | −24.42385071(4) |
| 0.3 | 1.4353357683(4) | −0.268018379(3) | 170.29(3) | −10.462299719(6) |
| 0.4 | 0.6679429860(2) | −0.8988049477(8) | 197.56(3) | −5.586727299(2) |
| 0.5 | 0.23369734525(5) | −1.2083509101(3) | 230.98(3) | −3.3514912011(5) |
| 0.6 | −0.03614663925(2) | −1.3670950254(2) | 270.86(3) | −2.1580029115(2) |
| 0.7 | −0.21396964720(8) | −1.4469278846(9) | 316.5(6) | −1.4556979860(10) |
| 0.8 | −0.335843480423(7) | −1.48266156315(4) | 372.39(5) | −1.01371825287(3) |
| 0.9 | −0.421654908186(5) | −1.49274689223(4) | 435.64(8) | −0.721596750959(2) |
| 1.0 | −0.483194352338(4) | −1.487600491347(7) | 508.68(4) | −0.5212117866713(5) |
| 1.1 | −0.527846263528(4) | −1.473379491779(8) | 592.56(5) | −0.37971542247515(3) |
| 1.2 | −0.560438201388(4) | −1.45384908150(2) | 688.78(5) | −0.277477232274(3) |
| 1.3 | −0.584236721495(7) | −1.43137004591(4) | 798.90(9) | −0.20222815609(2) |
| 1.4 | −0.601515453262(4) | −1.407449024795(3) | 925.20(4) | −0.146012941627(3) |
| 1.5 | −0.613894668415(4) | −1.383058338024(4) | 1069.63(4) | −0.103512667467(3) |
| 1.6 | −0.622552304911(4) | −1.358828450219(3) | 1234.96(4) | −0.071077400253(3) |
| 1.7 | −0.628359484639(2) | −1.335167209346(6) | 1424.36(4) | −0.046146023571(2) |
| 1.8 | −0.631970023438(4) | −1.312335566114(9) | 1641.57(3) | −0.0268863995767(5) |
| 1.9 | −0.633881011453(3) | −1.290496696858(8) | 1891.03(3) | −0.0119656178701(2) |
| 2.0 | −0.634474699096(2) | −1.269748485726(8) | 2178.03(3) | −0.0003995437677(4) |
| 2.1 | −0.634048010803(2) | −1.250145393312(10) | 2508.95(3) | 0.0085479182349(6) |
| 2.2 | −0.632833696942(5) | −1.23171345756(2) | 2891.48(3) | 0.015433607419(2) |
| 2.3 | −0.631015728869(2) | −1.21446081535(2) | 3334.92(3) | 0.020682887998(2) |
| 2.4 | −0.628740665838(3) | −1.19838530967(2) | 3850.56(3) | 0.024623342500(3) |
| 2.5 | −0.626126163784(2) | −1.18348024143(2) | 4452.14(3) | 0.027508834455(3) |
| 2.6 | −0.623267432745(3) | −1.16973901006(3) | 5156.41(3) | 0.029536867471(4) |
| 2.7 | −0.620242209025(2) | −1.15715918799(3) | 5983.62(3) | 0.030861196317(4) |
| 2.8 | −0.6171146462161(8) | −1.14574643036(3) | 6958.07(3) | 0.031601022170(5) |
| 2.9 | −0.613938417248(2) | −1.13551847539(3) | 8108.32(3) | 0.031847710038(5) |
| 3.0 | −0.6107592382490(3) | −1.12650924557(3) | 9466.59(3) | 0.031669743645(5) |
| 3.1 | −0.607616958029(6) | −1.11877254279(3) | 11066.46(3) | 0.031116572023(5) |
| 3.2 | −0.604547286532(4) | −1.11238372680(4) | 12937.01(3) | 0.030222139461(7) |
| 3.3 | −0.6015831388247(9) | −1.10743560675(5) | 15090.430(6) | 0.029009294213(9) |
| 3.4 | −0.598755419516(7) | −1.10402122711(5) | 17499.1(2) | 0.027496944682(10) |
| 3.5 | −0.596092853521(2) | −1.10219239180(7) | 20060.64(2) | 0.02571237578(2) |
| 3.6 | −0.593620257975(3) | −1.1018843390(3) | 22552.5(2) | 0.02371004917(6) |
| 3.7 | −0.59135474883(2) | −1.1028169415(3) | 24610.17(6) | 0.02159258274(5) |
| 3.8 | −0.58930033248(2) | −1.1044302537(4) | 25768.1(2) | 0.01951852929(7) |
| 3.9 | −0.587443305895(2) | −1.1059524040(5) | 25610.29(8) | 0.01767543792(6) |
| 4.0 | −0.585752331321(3) | −1.1066394141(5) | 23965.67(3) | 0.01621631218(8) |
| 4.1 | −0.584185223090(6) | −1.10605884822(8) | 21012.8(10) | 0.01519795072(2) |
| 4.2 | −0.582699683556(6) | −1.10420939855(8) | 17201.1(10) | 0.01456904013(2) |
| 4.3 | −0.581262361898(6) | −1.10141543864(7) | 13048.4(9) | 0.01421146166(2) |
| 4.4 | −0.579852676674(4) | −1.09812163741(5) | 8980.7(10) | 0.013996299078(9) |
| 4.5 | −0.578461827788(3) | −1.0947306592(4) | 5267.75(4) | 0.01382066587(6) |
| 4.6 | −0.577089453604(5) | −1.09153231092(5) | 2029.9(9) | 0.013618825279(9) |
| 4.7 | −0.575740073294(5) | −1.08870032059(5) | −704.6(9) | 0.013357409786(9) |
| 4.8 | −0.574420336517(4) | −1.08631837819(3) | −2967.9(9) | 0.013025478092(5) |
| 4.9 | −0.573137258629(4) | −1.08441040008(3) | −4813.3(3) | 0.012625330036(5) |
| 5.0 | −0.571897247968(2) | −1.08296480632(7) | −6302.97(2) | 0.012165937925(9) |

| $2^1\Pi_g$ continued | | | | |
|---|---|---|---|---|
| $R$ | $E$ | $\langle V \rangle$ | $10^6 \cdot \langle \nabla_1 \cdot \nabla_2 \rangle$ | $\mathrm{d}E/\mathrm{d}R$ |
| 5.1 | −0.570705660189(4) | −1.08195103980(3) | −7494.1(3) | 0.011658878544(5) |
| 5.2 | −0.569566662857(4) | −1.08132974701(3) | −8435.3(3) | 0.011116072828(5) |
| 5.3 | −0.568483264306(4) | −1.08105861036(3) | −9168.7(3) | 0.010548663820(5) |
| 5.4 | −0.567457418740(4) | −1.08109547131(3) | −9728.4(3) | 0.009966549291(4) |
| 5.5 | −0.5664901587152(8) | −1.08139987277(9) | −10141.763(8) | 0.00937826267(2) |
| 5.6 | −0.565581729976(4) | −1.08193373059(3) | −10431.9(3) | 0.008791023100(4) |
| 5.7 | −0.564731717180(4) | −1.08266155588(3) | −10616.2(3) | 0.008210855874(4) |
| 5.8 | −0.563939156335(4) | −1.08355046687(3) | −10709.5(3) | 0.007642732035(4) |
| 5.9 | −0.563202633402(4) | −1.08457012074(3) | −10724.1(3) | 0.007090702723(4) |
| 6.0 | −0.5625203701836(6) | −1.085692630102(10) | −10670.008(2) | 0.006558018378(2) |
| 6.5 | −0.5598439170224(5) | −1.092036477110(7) | −9646.733(2) | 0.0042540549132(7) |
| 7.0 | −0.5581563807460(4) | −1.098092696105(6) | −7889.0820(7) | 0.0026028664840(5) |
| 7.5 | −0.5571442316310(4) | −1.102812526808(5) | −5897.17227(10) | 0.0015301248606(4) |
| 8.0 | −0.5565555381049(3) | −1.106054491074(4) | −3964.8422(3) | 0.0008820731421(3) |
| 8.5 | −0.5562164399864(3) | −1.108100153648(3) | −2235.7590(6) | 0.0005097325089(2) |
| 9.0 | −0.5560185449046(3) | −1.109316439703(3) | −779.9190(7) | 0.0003022944563(2) |
| 9.5 | −0.5558987748977(2) | −1.110011142256(2) | 342.0609(7) | 0.00018804289894(8) |
| 10.0 | −0.5558221945781(2) | −1.110401969994(2) | 1033.0662(7) | 0.00012424191619(10) |
| 11.0 | −0.5557335542238(2) | −1.110795088842(3) | 149.9926(5) | 0.0000610926914(2) |
| 12.0 | −0.5556957026404(4) | −1.111155764032(6) | 920.4134(6) | 0.0000196367708(4) |
| 13.0 | −0.55567702488107(7) | −1.1110967472276(8) | 5349.58440(8) | 0.00001979250266(4) |
| 14.0 | −0.5556565510545(2) | −1.111025483731(2) | 6841.98756(7) | 0.00002054416987(5) |
| 15.0 | −0.5556368480510(4) | −1.110995120281(3) | 7750.579152(7) | 0.00001857172142(10) |
| 16.0 | −0.5556197371646(2) | −1.110990183924(2) | 8566.24287(9) | 0.00001558065033(3) |
| 17.0 | −0.5556057060000(2) | −1.1109986676740(9) | 9432.99453(3) | 0.000012514372126(2) |
| 18.0 | −0.55559459594413(5) | −1.11101320824144(9) | 10407.6213(3) | 0.00000977686925(2) |
| 19.0 | −0.55558599811026(9) | −1.11102953652340(5) | 11503.55681(3) | 0.00000749787876(2) |
| 20.0 | −0.55557944576008(7) | −1.11104527987147(6) | 12689.85889(2) | 0.00000568058241(2) |

TABLE S3. Calculated BO energies, expectation value of potential, $\langle\nabla_1\cdot\nabla_2\rangle$, and $\mathrm{d}E/\mathrm{d}R$ of the $3^1\Pi_g$ state in atomic units (hartree). Uncertainties originate purely from extrapolation to the complete basis set limit. United atom values at $R=0$ are taken from Ref. [1].

| $3^1\Pi_\mathrm{g}$ | | | | |
|---|---|---|---|---|
| $R$ | $E$ | $\langle V\rangle$ | $10^6\cdot\langle\nabla_1\cdot\nabla_2\rangle$ | $\mathrm{d}E/\mathrm{d}R$ |
| 0.0 | −2.020015836159984(4) | – | 71.883131(6) | – |
| 0.01 | 97.98024551692(8) | 95.9610084699(6) | 71.9085(10) | −9999.94825640(4) |
| 0.05 | 17.986007318(5) | 15.98344542(3) | 72.4(2) | −399.7713843(4) |
| 0.1 | 8.001741175(7) | 6.04258320(5) | 74.999(7) | −99.6089915(4) |
| 0.15 | 4.690927296(7) | 2.79055814(5) | 78.473(6) | −43.9419764(3) |
| 0.2 | 3.051360481(4) | 1.21795653(3) | 82.98(2) | −24.42382214(8) |
| 0.3 | 1.446606285(2) | −0.245465395(8) | 94.68(3) | −10.46225988(2) |
| 0.4 | 0.6792180268(5) | −0.876234624(4) | 109.764(2) | −5.586676693(6) |
| 0.5 | 0.2449779797(2) | −1.185759006(2) | 128.237(4) | −3.351429931(2) |
| 0.6 | −0.02485933989(8) | −1.3444771901(7) | 150.278(3) | −2.1579308505(8) |
| 0.7 | −0.20267459095(3) | −1.4242795783(3) | 176.191(4) | −1.4556148519(3) |
| 0.8 | −0.32453954069(3) | −1.4599779926(3) | 206.32(4) | −1.0136236390(3) |
| 0.9 | −0.41034091172(5) | −1.4700229433(4) | 241.20(6) | −0.7214901332(4) |
| 1.0 | −0.471869067616(3) | −1.464830657435(4) | 281.56(2) | −0.521092522208(3) |
| 1.1 | −0.516508388425(2) | −1.45055778977(4) | 327.854(8) | −0.379582739005(4) |
| 1.2 | −0.549086349362(4) | −1.43096895181(5) | 380.63(8) | −0.2773302108956(4) |
| 1.3 | −0.5728694058654(6) | −1.4084242331(3) | 441.41(9) | −0.20206570866(8) |
| 1.4 | −0.590131068915(4) | −1.38442943285(3) | 510.99(10) | −0.14583378217(2) |
| 1.5 | −0.602491470290(2) | −1.35995585486(3) | 590.55(9) | −0.10312564866(2) |
| 1.6 | −0.611128382454(2) | −1.33563273274(2) | 682.1(2) | −0.07085997995(5) |
| 1.7 | −0.6169127315137(10) | −1.3118664196(4) | 786.4(2) | −0.0459064450(2) |
| 1.8 | −0.6204981010747(10) | −1.28891604523(7) | 906.3(2) | −0.02662213504(3) |
| 1.9 | −0.622381305268(2) | −1.26694256387(3) | 1044.2(2) | −0.01167365972(8) |
| 2.0 | −0.6229442655573(9) | −1.24604113505(4) | 1203.323(5) | −0.00007630199(4) |
| 2.1 | −0.622483513172(4) | −1.226262869473(9) | 1386.517(5) | 0.00890674135(2) |
| 2.2 | −0.621231326927(2) | −1.20762967126(8) | 1598.535(6) | 0.01583317391(3) |
| 2.3 | −0.6193711108282(9) | −1.19014455791(8) | 1844.669(7) | 0.02112941902(3) |
| 2.4 | −0.617048739210(3) | −1.173799014243(3) | 2130.7(2) | 0.025124360064(6) |
| 2.5 | −0.614381038582(2) | −1.158578427009(10) | 2465.9(2) | 0.0280734600628(2) |
| 2.6 | −0.6114622119373(7) | −1.144466336618(7) | 2859.1(2) | 0.0301761874070(7) |
| 2.7 | −0.608368770770(2) | −1.131448052442(4) | 3322.1(2) | 0.031588699659(5) |
| 2.8 | −0.605163378709(2) | −1.11951405305(3) | 3869.71(6) | 0.032433108703(7) |
| 2.9 | −0.6018979001210(10) | −1.1086634889(3) | 4516.51(6) | 0.03280424531(8) |
| 3.0 | −0.598615868329(2) | −1.09890792783(9) | 5280.95(7) | 0.03277460295(2) |
| 3.1 | −0.595354525705(5) | −1.09027506387(7) | 6179.65(7) | 0.03239806050(2) |
| 3.2 | −0.592146522881(2) | −1.0828110341(2) | 7222.23(8) | 0.03171312866(4) |
| 3.3 | −0.589021268989(5) | −1.0765775859(2) | 8398.68(9) | 0.03074695518(3) |
| 3.4 | −0.586005756797(6) | −1.0716357388(2) | 9655.83(5) | 0.02952228671(4) |
| 3.5 | −0.583124412319(9) | −1.0680018191(2) | 10861.73(5) | 0.02807057301(5) |
| 3.6 | −0.580397232006(7) | −1.0655638231(3) | 11768.27(5) | 0.02645295581(6) |
| 3.7 | −0.577835676195(8) | −1.0639798481(7) | 12021.46(5) | 0.0247814876(2) |
| 3.8 | −0.575437429020(10) | −1.0626576394(4) | 11276.31(4) | 0.02321505754(9) |
| 3.9 | −0.57318403156(2) | −1.0609406401(5) | 9416.42(4) | 0.0219044674(2) |
| 4.0 | −0.57104574559(2) | −1.0584379155(5) | 6685.47(6) | 0.0209133939(2) |
| 4.1 | −0.56899231280(3) | −1.0552002953(2) | 3571.24(6) | 0.02019130007(3) |
| 4.2 | −0.56700237369(3) | −1.05158882920(10) | 544.93(7) | 0.019622837660(10) |
| 4.3 | −0.56506641508(4) | −1.04802146416(6) | −2105.93(9) | 0.0190956665120(6) |
| 4.4 | −0.56318441172(4) | −1.04481640217(9) | −4283.1(2) | 0.018534641200(2) |
| 4.5 | −0.56136190667(3) | −1.0421657312(4) | −6006.3(2) | 0.01790179603(5) |
| 4.6 | −0.55960694093(5) | −1.0401739306071(2) | −7345.3(2) | 0.01718259806(2) |
| 4.7 | −0.55792843247(5) | −1.03890851432(4) | −8374.8(2) | 0.01637198946(3) |
| 4.8 | −0.55633578677(3) | −1.03844559970(9) | −9156.6(3) | 0.01546374453(3) |
| 4.9 | −0.55483945143(3) | −1.0389138705(2) | −9726.9(3) | 0.01444184331(4) |
| 5.0 | −0.55345233874(2) | −1.0405481181(2) | −10084.7(3) | 0.01327131183(5) |

| $3^1\Pi_g$ continued | | | | |
|---|---|---|---|---|
| $R$ | $E$ | $\langle V\rangle$ | $10^6\cdot\langle\nabla_1\cdot\nabla_2\rangle$ | $\mathrm{d}E/\mathrm{d}R$ |
| 5.1 | −0.55219227845(3) | −1.0437625960(2) | −10173.8(3) | 0.01188665898(4) |
| 5.2 | −0.55108565805(3) | −1.0492289213(2) | −9837.3(3) | 0.01018122975(5) |
| 5.3 | −0.55017123941(3) | −1.0578282696(3) | −8781.2(4) | 0.00802154889(5) |
| 5.4 | −0.54949862426(2) | −1.0700841180(3) | −6630.6(3) | 0.00535428342(6) |
| 5.5 | −0.549109438920(3) | −1.08485964803(7) | −3289.71(3) | 0.00242895087(2) |
| 5.6 | −0.54900229322(2) | −1.0990459328(3) | 645.1(3) | −0.00018595471(5) |
| 5.7 | −0.54912139941(3) | −1.1099878047(4) | 4279.7(4) | −0.00206052737(8) |
| 5.8 | −0.54938911234(2) | −1.1172411649(3) | 7144.2(4) | −0.00318326557(6) |
| 5.9 | −0.549739795756(6) | −1.12164884109(8) | 9234.7(2) | −0.00375749993(2) |
| 6.0 | −0.5501291224359(10) | −1.124166740522(6) | 10720.923(3) | −0.003984749276(2) |
| 6.5 | −0.5520136062840(6) | −1.125516912204(6) | 13728.055(2) | −0.0033061076362(5) |
| 7.0 | −0.5533892069461(5) | −1.12237879354(3) | 14251.9880(8) | −0.002228625664(3) |
| 7.5 | −0.5542897570472(5) | −1.11925454096(3) | 14183.0897(8) | −0.001423336915(3) |
| 8.0 | −0.5548573111015(5) | −1.11679772493(2) | 13929.2339(3) | −0.000885387841(2) |
| 8.5 | −0.5552072992737(5) | −1.11501171213(2) | 13619.9237(3) | −0.000540836892(2) |
| 9.0 | −0.5554194618762(5) | −1.11376219641(2) | 13334.6989(3) | −0.0003248080731(10) |
| 9.5 | −0.5555456677359(5) | −1.112902635467(10) | 13165.5585(5) | −0.0001906631574(8) |
| 10.0 | −0.5556185277375(6) | −1.112310089186(10) | 13246.8167(3) | −0.0001073033711(7) |
| 11.0 | −0.5556761340818(5) | −1.1115664330174(3) | 15263.8056(5) | −0.0000194695325(2) |
| 12.0 | −0.55566779836772(4) | −1.110989841507(8) | 15241.9217(2) | 0.0000288129357(7) |
| 13.0 | −0.55563898013907(5) | −1.110943467126(2) | 11306.9422(5) | 0.0000257302424(2) |
| 14.0 | −0.55561711224048(3) | −1.1109776556118(4) | 10138.68679(6) | 0.00001832634780(2) |
| 15.0 | −0.55560160761690(2) | −1.1110080152956(3) | 9440.55024(6) | 0.000013013329216(10) |
| 16.0 | −0.55559052656376(2) | −1.1110309804546(3) | 8760.0752(2) | 0.000009379542059(8) |
| 17.0 | −0.555582469094821(7) | −1.11104781378529(7) | 7979.4009(2) | 0.000006889670846(2) |
| 18.0 | −0.555576494523461(6) | −1.11106007054241(7) | 7059.2862(2) | 0.000005162139140(2) |
| 19.0 | −0.555571976395343(8) | −1.11106904197475(6) | 5997.8480(2) | 0.0000039426745240(6) |
| 20.0 | −0.555568496600803(8) | −1.111075738449278(6) | 4833.4858(2) | 0.000003062737613(3) |

TABLE S4. Calculated BO energies, expectation value of potential, $\langle \nabla_1 \cdot \nabla_2 \rangle$, and $\mathrm{d}E/\mathrm{d}R$ of the $4^1\Pi_g$ state in atomic units (hartree). Uncertainties originate purely from extrapolation to the complete basis set limit. United atom values at $R = 0$ are taken from Ref. [1].

| $4^1\Pi_\mathrm{g}$ | | | | |
|---|---|---|---|---|
| $R$ | $E$ | $\langle V \rangle$ | $10^6 \cdot \langle \nabla_1 \cdot \nabla_2 \rangle$ | $\mathrm{d}E/\mathrm{d}R$ |
| 0.0 | −2.02000071089858471(1) | − | 1.4044136 | − |
| 0.01 | 97.980260650989(7) | 95.96103875451(2) | 1.4(2) | −9999.9482547467(3) |
| 0.05 | 17.986022651915(9) | 15.98347647195(3) | 1.5(3) | −399.7713766376(2) |
| 0.1 | 8.00175710873(2) | 6.04261658202(4) | 1.5(3) | −99.6089763544(2) |
| 0.15 | 4.690944156554(10) | 2.79059507758(4) | 1.4(4) | −43.94195490354(8) |
| 0.2 | 3.051378563840(9) | 1.21799813423(3) | 1.6(3) | −24.42379496724(5) |
| 0.3 | 1.44662761337(2) | −0.24541146531(4) | 1.6(6) | −10.46222230686(4) |
| 0.4 | 0.67924360789(2) | −0.87616448791(5) | 2.05(7) | −5.58662925921(4) |
| 0.5 | 0.24500879223(2) | −1.18566877746(5) | 2.62(6) | −3.35137272383(5) |
| 0.6 | −0.02482231207(2) | −1.34436284750(7) | 3.34(8) | −2.15786370561(5) |
| 0.7 | −0.20263033837(3) | −1.42413687960(9) | 4.16(9) | −1.45553743264(5) |
| 0.8 | −0.32448701317(3) | −1.45980240139(2) | 5.13(10) | −1.01353546882(6) |
| 0.9 | −0.41027900492(3) | −1.4698095530(2) | 6.3(2) | −0.72139060371(7) |
| 1.0 | −0.471796609452(7) | −1.46457410659(3) | 8.22(10) | −0.52098088769(2) |
| 1.1 | −0.516424124807(7) | −1.4502521608(4) | 9.8(2) | −0.3794581010(2) |
| 1.2 | −0.548988927859(2) | −1.43060765139(5) | 11.60(8) | −0.27719149640(2) |
| 1.3 | −0.5727573568182(2) | −1.40799984609(2) | 13.55(9) | −0.201911640352(4) |
| 1.4 | −0.5900027831365(3) | −1.383933541993(9) | 15.86(6) | −0.145662839797(2) |
| 1.5 | −0.6023451724546(3) | −1.3593788177149(4) | 18.2(2) | −0.1031256485379(7) |
| 1.6 | −0.61096209914(3) | −1.3349634047(3) | 20.9(2) | −0.0706495040(2) |
| 1.7 | −0.616724252240(5) | −1.311091804780(2) | 24.02(8) | −0.045672529599(7) |
| 1.8 | −0.620284930999(6) | −1.288020859716(3) | 27.34(8) | −0.026361665410(8) |
| 1.9 | −0.622140606844(7) | −1.265908673843(2) | 31.01(9) | −0.011382873779(8) |
| 2.0 | −0.62267278638(4) | −1.2448468421(5) | 34.9(2) | 0.0002493657(3) |
| 2.1 | −0.622177495806(2) | −1.224881980857(8) | 39.4(2) | 0.00927286224(2) |
| 2.2 | −0.6208863958439(4) | −1.206030292772(2) | 44.3(2) | 0.016246590410(6) |
| 2.3 | −0.618982128697(4) | −1.18828749956(7) | 49.6(2) | 0.02159859034(4) |
| 2.4 | −0.616609623343(3) | −1.17163567435(3) | 55.7(2) | 0.02565982179(3) |
| 2.5 | −0.613884524203(2) | −1.156047958225(8) | 62.2(2) | 0.02868843603(4) |
| 2.6 | −0.6108995443303(8) | −1.14149182228(2) | 69.4(2) | 0.03088741014(2) |
| 2.7 | −0.6077293020380(2) | −1.12793132212(5) | 77.3(2) | 0.032417511843(7) |
| 2.8 | −0.604434036573(5) | −1.11532864823(6) | 85.7(3) | 0.03340693744(4) |
| 2.9 | −0.6010624864(2) | −1.1036451813(9) | 95.2(3) | 0.0339585487(2) |
| 3.0 | −0.59765413634(2) | −1.09284220365(2) | 105.7(3) | 0.03415535626(6) |
| 3.1 | −0.594240983190(2) | −1.08288135807(3) | 117.3(3) | 0.03406471235(2) |
| 3.2 | −0.59084893391686(7) | −1.07372494609(3) | 130.6(2) | 0.033741538049(3) |
| 3.3 | −0.5874989179321(2) | −1.065336099839(7) | 144.80(4) | 0.033230829097(3) |
| 3.4 | −0.58420777795027(7) | −1.057678877310(8) | 160.3(5) | 0.032569611350(3) |
| 3.5 | −0.5809889871133(3) | −1.05071830470(3) | 177.54(6) | 0.031788477005(9) |
| 3.6 | −0.57785322934(2) | −1.0444203876(2) | 196.0(4) | 0.03091279748(7) |
| 3.7 | −0.5748088714682(2) | −1.038752104694(9) | 215.3(7) | 0.029963686006(8) |
| 3.8 | −0.57186234936291(9) | −1.03368140265(2) | 241.2(2) | 0.028958762119(10) |
| 3.9 | −0.5690184855323(2) | −1.02917719091(2) | 264.8(7) | 0.027912764142(5) |
| 4.0 | −0.56628075196476(2) | −1.025209356998(7) | 293.8(7) | 0.026838036733(2) |
| 4.1 | −0.56365148927456(8) | −1.0217488049730(5) | 325.5(9) | 0.02574492038443(7) |
| 4.2 | −0.56113209109228(8) | −1.0187675319700(6) | 361.8(9) | 0.02464205957489(9) |
| 4.3 | −0.55872316119001(9) | −1.0162387647427(7) | 402.7(9) | 0.0235366413110(2) |
| 4.4 | −0.556424650038(6) | −1.01413720247(4) | 450.1(8) | 0.02243456763(2) |
| 4.5 | −0.554235977807(2) | −1.01243948274(8) | 502.2(8) | 0.02134054952(3) |
| 4.6 | −0.552156154074(6) | −1.01112522422(4) | 561.4(8) | 0.02025806172(2) |
| 4.7 | −0.550183917496(6) | −1.01017995229(4) | 629.1(8) | 0.01918891121(2) |
| 4.8 | −0.548317979036(3) | −1.00960630645(3) | 707.9(10) | 0.018131177420(6) |
| 4.9 | −0.546557843250(3) | −1.00949288207(2) | 800.4(4) | 0.017065878454(5) |
| 5.0 | −0.544911255182(2) | −1.0111610506(4) | 887.16(10) | 0.01573229196(7) |

| $4^1\Pi_g$ continued | | | | |
|---|---|---|---|---|
| $R$ | $E$ | $\langle V\rangle$ | $10^6\cdot\langle\nabla_1\cdot\nabla_2\rangle$ | $\mathrm{d}E/\mathrm{d}R$ |
| 5.1 | −0.54368573246(2) | −1.0505036661(6) | 1256.9(5) | 0.0072289802(2) |
| 5.2 | −0.54320192046(3) | −1.0711463916(5) | 6022.92(3) | 0.00293412486(8) |
| 5.3 | −0.54302548727(3) | −1.0809108440(6) | 9837.26(4) | 0.00096983594(9) |
| 5.4 | −0.54293789782(3) | −1.0800525367(6) | 11085.7(6) | 0.00107838128(9) |
| 5.5 | −0.542766419283(7) | −1.07188955364(7) | 9884.59(8) | 0.002480597259(9) |
| 5.6 | −0.54243292422(3) | −1.0615650799(5) | 7274.92(7) | 0.00416085152(7) |
| 5.7 | −0.54194866213(3) | −1.0529511718(5) | 4476.5(2) | 0.00542914955(7) |
| 5.8 | −0.54136619133(3) | −1.0471591648(4) | 2156.4(3) | 0.00613331342(6) |
| 5.9 | −0.54073659844(3) | −1.0437145544(4) | 434.0(3) | 0.00639976992(5) |
| 6.0 | −0.540095497165(4) | −1.04187066192(3) | −790.24(7) | 0.006386722063(9) |
| 6.5 | −0.537224683459(4) | −1.04246461933(3) | −3027.69(7) | 0.004920730393(8) |
| 7.0 | −0.535182222692(4) | −1.04720328031(4) | −2822.00(6) | 0.003308737863(8) |
| 7.5 | −0.533842859154(3) | −1.05176374318(5) | −1960.12(6) | 0.002122930013(8) |
| 8.0 | −0.532992118107(3) | −1.05527884624(5) | −1043.45(5) | 0.001338173744(8) |
| 8.5 | −0.532456202578(2) | −1.05773142774(5) | −340.98(4) | 0.000844820870(7) |
| 9.0 | −0.532115776310(2) | −1.05935690349(5) | 57.43(3) | 0.000541627680(6) |
| 9.5 | −0.5318951269451(9) | −1.06040827828(4) | 171.35(3) | 0.000355997431(4) |
| 10.0 | −0.5317480709094(8) | −1.06108402680(2) | 83.89(2) | 0.000241211502(3) |
| 11.0 | −0.531575216531(2) | −1.061814827689(7) | −295.21(2) | 0.0001214186704(2) |
| 12.0 | −0.531484073029(2) | −1.06215995175(3) | −575.80(2) | 0.000067349526(2) |
| 13.0 | −0.531431848942(2) | −1.06234369567(3) | −718.50(2) | 0.000040000171(2) |
| 14.0 | −0.531399894176(3) | −1.06244397330(3) | −766.94(2) | 0.000025415361(2) |
| 15.0 | −0.531378768891(3) | −1.06249264579(3) | −727.43(2) | 0.000017659466(2) |
| 16.0 | −0.531363355767(3) | −1.06250903107(3) | −621.98(2) | 0.0000136050293(9) |
| 17.0 | −0.531350924558(2) | −1.06250670422(2) | −480.84(2) | 0.0000114791118(7) |
| 18.0 | −0.531340086370(2) | −1.06249475025(2) | −326.31(2) | 0.0000103012497(5) |
| 19.0 | −0.531330184557(2) | −1.06247903310(2) | −171.79(2) | 0.0000095440008(4) |
| 20.0 | −0.531320951017(2) | −1.062463234414(10) | −24.71(2) | 0.0000089333810(2) |

TABLE S5. Calculated BO energies, expectation value of potential, $\langle\nabla_1 \cdot \nabla_2\rangle$, and $\mathrm{d}E/\mathrm{d}R$ of the $1^3\Pi_g$ state in atomic units (hartree). Uncertainties originate purely from extrapolation to the complete basis set limit. United atom values at $R = 0$ are taken from Ref. [1].

| $1^3\Pi_g$ | | | | |
|---|---|---|---|---|
| $R$ | $E$ | $\langle V\rangle$ | $10^6 \cdot \langle\nabla_1 \cdot \nabla_2\rangle$ | $\mathrm{d}E/\mathrm{d}R$ |
| 0.0 | −2.055620732852246(6) | – | −25.322839(1) | – |
| 0.01 | 97.94462500300(2) | 95.8897673608(2) | −25.347(6) | −9999.948264525(9) |
| 0.05 | 17.9503858791(3) | 15.912200652(2) | −25.6986(4) | −399.77142213(3) |
| 0.1 | 7.96612707339(9) | 5.971328111(2) | −26.676(5) | −99.609060363(10) |
| 0.15 | 4.6552990567(4) | 2.719287184(2) | −28.083(5) | −43.942072865(8) |
| 0.2 | 3.015736780386(7) | 1.1466647710(3) | −29.847(5) | −24.4239439487(8) |
| 0.3 | 1.410958041133(9) | −0.31681240027(5) | −34.267(9) | −10.46242827513(10) |
| 0.4 | 0.643550737713(5) | −0.947654097237(9) | −39.751(3) | −5.5869389314(3) |
| 0.5 | 0.2092873205590(5) | −1.25726786806(3) | −46.369(3) | −3.35172501810(4) |
| 0.6 | −0.06057764443435(3) | −1.4160925136660(3) | −54.230(3) | −2.1582287079955(3) |
| 0.7 | −0.238424837235351(3) | −1.4960188312820(2) | −63.515(3) | −1.455984509733(2) |
| 0.8 | −0.360326089847806(4) | −1.5318591958253(6) | −74.452(3) | −1.0140337701622(4) |
| 0.9 | −0.4461682204850169(8) | −1.542064796361(2) | −87.318(2) | −0.7219426171005(7) |
| 1.0 | −0.5077417129942512(10) | −1.537052655548(2) | −102.438(2) | −0.5215892295590(10) |
| 1.1 | −0.5524310896822232(8) | −1.522980343681(2) | −120.195(2) | −0.3801256039240(4) |
| 1.2 | −0.585063989615279(7) | −1.5036135204861(5) | −141.042(2) | −0.2779212843796(2) |
| 1.3 | −0.608907054468511(2) | −1.48131347386(7) | −165.57(6) | −0.20270720375(3) |
| 1.4 | −0.626234005739364(2) | −1.45758737555(2) | −194.31(6) | −0.146528117186(6) |
| 1.5 | −0.638665212798672(2) | −1.433408106498(3) | −228.0418(9) | −0.1040651206001(10) |
| 1.6 | −0.647378716476691(2) | −1.409406718892(2) | −267.7908(10) | −0.0716683037118(8) |
| 1.7 | −0.653245746384718(2) | −1.385991670694(3) | −314.6310(9) | −0.046776575250(2) |
| 1.8 | −0.656920230372685(2) | −1.363424536754(3) | −369.9339(9) | −0.027557820005(2) |
| 1.9 | −0.658899373938490(3) | −1.341869116725(3) | −435.3778(10) | −0.0126791414987(10) |
| 2.0 | −0.659565544600868(3) | −1.321423891691(4) | −513.0275(8) | −0.001156401245(2) |
| 2.1 | −0.659215783031648(3) | −1.302143850859(4) | −605.4372(8) | 0.007746531050(2) |
| 2.2 | −0.658082950784804(3) | −1.284055425623(4) | −715.7780(9) | 0.014586579976(2) |
| 2.3 | −0.656351118823734(4) | −1.267166907248(4) | −848.0092(9) | 0.019789274087(2) |
| 2.4 | −0.654166924488570(4) | −1.251475896218(5) | −1007.0977(10) | 0.023682480316(2) |
| 2.5 | −0.651648065471791(4) | −1.236974819644(5) | −1199.306(2) | 0.026520524520(2) |
| 2.6 | −0.648889735599453(5) | −1.223655234290(5) | −1432.570(2) | 0.028501629580(2) |
| 2.7 | −0.645969566320446(5) | −1.211511434369(5) | −1716.998(2) | 0.029780628990(2) |
| 2.8 | −0.642951475809495(5) | −1.200543760788(6) | −2065.5268(9) | 0.030478282440(2) |
| 2.9 | −0.639888717148283(5) | −1.190761932048(6) | −2494.7824(9) | 0.030688104224(2) |
| 3.0 | −0.636826340677847(5) | −1.182188660866(6) | −3026.2001(9) | 0.030481340163(2) |
| 3.1 | −0.633803231604719(5) | −1.174863753226(6) | −3687.4565(9) | 0.029910551608(2) |
| 3.2 | −0.630853843666905(6) | −1.168848756461(6) | −4514.2367(8) | 0.029012165898(2) |
| 3.3 | −0.628009715485452(5) | −1.164231936802(6) | −5552.2761(8) | 0.0278083315665(10) |
| 3.4 | −0.625300819501107(5) | −1.161132760547(8) | −6859.4165(9) | 0.026308493663(2) |
| 3.5 | −0.622756742501709(5) | −1.159703871803(8) | −8506.9953(8) | 0.024511318057(2) |
| 3.6 | −0.620407616136948(4) | −1.160126516766(7) | −10579.1322(8) | 0.022407976530(2) |
| 3.7 | −0.618284589996605(4) | −1.162592469710(6) | −13167.3473(7) | 0.0199883000767(10) |
| 3.8 | −0.6164194715688430(5) | −1.1672630132324(3) | −16356.8482(2) | 0.0172515605012(3) |
| 3.9 | −0.6148430127018683(3) | −1.1741975019997(5) | −20201.21857(9) | 0.0142226983086(3) |
| 4.0 | −0.6135813920642892(2) | −1.1832578210603(2) | −24686.92266(6) | 0.01097624076700(8) |
| 4.1 | −0.61264102319971(2) | −1.19402450549040(5) | −29699.8796058(8) | 0.00762379046560(3) |
| 4.2 | −0.61204300455725(2) | −1.205788604580563(8) | −35017.685123(2) | 0.004356524889018(9) |
| 4.3 | −0.61175967360714(2) | −1.21766771029289(8) | −40346.995929(2) | 0.00136084579567(2) |
| 4.4 | −0.61175550977433(2) | −1.2288150325516(3) | −45397.230859(2) | −0.00120545750057(4) |
| 4.5 | −0.6119925392460975(2) | −1.238612312751(2) | −49951.73927(3) | −0.0032549409463(2) |
| 4.6 | −0.612387969721989(5) | −1.246751130078(2) | −53900.338960(10) | −0.0047772153551(4) |
| 4.7 | −0.612921095686271(6) | −1.253196032447(3) | −57228.8354510(10) | −0.0058199661861(5) |
| 4.8 | −0.613537719915784(4) | −1.258089013289(2) | −59986.173653(5) | −0.0064611611369(4) |
| 4.9 | −0.6142019566093(2) | −1.261655155612(3) | −62251.048607(9) | −0.0067859678354(4) |
| 5.0 | −0.6148961836067952(3) | −1.264137041445(3) | −64108.43754(2) | −0.0068729348463(5) |

| $1^3\Pi_g$ continued | | | | |
|---|---|---|---|---|
| $R$ | $E$ | $\langle V\rangle$ | $10^6\cdot\langle\nabla_1\cdot\nabla_2\rangle$ | $\mathrm{d}E/\mathrm{d}R$ |
| 5.1 | −0.615570031381760(6) | −1.265759260899(3) | −65636.86120(2) | −0.0067880780657(5) |
| 5.2 | −0.61623904916449(3) | −1.266714068969(4) | −66903.26601(2) | −0.0065838405077(5) |
| 5.3 | −0.616883401355604(9) | −1.267158926281(4) | −67962.20188(2) | −0.0063004006735(6) |
| 5.4 | −0.617496744203276(9) | −1.267219536365(4) | −68856.97913(2) | −0.0059677866589(6) |
| 5.5 | −0.6180853196896611(4) | −1.266994774604(4) | −69621.493243(10) | −0.0056080245862(6) |
| 5.6 | −0.61861725175936(8) | −1.2665617579874(8) | −70282.0815747(3) | −0.0052370097265(2) |
| 5.7 | −0.61912201191664(8) | −1.2659803415671(8) | −70859.1559792(3) | −0.0048660206551(2) |
| 5.8 | −0.61959001904326(8) | −1.2652968411745(8) | −71368.5422729(2) | −0.0045028970841(2) |
| 5.9 | −0.62002234241467(9) | −1.2645470073349(8) | −71822.5397140(2) | −0.00415293601788(10) |
| 6.0 | −0.6204304827255747(5) | −1.263758359(3) | −72230.89(8) | −0.0038162323(5) |
| 6.5 | −0.62197421146385(3) | −1.2598165566(10) | −73799.2527(5) | −0.0024412514(2) |
| 7.0 | −0.62294868122491(2) | −1.2565668374(5) | −74882.642(2) | −0.00152421072(8) |
| 7.5 | −0.62355517660007(2) | −1.2542213627(3) | −75675.0084(5) | −0.00094813461(5) |
| 8.0 | −0.623934198222452(9) | −1.2526481546(2) | −76263.5451(3) | −0.00059746978(3) |
| 8.5 | −0.624175920351951(6) | −1.251644951966(5) | −76700.1251(3) | −0.0003874248547(9) |
| 9.0 | −0.624335617890345(5) | −1.251029658832(4) | −77022.11251(2) | −0.0002620470059(7) |
| 9.5 | −0.624446191820649(10) | −1.250663874871(7) | −77258.445184(9) | −0.0001885780243(9) |
| 10.0 | −0.624526858556839(2) | −1.250451608377(3) | −77431.645411(5) | −0.0001397891264(4) |
| 11.0 | −0.6246382508422657(3) | −1.25026097210325(2) | −77653.0312283(2) | −0.000089497310795(3) |
| 12.0 | −0.62471380189591186(10) | −1.25019536682094(9) | −77776.64663864(4) | −0.000063980252425(5) |
| 13.0 | −0.624769358751530723(10) | −1.25016520828807(10) | −77849.6363596(2) | −0.000048191598845(6) |
| 14.0 | −0.6248117530815691 10(6) | −1.25014420717773(3) | −77895.65769984(6) | −0.000037192929615(3) |
| 15.0 | −0.624844707349533346(4) | −1.250126062678238(3) | −77926.55327888(9) | −0.0000291098652784(5) |
| 16.0 | −0.624870637584202693(2) | −1.250109782346086(2) | −77948.41483907(9) | −0.0000230316986052(3) |
| 17.0 | −0.6248912526172034632(10) | −1.250095383081320(2) | −77964.53144884(7) | −0.0000184045792303(3) |
| 18.0 | −0.624907802583200445(2) | −1.250082877226923(8) | −77976.7884072(6) | −0.000014848447808(2) |
| 19.0 | −0.6249212147302255493(4) | −1.2500721469967913(3) | −77986.33463603(5) | −0.0000120903966496(2) |
| 20.0 | −0.6249321825437318401(2) | −1.2500629969621513(6) | −77993.91014723(6) | −0.00000993159373442(6) |

TABLE S6. Calculated BO energies, expectation value of potential, $\langle\nabla_1 \cdot \nabla_2\rangle$, and $\mathrm{d}E/\mathrm{d}R$ of the $2^3\Pi_g$ state in atomic units (hartree). Uncertainties originate purely from extrapolation to the complete basis set limit. United atom values at $R = 0$ are taken from Ref. [1].

| $2^3\Pi_\mathrm{g}$ | | | | |
|---|---|---|---|---|
| $R$ | $E$ | $\langle V\rangle$ | $10^6 \cdot \langle\nabla_1 \cdot \nabla_2\rangle$ | $\mathrm{d}E/\mathrm{d}R$ |
| 0.0 | −2.031279846178687(7) | – | −29.442651(2) | – |
| 0.01 | 97.96897249229(5) | 95.9384623939(3) | −29.58(4) | −9999.94825907(3) |
| 0.05 | 17.974733993(3) | 15.96089816(2) | −29.95(4) | −399.7713966(3) |
| 0.1 | 7.990466994(4) | 6.02003263(3) | −30.96(4) | −99.6090136(2) |
| 0.15 | 4.679651792(3) | 2.76800251(2) | −32.47(4) | −43.94200712(9) |
| 0.2 | 3.040083244(2) | 1.195394350(8) | −34.36(4) | −24.42386069(3) |
| 0.3 | 1.4353244743(5) | −0.268044819(3) | −39.341(5) | −10.462312558(7) |
| 0.4 | 0.6679302897(2) | −0.898836393(2) | −45.516(6) | −5.586742432(2) |
| 0.5 | 0.23368303745(7) | −1.2083880467(5) | −52.96(2) | −3.3515082433(7) |
| 0.6 | −0.036162732986(10) | −1.36713838656(7) | −61.75(2) | −2.15802153431(7) |
| 0.7 | −0.21398766828(2) | −1.44697783131(8) | −71.84(8) | −1.45571784965(7) |
| 0.8 | −0.335863533943(8) | −1.48271824072(4) | −83.53(5) | −1.01373896604(3) |
| 0.9 | −0.42167705612(4) | −1.4928101672(2) | −97.53(7) | −0.72161783887(10) |
| 1.0 | −0.483218603955(4) | −1.48766987222(6) | −112.90(7) | −0.52123266430(2) |
| 1.1 | −0.527872562920(4) | −1.47345402934(2) | −130.82(5) | −0.379735366815(4) |
| 1.2 | −0.560466412202(2) | −1.453927246952(10) | −151.46(5) | −0.277495352111(4) |
| 1.3 | −0.584266608433(5) | −1.43144958156(2) | −175.09(5) | −0.202243357455(3) |
| 1.4 | −0.601546659844(5) | −1.40752676236(2) | −202.17(4) | −0.146023887623(6) |
| 1.5 | −0.613926690353(5) | −1.383129975964(8) | −233.25(5) | −0.1035177301723(5) |
| 1.6 | −0.622584458218(5) | −1.35888828103(2) | −268.93(4) | −0.071074602872(2) |
| 1.7 | −0.628390867321(5) | −1.33520778332(2) | −310.00(4) | −0.046132969810(3) |
| 1.8 | −0.631999469354(2) | −1.312347274881(10) | −357.37(4) | −0.026860186750(3) |
| 1.9 | −0.6339070344882(10) | −1.29046725435(2) | −412.18(4) | −0.011922729142(4) |
| 2.0 | −0.634495425267(6) | −1.26966227753(2) | −475.81(4) | −0.000335713500(4) |
| 2.1 | −0.6340610952283(10) | −1.24998265547(3) | −549.98(4) | 0.008637873804(5) |
| 2.2 | −0.6328362217667(9) | −1.23144923436(2) | −636.83(4) | 0.015556004171(2) |
| 2.3 | −0.631004077017(3) | −1.21406362994(2) | −739.05(4) | 0.020845445252(3) |
| 2.4 | −0.6287103641287(10) | −1.19781546324(2) | −860.05(5) | 0.024835527092(2) |
| 2.5 | −0.626071687315(2) | −1.18268763655(2) | −1004.14(4) | 0.0277822952317(7) |
| 2.6 | −0.623181960512(2) | −1.16866037939(4) | −1176.98(5) | 0.029885977557(8) |
| 2.7 | −0.620117319480(9) | −1.15571461300(5) | −1385.82(5) | 0.031303713318(10) |
| 2.8 | −0.616939941277(2) | −1.14383509553(3) | −1640.34(5) | 0.032158852512(2) |
| 2.9 | −0.613701067412(2) | −1.13301379787(3) | −1953.35(4) | 0.032547702403(2) |
| 3.0 | −0.610443454976(10) | −1.12325402413(6) | −2342.13(5) | 0.03254429527(2) |
| 3.1 | −0.6072034345004(8) | −1.11457593274(3) | −2830.23(5) | 0.0322035278307(8) |
| 3.2 | −0.6040127274893(4) | −1.10702433055(6) | −3450.05(5) | 0.031562851390(10) |
| 3.3 | −0.60090016421(5) | −1.1006798295(2) | −4246.34(9) | 0.03064257542(3) |
| 3.4 | −0.597893438122(2) | −1.0956743553(2) | −5280.6(2) | 0.02944485912(2) |
| 3.5 | −0.5950210111332(9) | −1.09221049207(5) | −6635.36(10) | 0.027951865773(7) |
| 3.6 | −0.5923141735452(10) | −1.09057810870(8) | −8415.19(9) | 0.026125066233(6) |
| 3.7 | −0.58980888806(5) | −1.0911438734(3) | −10731.78(10) | 0.02391186561(4) |
| 3.8 | −0.5875460383889(4) | −1.09425014963(7) | −13650.69(9) | 0.02127419135(2) |
| 3.9 | −0.585566812893(2) | −1.0999184816(2) | −17069.24(5) | 0.01826029340(3) |
| 4.0 | −0.58389875797(7) | −1.1073512504(9) | −20551.8(2) | 0.0151115664(2) |
| 4.1 | −0.582533615723(10) | −1.1146761090(3) | −23320.32(10) | 0.01229051766(5) |
| 4.2 | −0.58141345036(2) | −1.1196745366(3) | −24626.08(8) | 0.01027437242(6) |
| 4.3 | −0.58044545601(2) | −1.1211438305(3) | −24239.72(6) | 0.00924350733(6) |
| 4.4 | −0.579537736090(4) | −1.119396887738(10) | −22509.4(2) | 0.0090178601005(7) |
| 4.5 | −0.578626447785(2) | −1.11559560495(4) | −20018.1(2) | 0.00925717569(2) |
| 4.6 | −0.577681007509(4) | −1.11092911352(3) | −17273.2(2) | 0.009659326412(4) |
| 4.7 | −0.576695637475(4) | −1.10623517270(3) | −14597.80(10) | 0.010033213245(5) |
| 4.8 | −0.575678431733(2) | −1.101978327294(8) | −12153.1(2) | 0.0102871950359(10) |
| 4.9 | −0.574643151342(2) | −1.098357357808(9) | −9994.61(10) | 0.010393662220(2) |
| 5.0 | −0.5736044316392(6) | −1.09541587003(5) | −8121.37(4) | 0.010358598656(2) |

| $2^3\Pi_g$ continued | | | | |
|---|---|---|---|---|
| $R$ | $E$ | $\langle V\rangle$ | $10^6\cdot\langle\nabla_1\cdot\nabla_2\rangle$ | $\mathrm{d}E/\mathrm{d}R$ |
| 5.1 | −0.572575477973(2) | −1.093119471736(10) | −6507.09(8) | 0.010202251806(2) |
| 5.2 | −0.571567218809(2) | −1.091401019259(10) | −5116.86(8) | 0.009948734300(2) |
| 5.3 | −0.570588196543(2) | −1.090184287824(10) | −3916.27(7) | 0.009621151936(2) |
| 5.4 | −0.569644779897(2) | −1.08939511668(2) | −2874.52(7) | 0.009239711688(2) |
| 5.5 | −0.5687414837363(4) | −1.088965929463(6) | −1965.4156(7) | 0.0088212796383(7) |
| 5.6 | −0.567881296888(2) | −1.08883701003(2) | −1167.72(6) | 0.008379568525(2) |
| 5.7 | −0.567065977772(2) | −1.08895632656(2) | −463.71(6) | 0.007925548944(2) |
| 5.8 | −0.566296306044(2) | −1.08927880037(2) | 160.57(6) | 0.007467898573(2) |
| 5.9 | −0.565572290847(2) | −1.089765440700(2) | 716.38(6) | 0.007013413728(2) |
| 6.0 | −0.5648933409067(3) | −1.090382525557(5) | 1212.8604(2) | 0.0065673593761(5) |
| 6.5 | −0.5621272672658(3) | −1.094533119681(5) | 3016.4348(2) | 0.0045725253617(5) |
| 7.0 | −0.5602367585114(3) | −1.098954993884(4) | 4014.6310(4) | 0.0030740747342(4) |
| 7.5 | −0.5589750788789(3) | −1.102634972097(5) | 4448.0180(5) | 0.0020420247548(4) |
| 8.0 | −0.5581352901404(3) | −1.105336010159(5) | 4443.1333(7) | 0.0013668212652(5) |
| 8.5 | −0.5575673021790(3) | −1.107159388805(6) | 4076.9943(6) | 0.0009382606533(5) |
| 9.0 | −0.5571703362076(4) | −1.108304198224(6) | 3420.5415(6) | 0.0006707193546(5) |
| 9.5 | −0.5568799100018(3) | −1.108973060378(5) | 2568.2339(7) | 0.0005038694343(4) |
| 10.0 | −0.5566565205232(3) | −1.109341170137(5) | 1630.4671(7) | 0.0003971870909(4) |
| 11.0 | −0.5563284005582(3) | −1.109664801141(5) | −152.0813(5) | 0.0002719999978(3) |
| 12.0 | −0.5560970777438(3) | −1.109850331165(4) | −1552.6811(2) | 0.0001953186935(2) |
| 13.0 | −0.5559309645041(3) | −1.110047299406(3) | −2548.6089(2) | 0.0001395868925(2) |
| 14.0 | −0.5558132331397(4) | −1.110255059114(2) | −3220.975(2) | 0.00009795765466(6) |
| 15.0 | −0.5557313019435(3) | −1.1104489609929(8) | −3651.0238(2) | 0.00006757619293(3) |
| 16.0 | −0.5556751333245(2) | −1.1106135897104(10) | −3898.9277(2) | 0.00004604230867(3) |
| 17.0 | −0.5556370122850(2) | −1.1107447155183(9) | −4005.5948(2) | 0.00003113582657(2) |
| 18.0 | −0.55561128066310(9) | −1.1108447965701(4) | −3998.8046(2) | 0.000020986930896(4) |
| 19.0 | −0.55559393894908(7) | −1.1109190340775(3) | −3899.0180(3) | 0.0000141496747722(4) |
| 20.0 | −0.55558223232900(9) | −1.1109730671575(3) | −3723.7860(3) | 0.000009569875012(8) |

TABLE S7. Calculated BO energies, expectation value of potential, $\langle \nabla_1 \cdot \nabla_2 \rangle$, and $\mathrm{d}E/\mathrm{d}R$ of the $3^3\Pi_g$ state in atomic units (hartree). Uncertainties originate purely from extrapolation to the complete basis set limit. United atom values at $R = 0$ are taken from Ref. [1].

| $3^3\Pi_\mathrm{g}$ | | | | |
|---|---|---|---|---|
| $R$ | $E$ | $\langle V \rangle$ | $10^6 \cdot \langle \nabla_1 \cdot \nabla_2 \rangle$ | $\mathrm{d}E/\mathrm{d}R$ |
| 0.0 | −2.020015836159984(4) | – | −19.56885(1) | – |
| 0.01 | 97.980260651(4) | 95.96103869(4) | −20(4) | −9999.948255(3) |
| 0.05 | 17.986002072(4) | 15.98343482(3) | −20(2) | −399.7713865(5) |
| 0.1 | 8.001735794(5) | 6.04257208(4) | −20.5(5) | −99.6089950(3) |
| 0.15 | 4.690921725(9) | 2.79054636(4) | −22.2(3) | −43.9419806(2) |
| 0.2 | 3.051354635(3) | 1.21794370(2) | −23.2(3) | −24.42382784(7) |
| 0.3 | 1.4465997850(10) | −0.245480588(7) | −25.95(3) | −10.46226719(2) |
| 0.4 | 0.6792107298(4) | −0.876252655(3) | −30.01(4) | −5.586685287(5) |
| 0.5 | 0.2449697690(2) | −1.185780251(2) | −34.87(4) | −3.351439577(2) |
| 0.6 | −0.02486855955(7) | −1.3445019281(5) | −40.59(4) | −2.1579413483(7) |
| 0.7 | −0.20263033853(6) | −1.4241368802(3) | 4.39(10) | −1.4555374331(3) |
| 0.8 | −0.32455098042(3) | −1.4600101054(2) | −54.96(5) | −1.0136351807(2) |
| 0.9 | −0.410353513774(8) | −1.4700586337(2) | −63.80(6) | −0.7215017846(2) |
| 1.0 | −0.47188282573(2) | −1.46486957680(10) | −73.799(7) | −0.52110392535(7) |
| 1.1 | −0.516523256428(4) | −1.4505993106(2) | −85.340(6) | −0.3795934525(2) |
| 1.2 | −0.54910223210(3) | −1.4310120949(7) | −99.3(4) | −0.27733969195(3) |
| 1.3 | −0.57288614798(3) | −1.4084675779(5) | −114.9(7) | −0.202073296(2) |
| 1.4 | −0.59014844149(3) | −1.3844710060(10) | −132.4(9) | −0.145838659(2) |
| 1.5 | −0.602509154775(7) | −1.3599929961(2) | −150.5(2) | −0.10331645769(2) |
| 1.6 | −0.611145951413(5) | −1.33566193194(2) | −172.8(2) | −0.070856268284(8) |
| 1.7 | −0.6169296252958(7) | −1.31188310842(3) | −198.3(2) | −0.04589638701(5) |
| 1.8 | −0.62051359977(3) | −1.28891434255(3) | −227.6(2) | −0.02660396840(5) |
| 1.9 | −0.6223944944604(9) | −1.26691495310(4) | −261.4(2) | −0.01164524421(2) |
| 2.0 | −0.6229539945173(2) | −1.24597805894(7) | −300.134(8) | −0.00003503495(3) |
| 2.1 | −0.6224883432629(8) | −1.2261522122(2) | −345.459(8) | 0.00896403544(6) |
| 2.2 | −0.621229467652(4) | −1.207456092(2) | −398.351(8) | 0.0159103834(5) |
| 2.3 | −0.61936033985(6) | −1.189888630(2) | −460.433(8) | 0.0212313261(5) |
| 2.4 | −0.617026301867(2) | −1.17343610673(8) | −534.5(3) | 0.02525687375(3) |
| 2.5 | −0.614343520731(3) | −1.15807724838(9) | −621.9(3) | 0.02824391723(4) |
| 2.6 | −0.611405378735(2) | −1.14378704185(7) | −726.7(3) | 0.03039373677(3) |
| 2.7 | −0.6082873623758(4) | −1.1305398186(3) | −853.6(3) | 0.03186478007(9) |
| 2.8 | −0.605050853566(3) | −1.1183120624(2) | −1008.168(6) | 0.03278201599(4) |
| 2.9 | −0.601746119221(9) | −1.1070854301(2) | −1200.612(7) | 0.03324372701(4) |
| 3.0 | −0.598414725798(3) | −1.0968505922(2) | −1442.244(8) | 0.03332628648(4) |
| 3.1 | −0.595091564382(2) | −1.08761282686(8) | −1750.299(10) | 0.03308719416(3) |
| 3.2 | −0.591806657791(4) | −1.0794009100(2) | −2149.82(2) | 0.03256637675(4) |
| 3.3 | −0.5885869362907(6) | −1.0722819623(2) | −2677.85(2) | 0.03178542734(4) |
| 3.4 | −0.585458221540(4) | −1.06638669579(8) | −3389.80(9) | 0.03074404332(2) |
| 3.5 | −0.582447749429(4) | −1.06195117164(8) | −4367.19(3) | 0.02941266491(2) |
| 3.6 | −0.57958761710(2) | −1.0593766634(4) | −5723.83(7) | 0.02772182520(10) |
| 3.7 | −0.576919104957(5) | −1.0592697080(5) | −7582.34(5) | 0.0255590545(2) |
| 3.8 | −0.574495127752(4) | −1.0622605937(3) | −9948.09(5) | 0.02282359521(6) |
| 3.9 | −0.572369539222(8) | −1.0680827644(5) | −12362.49(6) | 0.0196554651(2) |
| 4.0 | −0.57055501751(2) | −1.0740251841(7) | −13626.20(8) | 0.0167712127(2) |
| 4.1 | −0.56897296524(3) | −1.0759441729(4) | −12670.7(7) | 0.01512237989(8) |
| 4.2 | −0.56748417402(6) | −1.0726675837(7) | −9907.2(2) | 0.0148335153(2) |
| 4.3 | −0.56598403102(4) | −1.0665364737(3) | −6639.6(2) | 0.01521664844(6) |
| 4.4 | −0.56444044335(7) | −1.0601283091(6) | −3760.6(3) | 0.01562558581(9) |
| 4.5 | −0.56286778313(3) | −1.0547427949(4) | −1527.7(3) | 0.01577617139(5) |
| 4.6 | −0.56129549183(6) | −1.050735469356(5) | 116.6(4) | 0.01562076394(3) |
| 4.7 | −0.55975257539(6) | −1.04807832298(6) | 1309.9(4) | 0.01519719736(4) |
| 4.8 | −0.55826333472(4) | −1.04666443702(9) | 2171.7(4) | 0.01455463173(4) |
| 4.9 | −0.55684774996(4) | −1.0464265137(2) | 2782.6(5) | 0.01372836450(4) |
| 5.0 | −0.55552324180(2) | −1.0473762498(2) | 3184.0(3) | 0.01273404670(6) |

| $3^3\Pi_g$ continued | | | | |
|---|---|---|---|---|
| $R$ | $E$ | $\langle V\rangle$ | $10^6\cdot\langle\nabla_1\cdot\nabla_2\rangle$ | $\mathrm{d}E/\mathrm{d}R$ |
| 5.1 | −0.55430664336(4) | −1.0496159443(2) | 3377.2(5) | 0.01156810633(5) |
| 5.2 | −0.55321596915(4) | −1.0533322512(2) | 3328.7(5) | 0.01021147827(5) |
| 5.3 | −0.55227153165(3) | −1.0587517540(3) | 2964.7(5) | 0.00863986966(6) |
| 5.4 | −0.55149542065(3) | −1.0660148397(3) | 2186.7(5) | 0.00684740768(6) |
| 5.5 | −0.550907811175(6) | −1.07494668362(2) | 916.66(2) | 0.004885261579(7) |
| 5.6 | −0.55051950127(3) | −1.0848470408(3) | −831.0(4) | 0.00289142173(6) |
| 5.7 | −0.55032397818(2) | −1.0945893051(3) | −2893.6(4) | 0.00106292127(5) |
| 5.8 | −0.55029573584(2) | −1.1031081937(3) | −5023.7(3) | −0.00043391761(5) |
| 5.9 | −0.55039743388(2) | −1.1098469381(2) | −7005.2(3) | −0.00153424922(4) |
| 6.0 | −0.5505903149951(10) | −1.11478798400(4) | −8722.89(2) | −0.002267892337(8) |
| 6.5 | −0.5520226931304(9) | −1.123041986567(10) | −13687.530(2) | −0.0029225538931(5) |
| 7.0 | −0.5533069724790(5) | −1.121814783512(5) | −15610.0224(10) | −0.0021715483647(3) |
| 7.5 | −0.5542013958060(5) | −1.119168153365(5) | −16500.8104(7) | −0.0014353815670(3) |
| 8.0 | −0.5547756733757(3) | −1.116708047518(2) | −16924.8499(7) | −0.00089458759575(6) |
| 8.5 | −0.5551256323114(3) | −1.1147661795338(8) | −17039.5989(5) | −0.00053116646017(4) |
| 9.0 | −0.5553289651888(2) | −1.113364025742446(3) | −16903.4812(4) | −0.00030067726291(9) |
| 9.5 | −0.55544159127004(10) | −1.1124237919690(4) | −16580.1317(3) | −0.00016216941367(10) |
| 10.0 | −0.55550099498568(7) | −1.1118333062833(4) | −16152.6728(2) | −0.00008313163125(7) |
| 11.0 | −0.55554449337938(3) | −1.11128329348558(3) | −15268.13578(9) | −0.00001766424792(2) |
| 12.0 | −0.55555197077828(2) | −1.1111193407869(2) | −14561.53445(4) | −0.000001283269190(3) |
| 13.0 | −0.555551319952593(10) | −1.1110820304889(2) | −14065.32844(4) | 0.000001585339715(4) |
| 14.0 | −0.555549771540706(8) | −1.1110809890510(2) | −13735.94614(4) | 0.000001325287891(6) |
| 15.0 | −0.555548790654518(6) | −1.1110879318886(2) | −13533.42264(6) | 0.000000643294695(5) |
| 16.0 | −0.555548427064753(7) | −1.1110949209489(2) | −13432.75693(2) | 0.000000120823788(7) |
| 17.0 | −0.555548479071485(8) | −1.1111002615034(2) | −13419.64225(7) | −0.000000194315322(7) |
| 18.0 | −0.555548765560403(7) | −1.1111039897134(2) | −13485.07562(5) | −0.000000358810701(5) |
| 19.0 | −0.555549165800166(6) | −1.11110650159334(7) | −13621.264652(3) | −0.000000429999631(2) |
| 20.0 | −0.555549608016373(6) | −1.11110817701461(8) | −13818.942931(10) | −0.000000448049093(3) |

TABLE S8. Calculated BO energies, expectation value of potential, $\langle \nabla_1 \cdot \nabla_2 \rangle$, and $\mathrm{d}E/\mathrm{d}R$ of the $4^3\Pi_g$ state in atomic units (hartree). Uncertainties originate purely from extrapolation to the complete basis set limit. United atom values at $R = 0$ are taken from Ref. [1].

| $4^3\Pi_\mathrm{g}$ | | | | |
|---|---|---|---|---|
| $R$ | $E$ | $\langle V \rangle$ | $10^6 \cdot \langle \nabla_1 \cdot \nabla_2 \rangle$ | $\mathrm{d}E/\mathrm{d}R$ |
| 0.0 | −2.02000071089858471(1) | – | 1.4040013 | – |
| 0.01 | 97.98026065107(3) | 95.9610387553(2) | 1.403(3) | −9999.948254680(8) |
| 0.05 | 17.9860226531(9) | 15.983476480(7) | 1.22(5) | −399.77137652(9) |
| 0.1 | 8.001757107(3) | 6.04261657(3) | 1.30(5) | −99.6089764(2) |
| 0.15 | 4.6909441566(4) | 2.790595078(3) | 1.38(6) | −43.94195490(2) |
| 0.2 | 3.05137856388(8) | 1.2179981347(7) | 1.55(3) | −24.423794965(3) |
| 0.3 | 1.44662761328(8) | −0.2454114657(7) | 1.93(4) | −10.462222308(2) |
| 0.4 | 0.6792436074(10) | −0.876164494(4) | 2.42(6) | −5.586629266(4) |
| 0.5 | 0.2450087920(3) | −1.185668779(3) | 3.04(7) | −3.351372725(3) |
| 0.6 | −0.0248223122(2) | −1.3443628483(10) | 3.79(7) | −2.157863706(2) |
| 0.7 | −0.20263033850(7) | −1.4241368802(4) | 4.68(7) | −1.4555374331(4) |
| 0.8 | −0.32448701335(3) | −1.4598024023(5) | 5.75(7) | −1.0135354694(5) |
| 0.9 | −0.41027900504(2) | −1.4698095539(3) | 6.95(7) | −0.7213906042(3) |
| 1.0 | −0.47179660964(3) | −1.4645741074(2) | 8.31(8) | −0.5209808881(2) |
| 1.1 | −0.51642412504(5) | −1.4502521619(7) | 9.81(10) | −0.3794581014(2) |
| 1.2 | −0.548988928116(7) | −1.43060765248(6) | 11.64(8) | −0.27719149692(2) |
| 1.3 | −0.572757357129(4) | −1.40799986(2) | 12.2(2) | −0.201911651(10) |
| 1.4 | −0.5900027835016(10) | −1.38393354355(3) | 14.3(2) | −0.145662840390(5) |
| 1.5 | −0.60234517289(3) | −1.3593788198(3) | 18.2(2) | −0.1031256493(2) |
| 1.6 | −0.61096209962(2) | −1.3349634068(3) | 20.9(2) | −0.0706495047(2) |
| 1.7 | −0.61672425280(2) | −1.3110918072(2) | 22.4(3) | −0.04567253034(4) |
| 1.8 | −0.62028493151(9) | −1.2880208618(6) | 25.6(3) | −0.0263616662(2) |
| 1.9 | −0.622140607553(5) | −1.2659086763(8) | 30.52(5) | −0.0113828746(3) |
| 2.0 | −0.622672787129(2) | −1.2448468447(3) | 34.9(2) | 0.00024936486(6) |
| 2.1 | −0.622177496641(7) | −1.224881983630(10) | 39.3(2) | 0.00927286169(4) |
| 2.2 | −0.620886396721(5) | −1.20603029524(2) | 44.2(2) | 0.01624659006(3) |
| 2.3 | −0.6189821295875(8) | −1.18828750130(9) | 49.6(2) | 0.021598590407(10) |
| 2.4 | −0.616609624211(3) | −1.17163567500(3) | 55.7(2) | 0.02565982224(3) |
| 2.5 | −0.613884524997(2) | −1.156047957185(4) | 62.2(2) | 0.02868843709(4) |
| 2.6 | −0.61089954498231(3) | −1.141491818822(4) | 69.3(2) | 0.0308874119783(7) |
| 2.7 | −0.607729302462(3) | −1.12793132(2) | 77.2(2) | 0.032417512(4) |
| 2.8 | −0.604434036660(3) | −1.115328643(7) | 85.7(3) | 0.033406940(2) |
| 2.9 | −0.601062486082(2) | −1.10364516529(4) | 95.6(2) | 0.03395855408(2) |
| 3.0 | −0.5976541353407(3) | −1.092842180552(9) | 105.7(3) | 0.034155363373(5) |
| 3.1 | −0.594240981408(2) | −1.08288132760(5) | 117.7(2) | 0.03406472103(3) |
| 3.2 | −0.5908489311837(2) | −1.073724907610(7) | 130.62(4) | 0.033741548360(3) |
| 3.3 | −0.5874989141010(2) | −1.065336054083(8) | 144.70(4) | 0.033230840641(4) |
| 3.4 | −0.584207772941(2) | −1.05767882736(3) | 161(5) | 0.03256962303(5) |
| 3.5 | −0.5809889809831(8) | −1.05071825695(5) | 176.4(5) | 0.03178848714(2) |
| 3.6 | −0.577853222423(10) | −1.0444203562(2) | 195.9(4) | 0.03091280236(7) |
| 3.7 | −0.5748088645768(2) | −1.03875211641(3) | 216.5(5) | 0.02996367911(2) |
| 3.8 | −0.57186234419821(8) | −1.033681506919(9) | 241.21(3) | 0.028958731967(3) |
| 3.9 | −0.5690184853498(2) | −1.02917747912(3) | 265.3(7) | 0.02791269014(2) |
| 4.0 | −0.5662807628308(5) | −1.02520999997(4) | 294.5(7) | 0.02683788142(2) |
| 4.1 | −0.563651522477(2) | −1.02175013198(2) | 326.3(9) | 0.025744612919(4) |
| 4.2 | −0.561132168078(2) | −1.01877021099(2) | 363.0(9) | 0.024641458372(4) |
| 4.3 | −0.558723324592(2) | −1.01624425782(2) | 404.4(9) | 0.023535439850(4) |
| 4.4 | −0.556424991325(2) | −1.01414909522(2) | 451.2(10) | 0.022432019869(4) |
| 4.5 | −0.5542367194623(6) | −1.01246826453(5) | 506.2(10) | 0.02133448319(3) |
| 4.6 | −0.552157969677(3) | −1.01121240352(2) | 574.0(10) | 0.020239899094(2) |
| 4.7 | −0.550190044063(4) | −1.0106378188(3) | 686.2(9) | 0.01909409986(5) |
| 4.8 | −0.54837960546(5) | −1.017610257(6) | 1392.26(7) | 0.016489365(2) |
| 4.9 | −0.54685717563(2) | −1.02378502053(6) | 846.7(5) | 0.014271291994(2) |
| 5.0 | −0.545520491245(7) | −1.0289855764(2) | 435.19(3) | 0.01241108119(4) |

$4^3\Pi_g$ continued

| $R$ | $E$ | $\langle V \rangle$ | $10^6 \cdot \langle \nabla_1 \cdot \nabla_2 \rangle$ | $\mathrm{d}E/\mathrm{d}R$ |
|---|---|---|---|---|
| 5.1 | −0.544388163498(8) | −1.03693940053(8) | −1039.98(5) | 0.01016410323(2) |
| 5.2 | −0.543499875982(9) | −1.0476614273(2) | −3279.21(7) | 0.00756506244(3) |
| 5.3 | −0.54287304482(2) | −1.0590340778(3) | −6009.89(9) | 0.00504000224(4) |
| 5.4 | −0.54246677276(2) | −1.0673568701(3) | −8456.4(2) | 0.00325493989(5) |
| 5.5 | −0.542185330424(5) | −1.07033736098(2) | −9900.58(7) | 0.0025515090648(9) |
| 5.6 | −0.54192653397(2) | −1.0685181911(3) | −10165.6(2) | 0.00273837086(4) |
| 5.7 | −0.54162260302(4) | −1.0639831237(3) | −9516.4(2) | 0.00337931268(3) |
| 5.8 | −0.54124859050(4) | −1.0587813124(2) | −8370.8(3) | 0.00408894286(2) |
| 5.9 | −0.54080986750(4) | −1.05417180394(8) | −7084.3(3) | 0.0046521916946(10) |
| 6.0 | −0.540325255086(7) | −1.05062065262(2) | −5867.44(10) | 0.005004976249(8) |
| 6.5 | −0.537801898946(7) | −1.04500542947(6) | −2098.31(10) | 0.00470744129(2) |
| 7.0 | −0.535754064289(6) | −1.04719492291(5) | −654.20(8) | 0.00347331509(2) |
| 7.5 | −0.534299142806(5) | −1.05065086308(4) | −46.79(9) | 0.002392989665(9) |
| 8.0 | −0.533312900075(6) | −1.05384794035(2) | 260.97(6) | 0.001597232469(5) |
| 8.5 | −0.532663314686(6) | −1.056566944634(3) | 589.56(8) | 0.001030551140(4) |
| 9.0 | −0.532275678755(6) | −1.06024179869(3) | 1947.0(2) | 0.000478839863(7) |
| 9.5 | −0.532172897818(8) | −1.06365363957(7) | 3129.6(2) | 0.000072858527(10) |
| 10.0 | −0.532138695503(4) | −1.063530098533(5) | 2861.22(6) | 0.000074729244(3) |
| 11.0 | −0.532048285349(3) | −1.062997143635(2) | 2405.53(5) | 0.000099947913(2) |
| 12.0 | −0.531948458311(2) | −1.062733482675(3) | 2089.68(3) | 0.0000969528277(9) |
| 13.0 | −0.531856907345(2) | −1.062597356958(4) | 1828.93(2) | 0.0000858813635(3) |
| 14.0 | −0.531776339041(2) | −1.062493684751(4) | 1578.87(2) | 0.0000756423803(3) |
| 15.0 | −0.531704840705(3) | −1.062394393909(9) | 1325.79(4) | 0.000067685832(2) |
| 16.0 | −0.531640485492(2) | −1.06230210568(2) | 1072.39(4) | 0.000061179080(2) |
| 17.0 | −0.531582305099(2) | −1.062225845513(10) | 826.26(3) | 0.000055221451(2) |
| 18.0 | −0.531530015278(2) | −1.062171584740(4) | 594.610(9) | 0.00004935810078(4) |
| 19.0 | −0.5314835893486(10) | −1.062140689325(4) | 382.36(2) | 0.0000434994402(5) |
| 20.0 | −0.5314429823395(10) | −1.062131071774(6) | 192.165(8) | 0.00003774464524(8) |

TABLE S9. Calculated BO energies, expectation value of potential, $\langle \nabla_1 \cdot \nabla_2 \rangle$, and $\mathrm{d}E/\mathrm{d}R$ of the $1^1\Pi_u$ state in atomic units (hartree). Uncertainties originate purely from extrapolation to the complete basis set limit. United atom values at $R = 0$ are taken from Ref. [1].

| $1^1\Pi_\mathrm{u}$ | | | | |
|---|---|---|---|---|
| $R$ | $E$ | $\langle V \rangle$ | $10^6 \cdot \langle \nabla_1 \cdot \nabla_2 \rangle$ | $\mathrm{d}E/\mathrm{d}R$ |
| 0.0 | −2.123843086498093(2) | – | −46044.524937(1) | – |
| 0.01 | 97.87641882002(3) | 95.7533561775(2) | −46051.813(3) | −9999.94814625(2) |
| 0.05 | 17.878(3) | 15.775843794(3) | −46211.3428(4) | −399.77086138(3) |
| 0.1 | 7.89797526705(6) | 5.835130023(6) | −46644.3052(5) | −99.60820512(4) |
| 0.15 | 4.58721127140(5) | 2.5833363154(4) | −47262.6289(3) | −43.940574849(2) |
| 0.2 | 2.94772409428(2) | 1.0110393618(2) | −48007.6518346(10) | −24.4220441337(4) |
| 0.3 | 1.3431916946396(7) | −0.45158265945(2) | −49719.15865(3) | −10.45982016243(5) |
| 0.4 | 0.5760763831697(2) | −1.081335952969(6) | −51558.11223(2) | −5.583671798272(10) |
| 0.5 | 0.1421617432877(2) | −1.389665929514(9) | −53404.707(5) | −3.34793883218(2) |
| 0.6 | −0.12730504535678(7) | −1.547043344283(4) | −55193.346(7) | −2.154022089283(5) |
| 0.7 | −0.30472111986125(2) | −1.6253871098818(10) | −56889.031(2) | −1.451349814518(4) |
| 0.8 | −0.426144098149866(8) | −1.6595347035215(5) | −58474.737(2) | −1.009058134031(3) |
| 0.9 | −0.511476040894782(4) | −1.667959773943(3) | −59944.217(3) | −0.716675213508(7) |
| 1.0 | −0.5725122002500037(6) | −1.661099371730(4) | −61297.808(4) | −0.516074971233(7) |
| 1.1 | −0.6166414355384560(5) | −1.645128821106(3) | −62539.821(3) | −0.374405409119(4) |
| 1.2 | −0.6486953222788965(4) | −1.623829401961(2) | −63676.895(2) | −0.272032297837(2) |
| 1.3 | −0.6719440628717529(2) | −1.5995760188437(9) | −64716.9283(10) | −0.196682994693(2) |
| 1.4 | −0.6886645852543717(2) | −1.5738875749463(5) | −65668.3886(7) | −0.1403988603129(7) |
| 1.5 | −0.70048012973757201(7) | −1.5477468953045(3) | −66539.8629(5) | −0.0978577572198(4) |
| 1.6 | −0.70857128863671537(7) | −1.5217932622403(2) | −67339.7667(4) | −0.0654066781045(3) |
| 1.7 | −0.71381153642099093(7) | −1.49644168780805(4) | −68076.1598(3) | −0.0404815382154(2) |
| 1.8 | −0.71685674809695454(7) | −1.47195862051467(4) | −68756.6349(2) | −0.02124729128935(5) |
| 1.9 | −0.71820578281118996(10) | −1.44851099645105(10) | −69388.2535(2) | −0.006368121488745(3) |
| 2.0 | −0.71824236670036556(7) | −1.42619857507619(9) | −69977.51475(8) | 0.005143079162299(4) |
| 2.1 | −0.71726459560211364(9) | −1.4050755662359(2) | −70530.34526(6) | 0.01402553569922(4) |
| 2.2 | −0.71550606600699063(8) | −1.3851652666310(2) | −71052.10228(4) | 0.02083948426503(5) |
| 2.3 | −0.71315123661799040(10) | −1.3664700568044(3) | −71547.58484(4) | 0.02601409410072(6) |
| 2.4 | −0.71034674581405077(9) | −1.3489782734655(3) | −72021.04919(3) | 0.02988134090111(7) |
| 2.5 | −0.7072098505635767(2) | −1.3326689496068(4) | −72476.22621(2) | 0.0327003006082(2) |
| 2.6 | −0.7038347876834872(2) | −1.3175150823969(4) | −72916.33900(2) | 0.03467480498851(10) |
| 2.7 | −0.7002976163305326(2) | −1.3034858736413(4) | −73344.11968(2) | 0.03596642926661(10) |
| 2.8 | −0.6966599372605290(2) | −1.2905482462189(5) | −73761.82521(2) | 0.0367041529651(2) |
| 2.9 | −0.6929717724196934(2) | −1.2786678457900(5) | −74171.251766(9) | 0.0369916203619(2) |
| 3.0 | −0.6892738105894307(2) | −1.2678096737223(6) | −74573.748307(9) | 0.0369126491522(2) |
| 3.1 | −0.6855991699852617(2) | −1.2579384541750(7) | −74970.229575(7) | 0.0365354470308(2) |
| 3.2 | −0.6819747896432710(2) | −1.2490188089329(8) | −75361.18954(2) | 0.0359158657355(2) |
| 3.3 | −0.6784225332837652(2) | −1.2410152935379(9) | −75746.716048(9) | 0.0350999312211(2) |
| 3.4 | −0.6749500688674244(3) | −1.23389233468(7) | −76126.50807(4) | 0.03412582443(2) |
| 3.5 | −0.6716015720323385(3) | −1.227614099682(2) | −76499.896608(10) | 0.0330254412521(3) |
| 3.6 | −0.6683582904851809(3) | −1.222144323209(2) | −76865.87056(2) | 0.0318256271560(3) |
| 3.7 | −0.6652389981417824(3) | −1.217446112362(2) | −77223.109145(8) | 0.0305491578168(3) |
| 3.8 | −0.6622503616102817(3) | −1.213481749661(2) | −77570.021556(2) | 0.0292155193578(3) |
| 3.9 | −0.6593972369372506(3) | −1.210212511924(2) | −77904.794961(9) | 0.0278415287054(3) |
| 4.0 | −0.6566829109953528(4) | −1.207598522484(2) | −78225.45115(2) | 0.0264418248767(4) |
| 4.1 | −0.654099299184826(4) | −1.20559865337372(3) | −78529.91142295(5) | 0.025024376828276(6) |
| 4.2 | −0.651667109027330(2) | −1.20417049276955(2) | −78816.069067695(6) | 0.023610410782170(3) |
| 4.3 | −0.649375977578229(2) | −1.20327039079930(2) | −79081.866994670(6) | 0.022205014966780(3) |
| 4.4 | −0.64722458923940(2) | −1.20285359342066(9) | −79325.3783950(2) | 0.02081717842230(2) |
| 4.5 | −0.645220779416894(4) | −1.202874469363(8) | −79544.886531(6) | 0.019459353216(2) |
| 4.6 | −0.64333162846020(3) | −1.2032868292099(2) | −79738.95969890(10) | 0.01812531037184(3) |
| 4.7 | −0.641583549389955(10) | −1.20404432901620(8) | −79906.5170664(2) | 0.01683463186462(2) |
| 4.8 | −0.639962372040222(5) | −1.20510094370474(4) | −80046.88111079(5) | 0.015588291744939(5) |
| 4.9 | −0.638463425400578(5) | −1.20641148920627(4) | −80159.81319833(5) | 0.014390890121405(5) |
| 5.0 | −0.6370916191536998(10) | −1.207932167067(4) | −80245.52976(3) | 0.0132502142482(5) |

| $1^1\Pi_u$ continued | | | | |
|---|---|---|---|---|
| $R$ | $E$ | $\langle V \rangle$ | $10^6 \cdot \langle \nabla_1 \cdot \nabla_2 \rangle$ | $\mathrm{d}E/\mathrm{d}R$ |
| 5.1 | −0.635811524688255(5) | −1.20962110234689(4) | −80304.6977420516(5) | 0.012157244515612(5) |
| 5.2 | −0.634647455255780(5) | −1.21143884533120(3) | −80338.41035424(3) | 0.011126166380839(4) |
| 5.3 | −0.633583544463294(5) | −1.21334880994012(3) | −80348.14407516(3) | 0.010154392261598(4) |
| 5.4 | −0.632613821972769(5) | −1.21531762680567(3) | −80335.70120869(2) | 0.009242595766643(4) |
| 5.5 | −0.6317422851233830(9) | −1.217315395743(6) | −80303.14167(3) | 0.0083907590010(6) |
| 5.6 | −0.630932965196095(5) | −1.21931583019345(3) | −80252.708736439(4) | 0.007598232178347(3) |
| 5.7 | −0.630209987181096(5) | −1.22129629421567(3) | −80186.75407951(2) | 0.006863803534477(3) |
| 5.8 | −0.629557622154015(5) | −1.22323773935119(3) | −80107.66535146(3) | 0.006185776716697(3) |
| 5.9 | −0.628970331676965(5) | −1.22512455456054(3) | −80017.800857694(6) | 0.005562052337862(3) |
| 6.0 | −0.628452803975520(2) | −1.22694434582(2) | −79919.43326(2) | 0.004990210357(2) |
| 6.5 | −0.6265344615036(9) | −1.234792805325(4) | −79368.7821037(10) | 0.0028117104127(4) |
| 7.0 | −0.6254830758624(10) | −1.240434316360(4) | −78846.9515496(10) | 0.0015045479093(3) |
| 7.5 | −0.6249345126910(2) | −1.244200333827(10) | −78438.3159(7) | 0.000758492207(2) |
| 8.0 | −0.624679211501909(7) | −1.246601880059(7) | −78153.76591(3) | 0.000344567868(2) |
| 8.5 | −0.624568123253735(5) | −1.248086820078(6) | −77972.71109(2) | 0.0001234619326(10) |
| 9.0 | −0.624537960784432(2) | −1.248983581122(5) | −77867.575707(9) | 0.0000102600494(8) |
| 9.5 | −0.6245481466282422(8) | −1.249513834665(4) | −77813.945687(6) | −0.0000439517273(6) |
| 10.0 | −0.6245767350901419(3) | −1.249820500254(3) | −77793.254095(4) | −0.0000667030075(4) |
| 11.0 | −0.6246486388186960(2) | −1.25008649610831(4) | −77802.9074258(2) | −0.000071747133719(2) |
| 12.0 | −0.62471513973456472(10) | −1.25015485752458(10) | −77837.4046086(2) | −0.000060381504619(6) |
| 13.0 | −0.62476909754281706(2) | −1.25015927265955(10) | −77873.8851086(3) | −0.000047775197993(6) |
| 14.0 | −0.62481143329763644(2) | −1.25014525348072(10) | −77905.2293572(2) | −0.000037313348959(6) |
| 15.0 | −0.624844524351388597(4) | −1.25012757382227(10) | −77930.3020114(2) | −0.000029235007965(6) |
| 16.0 | −0.624870551390126816(2) | −1.2501107229993(2) | −77949.87476202(4) | −0.000023101263688(6) |
| 17.0 | −0.6248912155003121249(7) | −1.2500958590476(2) | −77965.09763516(6) | −0.000018436943939(7) |
| 18.0 | −0.6249077873851430764(5) | −1.2500830959983(2) | −77977.0072788(2) | −0.000014862290444(9) |
| 19.0 | −0.6249212086986736248(3) | −1.2500722421742(3) | −77986.4190265(3) | −0.000012096040887(10) |
| 20.0 | −0.6249321801986659208(2) | −1.2500630369473(3) | −77993.9426143(4) | −0.00000993382749(2) |

TABLE S10. Calculated BO energies, expectation value of potential, $\langle \nabla_1 \cdot \nabla_2 \rangle$, and $\mathrm{d}E/\mathrm{d}R$ of the $2^1\Pi_u$ state in atomic units (hartree). Uncertainties originate purely from extrapolation to the complete basis set limit. United atom values at $R = 0$ are taken from Ref. [1].

| $2^1\Pi_\mathrm{u}$ | | | | |
|---|---|---|---|---|
| $R$ | $E$ | $\langle V \rangle$ | $10^6 \cdot \langle \nabla_1 \cdot \nabla_2 \rangle$ | $\mathrm{d}E/\mathrm{d}R$ |
| 0.0 | −2.05514636209194(3) | – | −14548.047097(1) | – |
| 0.01 | 97.94511517135(10) | 95.8907481378(4) | −14550.6(3) | −9999.94822049(2) |
| 0.05 | 17.950881130(2) | 15.913201507(7) | −14596.8(3) | −399.77121507(10) |
| 0.1 | 7.966627265(2) | 5.972387177(10) | −14720.25(8) | −99.60867352(8) |
| 0.15 | 4.6558326467(8) | 2.720436298(6) | −14897.19(9) | −43.94152664(3) |
| 0.2 | 3.0162913325(5) | 1.147931870(4) | −15109.80(9) | −24.42325398(2) |
| 0.3 | 1.4116045615(2) | −0.315236556(2) | −15595.7(2) | −10.461485595(3) |
| 0.4 | 0.64430269414(8) | −0.9456857053(6) | −16113.49(5) | −5.585727734(2) |
| 0.5 | 0.21016522518(8) | −1.2548350840(3) | −16629.6(3) | −3.3503310688(3) |
| 0.6 | −0.0595555925(2) | −1.4131329195(3) | −17125.5(5) | −2.1567028917(8) |
| 0.7 | −0.237242357038(7) | −1.49247785835(2) | −17589.48(4) | −1.454275920391(8) |
| 0.8 | −0.358968543370(6) | −1.52768895743(3) | −18020.62(3) | −1.01218983836(2) |
| 0.9 | −0.444622398405(8) | −1.53722309917(3) | −18416.56(4) | −0.719975891513(10) |
| 1.0 | −0.505995654029(7) | −1.531502113127(10) | −18777.89(4) | −0.519510805078(5) |
| 1.1 | −0.550473919665(7) | −1.51668754663(2) | −19106.24(4) | −0.377945188456(3) |
| 1.2 | −0.582885772892(7) | −1.496548241043(9) | −19403.79(4) | −0.275647246058(5) |
| 1.3 | −0.606498653130(6) | −1.47344788730(2) | −19672.94(3) | −0.200346600797(3) |
| 1.4 | −0.623586943478(6) | −1.44889528142(2) | −19916.19(3) | −0.1440867103279(8) |
| 1.5 | −0.635771540644(6) | −1.42386412860(2) | −20135.97(2) | −0.101547364875(5) |
| 1.6 | −0.644230877691(6) | −1.39898546239(2) | −20334.57(2) | −0.069077316879(6) |
| 1.7 | −0.649836437571(8) | −1.37466680677(2) | −20514.17(4) | −0.04411407745(2) |
| 1.8 | −0.653242255418(7) | −1.35116778045(2) | −20676.64(3) | −0.0248240386788(7) |
| 1.9 | −0.654945486842(6) | −1.32864905535(2) | −20823.80(2) | −0.009872674561(4) |
| 2.0 | −0.655328276407(8) | −1.307204609756(10) | −20957.27(3) | 0.001725971524(3) |
| 2.1 | −0.654687247073(6) | −1.28688328429(3) | −21078.33(2) | 0.010710099932(5) |
| 2.2 | −0.653254619118(5) | −1.26770335866(2) | −21188.26(2) | 0.0176390361724(2) |
| 2.3 | −0.651213560945(7) | −1.249662501071(5) | −21288.06(3) | 0.022941139479(4) |
| 2.4 | −0.648709497184(6) | −1.23274460533(3) | −21378.559(8) | 0.026947662098(8) |
| 2.5 | −0.645858539690(6) | −1.21692450850(2) | −21460.51(2) | 0.029917028351(2) |
| 2.6 | −0.642753842361(5) | −1.202171249781(10) | −21534.43(2) | 0.0320524749773(2) |
| 2.7 | −0.639470438773(6) | −1.18845031572(3) | −21600.726(10) | 0.033515022897(6) |
| 2.8 | −0.636068958176(7) | −1.17572517599(4) | −21659.717(10) | 0.034433121558(7) |
| 2.9 | −0.632598503520(6) | −1.16395831943(2) | −21711.57(2) | 0.034909892279(2) |
| 3.0 | −0.629098897264(6) | −1.153111936916(6) | −21756.33(2) | 0.035028619200(2) |
| 3.1 | −0.625602445941(6) | −1.14314835406(2) | −21793.95(2) | 0.034856947686(2) |
| 3.2 | −0.622135335353(6) | −1.13403028727(2) | −21824.33(2) | 0.034450119824(3) |
| 3.3 | −0.618718740083(8) | −1.12572097592(6) | −21847.260(5) | 0.03385348613(2) |
| 3.4 | −0.615369710545(6) | −1.11818422886(2) | −21862.51(2) | 0.03310446830378(10) |
| 3.5 | −0.612101885658(6) | −1.111384413670(9) | −21869.74(2) | 0.0322341021831(8) |
| 3.6 | −0.608926068091(6) | −1.10528640950(2) | −21868.62(2) | 0.0312682574118(4) |
| 3.7 | −0.605850690616(6) | −1.09985553953(2) | −21858.82(2) | 0.0302286058649(3) |
| 3.8 | −0.602882195833(7) | −1.09505749537(2) | −21839.99(2) | 0.0291333937609(3) |
| 3.9 | −0.600025346725(7) | −1.09085826292(2) | −21811.82(2) | 0.0279980591102(3) |
| 4.0 | −0.597283481822(7) | −1.08722405734(2) | −21774.04(2) | 0.02683572657513(2) |
| 4.1 | −0.594658725960(6) | −1.08412127333(3) | −21726.455(6) | 0.025657604533(3) |
| 4.2 | −0.592152165391(4) | −1.081516455297(7) | −21668.98(2) | 0.024473303683(4) |
| 4.3 | −0.589763994311(7) | −1.07937629126(2) | −21601.58(2) | 0.02329109240965(5) |
| 4.4 | −0.587493638503(5) | −1.07766763303(3) | −21524.381(5) | 0.022118100903(3) |
| 4.5 | −0.585339860710(6) | −1.07635754385(2) | −21437.679(10) | 0.0209604839049(2) |
| 4.6 | −0.583300851470(4) | −1.075413374016(2) | −21341.844(7) | 0.019823549764(2) |
| 4.7 | −0.581374308459(6) | −1.07480286326(3) | −21237.443(2) | 0.018711862481(4) |
| 4.8 | −0.579557506745(6) | −1.074494267433(3) | −21125.203(9) | 0.017629322092(2) |
| 4.9 | −0.577847361884(3) | −1.074456506058(2) | −21005.927(6) | 0.016579228102(2) |
| 5.0 | −0.576240487369(5) | −1.074659325367(3) | −20880.604(7) | 0.015564329870(2) |

| $2^1\Pi_u$ continued | | | | |
|---|---|---|---|---|
| $R$ | $E$ | $\langle V\rangle$ | $10^6\cdot\langle\nabla_1\cdot\nabla_2\rangle$ | $\mathrm{d}E/\mathrm{d}R$ |
| 5.1 | −0.5747332477(3) | −1.0750734719(8) | −20750.5(2) | 0.01458686733(8) |
| 5.2 | −0.5733218068(3) | −1.0756708651(10) | −20616.3(2) | 0.01364860550(10) |
| 5.3 | −0.5720021754(3) | −1.076424772(2) | −20479.5(2) | 0.0127508639(2) |
| 5.4 | −0.5707702529(3) | −1.077309963(2) | −20341.2(2) | 0.0118945449(2) |
| 5.5 | −0.569621868018(4) | −1.07830285189(2) | −20202.32(2) | 0.011080160751(5) |
| 5.7 | −0.5675588990(4) | −1.080526260(3) | −19928.6(2) | 0.0095774629(4) |
| 5.8 | −0.5666359442(4) | −1.081718693(4) | −19795.2(2) | 0.0088884820(6) |
| 5.9 | −0.5657798469(5) | −1.082942727(5) | −19665.2(2) | 0.0082401638(7) |
| 6.0 | −0.5649865882492(2) | −1.084184057324(5) | −19538.938(3) | 0.0076315198622(9) |
| 6.5 | −0.56183080960121(4) | −1.090273456485(2) | −18976.6363(4) | 0.0051366404181(2) |
| 7.0 | −0.55972210610446(5) | −1.09558524074(2) | −18505.163(3) | 0.003408424495(2) |
| 7.5 | −0.5583288376230(4) | −1.09983725612(2) | −18039.6654(3) | 0.002242722550(2) |
| 8.0 | −0.5574145446368(2) | −1.103088169639(7) | −17463.9949(3) | 0.0014676149544(8) |
| 8.5 | −0.55681752585672(6) | −1.1055089749790(10) | −16656.7985(3) | 0.00095600902760(8) |
| 9.0 | −0.5564294172808(10) | −1.10727807955(3) | −15509.5462(4) | 0.000620083891(3) |
| 9.5 | −0.5561780284343(7) | −1.10854370615(2) | −13972.5310(2) | 0.000401300075(2) |
| 10.0 | −0.5560150859946(9) | −1.10941910879(2) | −12134.7702(4) | 0.000261106320(2) |
| 11.0 | −0.5558361283483(2) | −1.110358904788(3) | −8553.38701(4) | 0.0001193956281(2) |
| 12.0 | −0.5557479986964(7) | −1.110715426413(9) | −6203.63848(3) | 0.0000650475817(5) |
| 13.0 | −0.5556961115907(5) | −1.110851220285(5) | −4962.1459(3) | 0.0000416156074(2) |
| 14.0 | −0.55566111306376(7) | −1.1109090270975(6) | −4334.1179(2) | 0.00002951421644(2) |
| 15.0 | −0.55563556713766(5) | −1.1109399002889(3) | −4008.50164(8) | 0.0000220822657683(9) |
| 16.0 | −0.55561622332729(3) | −1.11096252165040(10) | −3821.87530(6) | 0.000016870312755(6) |
| 17.0 | −0.55560140904228(3) | −1.11098305464362(2) | −3688.95179(2) | 0.000012927261221(8) |
| 18.0 | −0.55559008007670(2) | −1.11100274834615(8) | −3564.92879(3) | 0.000009856211504(10) |
| 19.0 | −0.55558147283856(2) | −1.11102123499783(3) | −3426.99262(2) | 0.000007458456797(6) |
| 20.0 | −0.555574982611434(10) | −1.11103790313518(5) | −3265.135147(3) | 0.000005603104379(6) |

TABLE S11. Calculated BO energies, expectation value of potential, $\langle \nabla_1 \cdot \nabla_2 \rangle$, and $\mathrm{d}E/\mathrm{d}R$ of the $3^1\Pi_u$ state in atomic units (hartree). Uncertainties originate purely from extrapolation to the complete basis set limit. United atom values at $R = 0$ are taken from Ref. [1].

| $3^1\Pi_\mathrm{u}$ | | | | |
|---|---|---|---|---|
| $R$ | $E$ | $\langle V \rangle$ | $10^6 \cdot \langle \nabla_1 \cdot \nabla_2 \rangle$ | $\mathrm{d}E/\mathrm{d}R$ |
| 0.0 | −2.031255144381749(1) | – | 10.0242694(2) | – |
| 0.01 | 97.96900621343(6) | 95.9385298721(4) | 10.026(3) | −9999.94825548(3) |
| 0.05 | 17.974768118(3) | 15.96096722(2) | 10.161(7) | −399.7713804(3) |
| 0.1 | 7.990502276(3) | 6.02010615(2) | 10.51(2) | −99.6089840(2) |
| 0.15 | 4.6796888490(6) | 2.768082789(4) | 10.94(8) | −43.94196606(2) |
| 0.2 | 3.040122617(3) | 1.19548336(2) | 11.70(9) | −24.42380937(5) |
| 0.3 | 1.4353699121(3) | −0.267933052(2) | 13.937(4) | −10.462242921(4) |
| 0.4 | 0.66798354391(9) | −0.8986952649(7) | 16.629(8) | −5.586655882(2) |
| 0.5 | 0.23374576882(4) | −1.2082111053(3) | 19.9735(8) | −3.3514052859(4) |
| 0.6 | −0.03608888848(2) | −1.36691910203(10) | 23.9937(6) | −2.1579022085(2) |
| 0.7 | −0.213901063874(2) | −1.4467094737(3) | 28.48(2) | −1.4555819226(2) |
| 0.8 | −0.335762490242(9) | −1.48239380155(4) | 34.19(2) | −1.01358602633(3) |
| 0.9 | −0.421559845534(7) | −1.49242229645(4) | 40.51(2) | −0.72144733932(3) |
| 1.0 | −0.4830834382166(2) | −1.48721081710(2) | 47.721(7) | −0.52104394066(2) |
| 1.1 | −0.52771758166707(8) | −1.472915568114(8) | 55.876(6) | −0.379527640708(6) |
| 1.2 | −0.5602896712967(2) | −1.453300612159(10) | 65.070(5) | −0.277267724636(4) |
| 1.3 | −0.5840660672443(4) | −1.43072536750(2) | 75.396(5) | −0.201994794627(8) |
| 1.4 | −0.6013201666894(2) | −1.406694810571(10) | 86.955(5) | −0.145753197993(6) |
| 1.5 | −0.61367196530083(10) | −1.382179232022(8) | 99.862(5) | −0.103223534280(5) |
| 1.6 | −0.62229907235362(6) | −1.357806613543(7) | 114.245(5) | −0.070755293022(4) |
| 1.7 | −0.62807221744024(5) | −1.333981753549(5) | 130.25211(7) | −0.045786658040(3) |
| 1.8 | −0.63164474672497(8) | −1.310961841547(4) | 148.023(5) | −0.026484637832(2) |
| 1.9 | −0.63351318598876(4) | −1.288905393145(3) | 167.76002(10) | −0.011515274299(2) |
| 2.0 | −0.63405910469922(8) | −1.267904487228(4) | 189.64406(5) | 0.000106861085(2) |
| 2.1 | −0.63357860189655(7) | −1.248006312896(5) | 213.90473(4) | 0.009119471856(2) |
| 2.2 | −0.63230342242578(4) | −1.229227745287(4) | 240.79371(4) | 0.016081408893(2) |
| 2.3 | −0.63041630601095(7) | −1.211565302295(3) | 270.59474(4) | 0.0214205694467(10) |
| 2.4 | −0.62806229459085(7) | −1.195001998137(6) | 303.628453(5) | 0.025467746269(2) |
| 2.5 | −0.62535716359586(3) | −1.179512087631(4) | 340.24(2) | 0.028480895824(2) |
| 2.6 | −0.62239377820286(4) | −1.165064362910(4) | 380.893(2) | 0.030662766729(2) |
| 2.7 | −0.61924693362574(5) | −1.151624449532(4) | 426.00871(2) | 0.032173858415(2) |
| 2.8 | −0.6159770751770(2) | −1.1391564080602(3) | 476.1317(7) | 0.0331420508181(10) |
| 2.9 | −0.61263318190023(4) | −1.127623853581(5) | 531.88119(2) | 0.033669831110(2) |
| 3.0 | −0.60925501978092(6) | −1.116990742842(6) | 593.950(2) | 0.033839765574(2) |
| 3.1 | −0.60587491575974(7) | −1.107221936474(10) | 663.14947(7) | 0.033718675821(3) |
| 3.2 | −0.60251916477657(8) | −1.098283615007(8) | 740.400(2) | 0.033360848296(2) |
| 3.3 | −0.59920915398249(3) | −1.09014360839(2) | 826.775008(6) | 0.032810515025(3) |
| 3.4 | −0.59596226786315(7) | −1.08277168615(2) | 923.50533(2) | 0.032103779288(4) |
| 3.5 | −0.59279262307761(6) | −1.076139847821(7) | 1032.01979(2) | 0.031270113810(2) |
| 3.6 | −0.58971167080997(7) | −1.070222648863(7) | 1153.9694(4) | 0.030333525766(2) |
| 3.7 | −0.58672869628358(7) | −1.064997596083(2) | 1291.24(2) | 0.0293134585088(5) |
| 3.8 | −0.58385123904255(7) | −1.060445646756(9) | 1446.099(2) | 0.028225481929(2) |
| 3.9 | −0.58108545310471(8) | −1.056551846253(6) | 1620.996(3) | 0.027081810245(2) |
| 4.0 | −0.57843642270569(9) | −1.05330613846(2) | 1818.8164(9) | 0.025891676738(3) |
| 4.1 | −0.5759084467052(8) | −1.05070437618(2) | 2042.746(2) | 0.024661589569(3) |
| 4.2 | −0.5735053023974(10) | −1.04874953849(2) | 2296.2556(6) | 0.023395491978(4) |
| 4.3 | −0.571230496915(5) | −1.047453115(2) | 2581.2(8) | 0.0220948552(6) |
| 4.4 | −0.569087510704(2) | −1.04683648738(4) | 2906.221(2) | 0.020758757733(7) |
| 4.5 | −0.5670800314725(3) | −1.0469320172(2) | 3268.79(2) | 0.01938401017(3) |
| 4.6 | −0.565212165924(3) | −1.04778301555(7) | 3671.720(2) | 0.01796550354(2) |
| 4.7 | −0.563488598378(4) | −1.04944140503(8) | 4112.864(3) | 0.01649697696(2) |
| 4.8 | −0.561914636653(5) | −1.05196096510(10) | 4584.85(2) | 0.01497256421(2) |
| 4.9 | −0.560496048521(5) | −1.0553835663(2) | 5072.445(4) | 0.01338949607(3) |
| 5.0 | −0.5592385599918(7) | −1.0597163384(4) | 5549.84(5) | 0.01175215632(6) |

| $3^1\Pi_u$ continued | | | | |
|---|---|---|---|---|
| $R$ | $E$ | $\langle V\rangle$ | $10^6\cdot\langle\nabla_1\cdot\nabla_2\rangle$ | $\mathrm{d}E/\mathrm{d}R$ |
| 5.5 | −0.555416132802(2) | −1.08968313657(7) | 6362.383(8) | 0.00384529619(2) |
| 6.0 | −0.554668430236(2) | −1.10964769596(3) | 3550.674(6) | −0.000051805914(3) |
| 6.5 | −0.554932208220(2) | −1.11458878863(6) | 432.42041(10) | −0.00072682650(2) |
| 7.0 | −0.5552660307472(4) | −1.114487170634(5) | −1647.2922(5) | −0.0005650155912(4) |
| 7.5 | −0.5554874525832(3) | −1.113433000190(3) | −2919.0298(3) | −0.0003277460031(2) |
| 8.0 | −0.5556053571365(3) | −1.112462195983(2) | −3771.2760(7) | −0.00015643521369(7) |
| 8.5 | −0.5556551702212(3) | −1.111755460336(2) | −4526.5582(5) | −0.000052367046307(10) |
| 9.0 | −0.5556654965765(2) | −1.1112869171620(4) | −5430.4476(4) | 0.00000489733220(9) |
| 9.5 | −0.5556551596727(2) | −1.1110003941295(5) | −6624.8485(5) | 0.0000326237068(2) |
| 10.0 | −0.5556359044567(2) | −1.110851459399(2) | −8081.5902(2) | 0.0000420349513(3) |
| 11.0 | −0.55559625780807(5) | −1.110821829684(2) | −10924.41678(5) | 0.0000336987211(2) |
| 12.0 | −0.55557051756912(4) | −1.110920828423(2) | −12669.1260(2) | 0.0000183505596(2) |
| 13.0 | −0.555557556335343(10) | −1.1110033781885(2) | −13464.7135(2) | 0.00000859496016(3) |
| 14.0 | −0.555551692841503(6) | −1.11105115476994(7) | −13784.1981(2) | 0.000003730779506(2) |
| 15.0 | −0.55554924751854(2) | −1.1110767936785(2) | −13905.2087(2) | 0.00000144675723(2) |
| 16.0 | −0.555548402978363(8) | −1.111090799347596(4) | −13960.3639(2) | 0.000000375413066(3) |
| 17.0 | −0.555548311291048(7) | −1.111098811867588(4) | −14010.9171(2) | −0.000000128781503(3) |
| 18.0 | −0.55554857089486(2) | −1.1111036080589(2) | −14084.4411(2) | −0.000000359237173(5) |
| 19.0 | −0.555548984947825(9) | −1.1111065785693(2) | −14192.02608(10) | −0.00000045308809(2) |
| 20.0 | −0.555549454309680(8) | −1.1111084613651(2) | −14335.99101(9) | −0.00000047763729(2) |

TABLE S12. Calculated BO energies, expectation value of potential, $\langle \nabla_1 \cdot \nabla_2 \rangle$, and $\mathrm{d}E/\mathrm{d}R$ of the $4^1\Pi_u$ state in atomic units (hartree). Uncertainties originate purely from extrapolation to the complete basis set limit. United atom values at $R = 0$ are taken from Ref. [1].

| $4^1\Pi_u$ | | | | |
|---|---|---|---|---|
| $R$ | $E$ | $\langle V \rangle$ | $10^6 \cdot \langle \nabla_1 \cdot \nabla_2 \rangle$ | $\mathrm{d}E/\mathrm{d}R$ |
| 0.0 | −2.03106965045024(3) | – | −6254.9235543(1) | – |
| 0.01 | 97.96919178520(6) | 95.9389011706(4) | −6255.859(9) | −9999.94823998(3) |
| 0.05 | 17.974955488(2) | 15.96134562(2) | −6274.951(2) | −399.7713070(2) |
| 0.1 | 7.990694954(4) | 6.02050527(3) | −6326.740(5) | −99.6088464(3) |
| 0.15 | 4.679889863(2) | 2.76851403(2) | −6403(2) | −43.94177128(6) |
| 0.2 | 3.0403346762(8) | 1.195956722(7) | −6489.7(3) | −24.42356315(3) |
| 0.3 | 1.4356112125(3) | −0.267349651(3) | −6691.37678(9) | −10.461906918(6) |
| 0.4 | 0.6682623581(3) | −0.897972708(3) | −6906.67(2) | −5.586243561(5) |
| 0.5 | 0.23406918181(4) | −1.2073252509(3) | −7120.619(3) | −3.3509272290(5) |
| 0.6 | −0.03571475804(4) | −1.3658498886(4) | −7325.72(3) | −2.1573672875(5) |
| 0.7 | −0.21347092383(2) | −1.44544035045(9) | −7518.078(8) | −1.45499786113(10) |
| 0.8 | −0.335271776213(6) | −1.48091130513(5) | −7696.067(7) | −1.01295969088(5) |
| 0.9 | −0.421004643982(4) | −1.49071569864(4) | −7859.23(2) | −0.72078490076(3) |
| 1.0 | −0.482460422266(3) | −1.48527181946(4) | −8007.87(2) | −0.52035097492(3) |
| 1.1 | −0.527023955252(4) | −1.47073802835(3) | −8142.70(2) | −0.37880919804(3) |
| 1.2 | −0.559523119342(4) | −1.45088029758(3) | −8264.60(3) | −0.27652838242(2) |
| 1.3 | −0.583224710587(4) | −1.42805973147(3) | −8374.59(3) | −0.20123870023(2) |
| 1.4 | −0.600402520940(4) | −1.40378278899(3) | −8473.68(3) | −0.14498410508(2) |
| 1.5 | −0.612676903060(4) | −1.37902105684(3) | −8562.84(4) | −0.10244483381(2) |
| 1.6 | −0.621225788304(5) | −1.35440364006(4) | −8643.02(4) | −0.06997003966(2) |
| 1.7 | −0.626920195845(5) | −1.33033629813(3) | −8715.01(4) | −0.044997592024(10) |
| 1.8 | −0.630413730895(6) | −1.30707702612(3) | −8779.64(5) | −0.025694202406(8) |
| 1.9 | −0.632203149262(6) | −1.28478499264(4) | −8837.59(5) | −0.01072562849(2) |
| 2.0 | −0.632670222456(6) | −1.26355277577(5) | −8889.42(5) | 0.00089383457(2) |
| 2.1 | −0.632111224111(7) | −1.24342790420(5) | −8935.67(6) | 0.00990216381(2) |
| 2.2 | −0.630758046230(9) | −1.22442742240(5) | −8976.79(6) | 0.01685848639(2) |
| 2.3 | −0.628793547669(7) | −1.20654783089(3) | −9013.08(6) | 0.022190984542(2) |
| 2.4 | −0.626362860314(8) | −1.18977191740(3) | −9044.94(6) | 0.0262307513462(6) |
| 2.5 | −0.623581818423(9) | −1.17407347105(5) | −9072.64(7) | 0.029236066315(10) |
| 2.6 | −0.620543312213(8) | −1.15942054060(2) | −9096.12(6) | 0.0314100322442(3) |
| 2.7 | −0.617322124591(9) | −1.14577768231(6) | −9115.84(7) | 0.032913543285(8) |
| 2.8 | −0.613978646581(9) | −1.13310750028(3) | −9131.45(6) | 0.0338749260328(4) |
| 2.9 | −0.610561755163(10) | −1.12137169105(3) | −9143.32(6) | 0.034397179063(2) |
| 3.0 | −0.60711105923(2) | −1.11053173672(6) | −9151.17(4) | 0.034563460575(8) |
| 3.1 | −0.60365866464(2) | −1.10054935104(8) | −9155.22(4) | 0.03444128330(2) |
| 3.2 | −0.60023057028(2) | −1.09138675154(6) | −9155.24(4) | 0.034085746563(7) |
| 3.3 | −0.59684777871(2) | −1.08300680946(6) | −9151.110(3) | 0.033542044836(5) |
| 3.4 | −0.59352718475(2) | −1.07537311580(4) | −9142.69(2) | 0.032847427561(4) |
| 3.5 | −0.59028228983(2) | −1.06844999151(7) | −9129.822(3) | 0.032032739469(6) |
| 3.6 | −0.58712377929(2) | −1.06220246042(7) | −9112.374(6) | 0.031123638375(6) |
| 3.7 | −0.58405999085(2) | −1.05659620211(7) | −9090.180(8) | 0.030141562048(5) |
| 3.8 | −0.58109729660(2) | −1.05159749355(7) | −9063.092(4) | 0.029104499910(6) |
| 3.9 | −0.57824041584(2) | −1.04717314892(10) | −9030.97884(2) | 0.02802761097(2) |
| 4.0 | −0.57549267233(2) | −1.04329046377(2) | −8993.91(7) | 0.026923720211(10) |
| 4.1 | −0.57285620704(2) | −1.03991716734(2) | −8951.49(7) | 0.025803718673(2) |
| 4.2 | −0.57033215480(4) | −1.0370213886(2) | −8903.71(2) | 0.024676885945(9) |
| 4.3 | −0.56792079200(2) | −1.034571636684(7) | −8850.98(6) | 0.023551150480(3) |
| 4.4 | −0.56562166080(3) | −1.03253680390(3) | −8793.13(8) | 0.022433299424(2) |
| 4.5 | −0.563433674549(10) | −1.030886186793(4) | −8730.12(4) | 0.021329147173(4) |
| 4.6 | −0.56135520807(2) | −1.02958953703(2) | −8662.68(8) | 0.02024366934(2) |
| 4.7 | −0.55938417602(2) | −1.02861713785(2) | −8590.72(6) | 0.01918110942(2) |
| 4.8 | −0.55751810183(2) | −1.027939913574(8) | −8514.794(5) | 0.01814506040(2) |
| 4.9 | −0.55575417941(4) | −1.02752956681(3) | −8435.84(7) | 0.017138529015(3) |
| 5.0 | −0.554089329273(10) | −1.02735874132(7) | −8353.933(6) | 0.016163983447(10) |

| $4^1\Pi_u$ continued | | | | |
|---|---|---|---|---|
| $R$ | $E$ | $\langle V \rangle$ | $10^6 \cdot \langle \nabla_1 \cdot \nabla_2 \rangle$ | $\mathrm{d}E/\mathrm{d}R$ |
| 5.5 | −0.547130494300(7) | −1.02922781957(8) | −7936.90(9) | 0.01182421254(3) |
| 6.0 | −0.542110507075(9) | −1.033783152(4) | −7591.85(4) | 0.0084063103(7) |
| 6.5 | −0.5385829807664(5) | −1.03924597591(2) | −7382.925(7) | 0.005833843942(2) |
| 7.0 | −0.5361589831596(6) | −1.04454759093(2) | −7279.964(8) | 0.003967196485(2) |
| 7.5 | −0.534523275932(8) | −1.04912705530(8) | −7215.00(8) | 0.00265593287(2) |
| 8.0 | −0.533434102274(5) | −1.05279525231(5) | −7134.77(6) | 0.001759119026(8) |
| 8.5 | −0.532715078128(5) | −1.05558966628(5) | −7012.82(6) | 0.001157704698(8) |
| 9.0 | −0.532242655247(4) | −1.05764888576(4) | −6837.67(5) | 0.000759602746(6) |
| 9.5 | −0.531932821972(2) | −1.05913365382(3) | −6600.445(10) | 0.000498104224(2) |
| 10.0 | −0.531729575482(2) | −1.06018961805(3) | −6287.512(9) | 0.000326953291(2) |
| 11.0 | −0.5315091958367(8) | −1.06153320476(7) | −5234.371(7) | 0.000135016991(7) |
| 12.0 | −0.531444947891(2) | −1.06245559262(5) | −1615.23(2) | 0.000036191930(3) |
| 13.0 | −0.531414787611(3) | −1.06249922172(5) | −1420.78(2) | 0.000025411808(3) |
| 14.0 | −0.531392772851(3) | −1.06251852662(5) | −1347.81(2) | 0.000019072792(3) |
| 15.0 | −0.531375882969(3) | −1.06252638105(5) | −1255.64(3) | 0.000015025659(2) |
| 16.0 | −0.531362195352(3) | −1.06252343116(4) | −1145.97(3) | 0.000012559972(2) |
| 17.0 | −0.531350434205(3) | −1.06251240472(4) | −1035.33(2) | 0.000011086100(2) |
| 18.0 | −0.531339840773(3) | −1.06249672282(3) | −935.07(2) | 0.0000101643735(9) |
| 19.0 | −0.531330020045(2) | −1.06247948779(3) | −850.73(2) | 0.0000095027525(7) |
| 20.0 | −0.531320808096(2) | −1.06246310788(2) | −784.12(2) | 0.0000089254159(5) |

TABLE S13. Calculated BO energies, expectation value of potential, $\langle \nabla_1 \cdot \nabla_2 \rangle$, and $\mathrm{d}E/\mathrm{d}R$ of the $1^3\Pi_u$ state in atomic units (hartree). Uncertainties originate purely from extrapolation to the complete basis set limit. United atom values at $R = 0$ are taken from Ref. [1].

| $1^3\Pi_\mathrm{u}$ | | | | |
|---|---|---|---|---|
| $R$ | $E$ | $\langle V \rangle$ | $10^6 \cdot \langle \nabla_1 \cdot \nabla_2 \rangle$ | $\mathrm{d}E/\mathrm{d}R$ |
| 0.0 | −2.123843086498093(2) | – | 64572.425024(4) | – |
| 0.01 | 97.86709492124(2) | 95.73470285376(9) | 64585.06318(3) | −9999.948698872(7) |
| 0.05 | 17.8728183563(2) | 15.756952570(2) | 64860.67829(6) | −399.77328286(3) |
| 0.1 | 7.88842353645(6) | 5.8156116724(9) | 65603.91522(5) | −99.612154006(7) |
| 0.15 | 4.5774293771(5) | 2.562944028(4) | 66657.392(2) | −43.94609817(2) |
| 0.2 | 2.937639120191(10) | 0.98961256543(9) | 67915.9848(10) | −24.4283283748(4) |
| 0.3 | 1.3324174365043(7) | −0.47534337084(2) | 70761.19780(2) | −10.46719414615(5) |
| 0.4 | 0.5645364079553(2) | −1.107561169738(7) | 73733.01047(2) | −5.59153496412(2) |
| 0.5 | 0.1298272808145(2) | −1.418323094452(5) | 76602.419188(10) | −3.355915312162(7) |
| 0.6 | −0.14043207358477(8) | −1.578002013033(3) | 79239.842496(7) | −2.161863109772(4) |
| 0.7 | −0.318618175318982(10) | −1.658456709946(6) | 81575.610(2) | −1.458886227582(4) |
| 0.8 | −0.440774586238020(4) | −1.69448898162579(5) | 83578.02105(7) | −1.016174761442(4) |
| 0.9 | −0.5267938790676480(2) | −1.704553656081(4) | 85239.9819(2) | −0.723295442164(5) |
| 1.0 | −0.5884651352607144(2) | −1.6990808718222(9) | 86570.3074(3) | −0.522150601302(2) |
| 1.1 | −0.63317350636365122(7) | −1.6842474227727(10) | 87587.771077(7) | −0.379909463678(2) |
| 1.2 | −0.66574870265886954(10) | −1.6638418158373(3) | 88316.97630(3) | −0.2769536754333(5) |
| 1.3 | −0.68946043541486091(6) | −1.6402499598424(2) | 88785.47514(3) | −0.2010223761637(3) |
| 1.4 | −0.70658615416404380(6) | −1.61500405128016(2) | 89021.78568(4) | −0.14416553068014(7) |
| 1.5 | −0.71875035217035077(7) | −1.58910139498553(5) | 89054.06279(2) | −0.10106712709657(3) |
| 1.6 | −0.72713538673373312(6) | −1.56319614059885(5) | 88909.244594(8) | −0.068078354457113(7) |
| 1.7 | −0.73261683909347919(6) | −1.53771799311280(8) | 88612.541423(6) | −0.04263783230930(2) |
| 1.8 | −0.73585290173154405(8) | −1.5129475405081(2) | 88187.167435(5) | −0.02291207613610(7) |
| 1.9 | −0.73734486220859607(7) | −1.4890650647139(2) | 87654.240729(4) | −0.00756596857721(6) |
| 2.0 | −0.73747891123618292(5) | −1.4661827411580(2) | 87032.796807(2) | 0.00438754065720(5) |
| 2.1 | −0.73655559047517172(8) | −1.4443662061127(2) | 86339.875093(3) | 0.01368808325602(7) |
| 2.2 | −0.73481088429473340(6) | −1.4236491890151(2) | 85590.649687(3) | 0.02089662707928(7) |
| 2.3 | −0.73243155451833786(9) | −1.4040435449615(3) | 84798.5838315(9) | 0.02644328872833(9) |
| 2.4 | −0.72956644077963539(8) | −1.3855461904592(3) | 83975.594054(2) | 0.03066112129173(9) |
| 2.5 | −0.72633488990980888(10) | −1.3681439263878(4) | 83132.2143823(8) | 0.03381034137273(10) |
| 2.6 | −0.72283311357693170(7) | −1.3518168021408(3) | 82277.754425(2) | 0.03609593269734(8) |
| 2.7 | −0.71913903175379168(9) | −1.3365404615788(4) | 81420.447444(3) | 0.03768059330696(10) |
| 2.8 | −0.7153159965322639(2) | −1.3222877713946(6) | 80567.5860983(7) | 0.0386943648821(2) |
| 2.9 | −0.7114156790624591(2) | −1.3090299392872(6) | 79725.644681(2) | 0.0392418685648(2) |
| 3.0 | −0.7074803247316160(2) | −1.2967372665477(6) | 78900.387381(4) | 0.0394077943052(2) |
| 3.1 | −0.7035445270119220(2) | −1.2853796368801(7) | 78096.962483(3) | 0.0392611023045(2) |
| 3.2 | −0.6996366314351171(2) | −1.2749268138770(7) | 77319.982743(5) | 0.0388582653104(2) |
| 3.3 | −0.6957798530696988(2) | −1.2653485992047(8) | 76573.592347(5) | 0.0382457899802(2) |
| 3.4 | −0.6919931704330150(2) | −1.2566148893943(9) | 75861.520798(9) | 0.0374621916094(2) |
| 3.5 | −0.6882920437468887(2) | −1.248695659282(2) | 75187.124362(9) | 0.0365395509176(3) |
| 3.6 | −0.6846889943089719(3) | −1.241560893329(2) | 74553.415471(7) | 0.0355047486914(3) |
| 3.7 | −0.6811940734319673(3) | −1.235180481387(2) | 73963.080832(7) | 0.0343804501291(3) |
| 3.8 | −0.6778152431428819(3) | −1.229524092390(2) | 73418.48894(2) | 0.0331858931305(3) |
| 3.9 | −0.6745586860948836(3) | −1.224561037471(2) | 72921.687934(5) | 0.0319375217227(4) |
| 4.0 | −0.6714290585358247(3) | −1.220260132796(2) | 72474.394808(7) | 0.0306494960689(3) |
| 4.1 | −0.668419697416228(2) | −1.216589571777470(10) | 72077.977748200(5) | 0.029329225135362(2) |
| 4.2 | −0.665552790595878(2) | −1.213516815938344(10) | 71733.432921185(5) | 0.027997325060336(2) |
| 4.3 | −0.662819517465230(2) | −1.211008513393224(10) | 71441.358223023(6) | 0.026658260822613(2) |
| 4.4 | −0.660220166016223(2) | −1.20903045352423(2) | 71201.92614520(2) | 0.025320426933686(3) |
| 4.5 | −0.6577642313845241(4) | −1.207547565652(3) | 71014.85859(2) | 0.0239957549149(4) |
| 4.6 | −0.655420500069249(2) | −1.20652396828002(2) | 70879.40653889(2) | 0.022677615621408(3) |
| 4.7 | −0.653217123359737(2) | −1.20592307366320(2) | 70794.33710810(2) | 0.021385355969420(3) |
| 4.8 | −0.651141682917086(3) | −1.20570774991040(2) | 70757.93112519(2) | 0.020119919984119(3) |
| 4.9 | −0.649191250937030(3) | −1.20584053977854(2) | 70767.99287316(2) | 0.018886114713372(3) |
| 5.0 | −0.6473724468364923(6) | −1.206283931723(4) | 70821.87377(2) | 0.0176921923901(5) |

| $1^3\Pi_u$ continued | | | | |
|---|---|---|---|---|
| $R$ | $E$ | $\langle V \rangle$ | $10^6 \cdot \langle \nabla_1 \cdot \nabla_2 \rangle$ | $\mathrm{d}E/\mathrm{d}R$ |
| 5.1 | −0.645651491944746(3) | −1.20700067505292(2) | 70916.51063896(2) | 0.016529864477760(3) |
| 5.2 | −0.644054263236758(3) | −1.20795412753332(2) | 71048.47768681(2) | 0.015414307488499(3) |
| 5.3 | −0.642566346724458(3) | −1.20910862073727(2) | 71214.05152150(2) | 0.014344164662575(3) |
| 5.4 | −0.641183090731343(3) | −1.21042982656531(2) | 71409.28595620(2) | 0.013321547203217(3) |
| 5.5 | −0.6399096589310119(7) | −1.2118851076(2) | 71630.09374(8) | 0.01235167459(2) |
| 5.6 | −0.638711082746008(3) | −1.21344383419598(2) | 71872.33190288(2) | 0.011424702017150(2) |
| 5.7 | −0.637612312492567(3) | −1.21507765497993(2) | 72131.88489906(2) | 0.010552100000914(2) |
| 5.8 | −0.636598266527892(3) | −1.21676070722305(2) | 72404.74485478(2) | 0.009730314798748(2) |
| 5.9 | −0.635663877610870(3) | −1.21846976189146(2) | 72687.08246249(2) | 0.008958981920386(2) |
| 6.0 | −0.6348141357193404(9) | −1.22018429918(7) | 72975.30770(6) | 0.008240662047(8) |
| 6.5 | −0.631458245403886(10) | −1.22830667405602(5) | 74400.83955026(2) | 0.005324587192577(4) |
| 7.0 | −0.629313556242347(5) | −1.234912514982(2) | 75621.69638(3) | 0.003390656784(2) |
| 7.5 | −0.627950934798369(6) | −1.239758606917(7) | 76540.66137(2) | 0.002155101689(3) |
| 8.0 | −0.627091405366481(8) | −1.243109576993(6) | 77176.083217(10) | 0.001384154217(2) |
| 8.5 | −0.626528240798876(7) | −1.245351849010(2) | 77589.876500(8) | 0.000906427363(2) |
| 9.0 | −0.626155135224279(5) | −1.24682787628977(10) | 77846.947399(3) | 0.00060915490650(4) |
| 9.5 | −0.625900908966620(2) | −1.247794296651(4) | 77999.899097(7) | 0.0004218443453(5) |
| 10.0 | −0.6257222116757563(9) | −1.248428790364(3) | 78086.602799(6) | 0.0003015632987(4) |
| 11.0 | −0.6254955149381342(2) | −1.249132170440(2) | 78154.103490(4) | 0.0001689872214(2) |
| 12.0 | −0.62536199674893989(4) | −1.2494628008583(7) | 78161.053116(2) | 0.00010509938661(7) |
| 13.0 | −0.62527576869255419(4) | −1.249634289924639(7) | 78149.6506828(2) | 0.0000690190354204(8) |
| 14.0 | −0.62521632296272500(2) | −1.24973329021444(9) | 78134.4901374(5) | 0.00004995397935(2) |
| 15.0 | −0.625173439941072551(5) | −1.24979612121462(7) | 78120.1333767(3) | 0.000036717244498(7) |
| 16.0 | −0.625141481419891787(3) | −1.249839008982235(5) | 78107.7245893(2) | 0.000027747116094(3) |
| 17.0 | −0.625117069157575256(2) | −1.249869855226915(10) | 78097.3217796(2) | 0.000021428416954(2) |
| 18.0 | −0.6250980498764705517(6) | −1.24989288510072(3) | 78088.68150160(10) | 0.0000168452584580(3) |
| 19.0 | −0.6250829872020891020(4) | −1.24991056007342(4) | 78081.51129363(9) | 0.00001344285951499(9) |
| 20.0 | −0.6250708895747465466(2) | −1.24992441784911(4) | 78075.54447619(5) | 0.00001086806502036(6) |

TABLE S14. Calculated BO energies, expectation value of potential, $\langle \nabla_1 \cdot \nabla_2 \rangle$, and $\mathrm{d}E/\mathrm{d}R$ of the $2^3\Pi_u$ state in atomic units (hartree). Uncertainties originate purely from extrapolation to the complete basis set limit. United atom values at $R = 0$ are taken from Ref. [1].

| $2^3\Pi_\mathrm{u}$ | | | | |
|---|---|---|---|---|
| $R$ | $E$ | $\langle V \rangle$ | $10^6 \cdot \langle \nabla_1 \cdot \nabla_2 \rangle$ | $\mathrm{d}E/\mathrm{d}R$ |
| 0.0 | −2.05514636209194(3) | – | 18369.001636(2) | – |
| 0.01 | 97.9421796391(3) | 95.884875471(3) | 18371.511(10) | −9999.9483807(2) |
| 0.05 | 17.947927878(2) | 15.907259954(9) | 18426.39(2) | −399.7719160(2) |
| 0.1 | 7.963625847(2) | 5.966264626(9) | 18572.43(2) | −99.60987068(7) |
| 0.15 | 4.6527620903(7) | 2.714062972(6) | 18774.768(9) | −43.94307473(3) |
| 0.2 | 3.0131368395(4) | 1.141263959(4) | 19009.168(9) | −24.42504860(2) |
| 0.3 | 1.4082545724(2) | −0.3225595998(7) | 19507.1(2) | −10.463562482(2) |
| 0.4 | 0.6407387542(2) | −0.953685282(2) | 19974.5(2) | −5.587906975(3) |
| 0.5 | 0.20638302081(8) | −1.2634853360(5) | 20363.3(2) | −3.3525027553(6) |
| 0.6 | −0.06355156071(9) | −1.4223814891(6) | 20652.1(2) | −2.1587972795(6) |
| 0.7 | −0.241441962005(9) | −1.50225782108(2) | 20835.2(3) | −1.4562484246(2) |
| 0.8 | −0.363358090254(4) | −1.53792628057(7) | 20916.121(4) | −1.01401262507(7) |
| 0.9 | −0.449186022790(5) | −1.54784148556(4) | 20902.508(2) | −0.72163271109(3) |
| 1.0 | −0.510716296965(4) | −1.54242613630(3) | 20805.785(5) | −0.52099354237(2) |
| 1.1 | −0.555334013438(3) | −1.52784461499(3) | 20637.955(4) | −0.37925144375(2) |
| 1.2 | −0.587867720451(3) | −1.50786974158(3) | 20410.911(4) | −0.2767785838816(10) |
| 1.3 | −0.611585156943(3) | −1.48486975727(3) | 20135.845(4) | −0.20130726414(2) |
| 1.4 | −0.628761223602(5) | −1.46035818963(3) | 19822.905(10) | −0.14488267316(2) |
| 1.5 | −0.641017471263(3) | −1.43531339906(3) | 19481.089(9) | −0.10218563769(2) |
| 1.6 | −0.649533064212(4) | −1.41037083700(3) | 19118.167(6) | −0.06956544286(2) |
| 1.7 | −0.655180250875(3) | −1.38594211596(3) | 18740.769(5) | −0.04445977306(2) |
| 1.8 | −0.658613835899(3) | −1.36229057004(3) | 18354.478(7) | −0.02503494347(2) |
| 1.9 | −0.660331727693(3) | −1.33958020240(3) | 17963.955(7) | −0.009956182640(10) |
| 2.0 | −0.660716793295(3) | −1.31790794973(3) | 17573.029(7) | 0.001762818430(10) |
| 2.1 | −0.660066339495(3) | −1.29732526324(3) | 17184.837(5) | 0.010860674168(10) |
| 2.2 | −0.658613227342(3) | −1.27785271948(3) | 16801.908(7) | 0.017897152365(8) |
| 2.3 | −0.656541221424(3) | −1.25949000883(3) | 16426.294(8) | 0.023301058268(5) |
| 2.4 | −0.653996298535(5) | −1.24222281450(2) | 16059.623(9) | 0.027404076072(3) |
| 2.5 | −0.651095080745(3) | −1.22602757356(2) | 15703.193(9) | 0.030465035174(3) |
| 2.6 | −0.647931193414(5) | −1.21087477967(2) | 15358.025(10) | 0.032687541214(3) |
| 2.7 | −0.644580106774(5) | −1.19673127239(2) | 15024.936(8) | 0.034232941168(4) |
| 2.8 | −0.641102856483(3) | −1.18356181693(2) | 14704.56(2) | 0.0352299628710(10) |
| 2.9 | −0.637548926592(5) | −1.17133018410(2) | 14397.424(3) | 0.035781954855(2) |
| 3.0 | −0.633958500603(3) | −1.15999987694(2) | 14103.939(10) | 0.035972374757(2) |
| 3.1 | −0.630364231516(3) | −1.14953460686(2) | 13824.493(4) | 0.035868985863(2) |
| 3.2 | −0.626792642633(3) | −1.13989859276(4) | 13559.395(7) | 0.035527091410(6) |
| 3.3 | −0.623265242795(3) | −1.13105673520(2) | 13308.978(4) | 0.034992045573(2) |
| 3.4 | −0.619799419190(3) | −1.12297470366(2) | 13073.549(9) | 0.034301216094(3) |
| 3.5 | −0.616409155765(2) | −1.11561896398(2) | 12853.473(9) | 0.033485527871(3) |
| 3.6 | −0.613105614109(2) | −1.10895676609(2) | 12649.127(3) | 0.032570683924(3) |
| 3.7 | −0.609897605264(2) | −1.10295610648(2) | 12460.921(9) | 0.031578136229(2) |
| 3.8 | −0.606791974614(2) | −1.09758567601(2) | 12289.368(3) | 0.030525861374(3) |
| 3.9 | −0.6037939171736(4) | −1.09281480077(3) | 12134.982(9) | 0.029428982970(4) |
| 4.0 | −0.6009072369177(4) | −1.08861338155(3) | 11998.403(9) | 0.028300273072(4) |
| 4.1 | −0.598134560958(5) | −1.08495183581(2) | 11880.307(7) | 0.027150557586(2) |
| 4.2 | −0.595477517142(6) | −1.08180104482(2) | 11781.438(9) | 0.025989045111(2) |
| 4.3 | −0.592936881957(8) | −1.07913230780(4) | 11702.624(7) | 0.024823594445(6) |
| 4.4 | −0.590512704231(5) | −1.07691730425(2) | 11644.732(7) | 0.023660932776(2) |
| 4.5 | −0.5882044090772(3) | −1.075128065163(6) | 11608.686(9) | 0.022506834000(2) |
| 4.6 | −0.586010885686(5) | −1.07373695361(3) | 11595.461(3) | 0.021366264730(4) |
| 4.7 | −0.583930561864(5) | −1.07271665528(3) | 11606.014(3) | 0.020243503924(4) |
| 4.8 | −0.581961467746(6) | −1.07204017934(3) | 11641.326(7) | 0.019142240864(2) |
| 4.9 | −0.580101290618(5) | −1.07168087052(2) | 11702.365(5) | 0.018065655247(2) |
| 5.0 | −0.5783474225041(2) | −1.07161243331(2) | 11790.020(7) | 0.01701648233984(8) |

| $2^3\Pi_u$ continued | | | | |
|---|---|---|---|---|
| $R$ | $E$ | $\langle V \rangle$ | $10^6 \cdot \langle \nabla_1 \cdot \nabla_2 \rangle$ | $\mathrm{d}E/\mathrm{d}R$ |
| 5.1 | −0.5766970020(3) | −1.071808970(2) | 11904.9(2) | 0.0159970654(2) |
| 5.2 | −0.575146950730(3) | −1.07224503070(2) | 12048.412(2) | 0.015009398221(4) |
| 5.3 | −0.5736940079(3) | −1.072895688(2) | 12220.2(2) | 0.0140551562(2) |
| 5.4 | −0.5723347590(3) | −1.073736612(2) | 12421.5(2) | 0.0131357234(3) |
| 5.5 | −0.5710656654584(8) | −1.074744182712(5) | 12652.4334(9) | 0.0122522087647(2) |
| 5.6 | −0.5698830916(4) | −1.075895615(3) | 12912.4(2) | 0.0114054585(4) |
| 5.7 | −0.5687833285(4) | −1.077169076(4) | 13201.9(2) | 0.0105960667(4) |
| 5.8 | −0.5677626212(5) | −1.078543853(4) | 13520.3(2) | 0.0098243775(5) |
| 5.9 | −0.5668171927(6) | −1.080000495(5) | 13867.0(2) | 0.0090904898(7) |
| 6.0 | −0.5659432672059(5) | −1.081520967019(5) | 14241.0570(3) | 0.008394261231(2) |
| 6.5 | −0.5625171794935(2) | −1.089563721276(6) | 16454.7661(3) | 0.0054570211863(7) |
| 7.0 | −0.5603514813976(4) | −1.09740673438(5) | 18803.359(7) | 0.003328032631(6) |
| 7.5 | −0.5590726874112(7) | −1.1038588192(2) | 19665.851(6) | 0.00190487409(2) |
| 8.0 | −0.558329991536(3) | −1.10731794567(7) | 17728.1280(2) | 0.001167754676(8) |
| 8.5 | −0.5578334410802(8) | −1.10834942525(2) | 14765.12633(5) | 0.000860877284(2) |
| 9.0 | −0.557445192242(3) | −1.10855139169(5) | 12217.848(3) | 0.000704332533(4) |
| 9.5 | −0.5571221417933(3) | −1.108621328762(4) | 10285.5101(2) | 0.0005918899816(3) |
| 10.0 | −0.5568504344795(4) | −1.108728792292(6) | 8857.6821(2) | 0.0004972076667(4) |
| 11.0 | −0.55575951572416(3) | −1.109081112783(3) | 7055.1736(9) | 0.0003441795112(2) |
| 12.0 | −0.5561478551589(2) | −1.109491690365(2) | 6152.0789(2) | 0.00023366832943(7) |
| 13.0 | −0.5559548564812(4) | −1.109866277174(4) | 5790.69692(4) | 0.0001571873683(2) |
| 14.0 | −0.5558252887067(5) | −1.110175681974(4) | 5772.8904(2) | 0.0001053496742(2) |
| 15.0 | −0.5557385144044(2) | −1.110419311221(2) | 5990.66169(10) | 0.00007051450585(5) |
| 16.0 | −0.55568044084928(10) | −1.1106057930895(7) | 6393.39937(8) | 0.00004719303807(2) |
| 17.0 | −0.5556415610819(2) | −1.1107456970544(6) | 6970.89257(2) | 0.000031613241735(5) |
| 18.0 | −0.55561549531781(8) | −1.1108490692914(4) | 7742.87643(6) | 0.0000212178524592(8(7) |
| 19.0 | −0.55559797845052(8) | −1.1109246018733(3) | 8747.82147(9) | 0.000014281843561(3) |
| 20.0 | −0.55558616842347(5) | −1.11097937283242(7) | 10019.95581(10) | 0.000009648200715(7) |

TABLE S15. Calculated BO energies, expectation value of potential, $\langle\nabla_1\cdot\nabla_2\rangle$, and $\mathrm{d}E/\mathrm{d}R$ of the $3^3\Pi_u$ state in atomic units (hartree). Uncertainties originate purely from extrapolation to the complete basis set limit. United atom values at $R=0$ are taken from Ref. [1].

| $3^3\Pi_\mathrm{u}$ | | | | |
|---|---|---|---|---|
| $R$ | $E$ | $\langle V\rangle$ | $10^6\cdot\langle\nabla_1\cdot\nabla_2\rangle$ | $\mathrm{d}E/\mathrm{d}R$ |
| 0.0 | −2.03106965045024(3) | – | 7555.17898(1) | – |
| 0.01 | 97.96793674552(8) | 95.9363904275(5) | 7555.99(2) | −9999.94830635(3) |
| 0.05 | 17.973693112(8) | 15.95880640(5) | 7575.14(10) | −399.7715965(7) |
| 0.1 | 7.989412601(3) | 6.01789097(2) | 7625.3(4) | −99.6093424(2) |
| 0.15 | 4.678578887(4) | 2.76579601(3) | 7695.50(8) | −43.9424117(2) |
| 0.2 | 3.038989001(3) | 1.19311713(2) | 7774.85(7) | −24.42430437(5) |
| 0.3 | 1.43418496(3) | −0.2704585(3) | 7937.72(3) | −10.4627612(8) |
| 0.4 | 0.6667482922(4) | −0.901357764(3) | 8081.459(9) | −5.587135871(5) |
| 0.5 | 0.23246596(2) | −1.21097412(7) | 8187.7(6) | −3.35181209(8) |
| 0.6 | −0.03740485663(8) | −1.3697395064(6) | 8252.89(2) | −2.1582163219(7) |
| 0.7 | −0.215243361937(5) | −1.4495420539(3) | 8274.00(2) | −1.4557933285(3) |
| 0.8 | −0.337120612874(7) | −1.48519391168(5) | 8254.68(3) | −1.01369085741(5) |
| 0.9 | −0.422923118196(5) | −1.49514745837(5) | 8199.43(4) | −0.72144580220(4) |
| 1.0 | −0.484441351024(6) | −1.48982163393(4) | 8113.53(4) | −0.52093893188(3) |
| 1.1 | −0.529060007460(6) | −1.47537617796(4) | 8002.32(5) | −0.37932378458(3) |
| 1.2 | −0.561607002378(2) | −1.45557883354(4) | 7870.89(5) | −0.27697069064(2) |
| 1.3 | −0.585349294188(8) | −1.43279264146(4) | 7723.83(6) | −0.20161081006(2) |
| 1.4 | −0.602560915761(8) | −1.40852601416(4) | 7565.20(6) | −0.14528870189(2) |
| 1.5 | −0.614862506795(9) | −1.38375241545(4) | 7398.50(7) | −0.102684934569(9) |
| 1.6 | −0.623432308595(10) | −1.35910269664(3) | 7226.62(7) | −0.070148799656(6) |
| 1.7 | −0.62914165701(2) | −1.33498420529(3) | 7052.02(7) | −0.045118171335(3) |
| 1.8 | −0.63264446963(2) | −1.31165635723(4) | 6876.64(8) | −0.025759676653(7) |
| 1.9 | −0.63443780313(2) | −1.28927957766(3) | 6702.22(8) | −0.010738932319(2) |
| 2.0 | −0.63490371402(2) | −1.26794754871(2) | 6529.92(8) | 0.000929939656(5) |
| 2.1 | −0.63433874277(2) | −1.24770876810(2) | 6360.83(9) | 0.009985103532(6) |
| 2.2 | −0.63297502942(2) | −1.22858113806(2) | 6195.75(9) | 0.016985873064(8) |
| 2.3 | −0.63099566281(2) | −1.210561939709(8) | 6035.30(9) | 0.022360602552(9) |
| 2.4 | −0.62854598908(2) | −1.19363472384(4) | 5879.89(10) | 0.026440522632(2) |
| 2.5 | −0.62574204649(2) | −1.177774171737(5) | 5730.17(9) | 0.029483968477(10) |
| 2.6 | −0.62267693381(2) | −1.162949886186(7) | 5585.75(9) | 0.031693838997(9) |
| 2.7 | −0.61942570996(2) | −1.14913183653(2) | 5443.78(9) | 0.033229475329(4) |
| 2.8 | −0.61604970837(2) | −1.1363448521(4) | 5240.3(2) | 0.03419805881(10) |
| 2.9 | −0.6126373276449(9) | −1.1273877072(6) | 1025.496(8) | 0.0337541200(3) |
| 3.0 | −0.6092565809066(3) | −1.1169704761(2) | 686.8614(6) | 0.03384756185(6) |
| 3.1 | −0.6058760067337(2) | −1.107215086305(6) | 728.1328(2) | 0.033721589406(3) |
| 3.2 | −0.6025200367719(2) | −1.098279992182(2) | 804.50572(7) | 0.033362525425(2) |
| 3.3 | −0.5992098882292(2) | −1.090141364550(6) | 899.20881(2) | 0.0328116399726(8) |
| 3.4 | −0.59596291148758(9) | −1.08277065421(2) | 1010.58055(3) | 0.032104461401(3) |
| 3.5 | −0.59279322541713(7) | −1.076140686200(10) | 1139.96220(3) | 0.031270218466(3) |
| 3.6 | −0.58971230473326(7) | −1.070226837631(5) | 1289.98488(2) | 0.0303327143988(10) |
| 3.7 | −0.58672948045000(7) | −1.065007739046(6) | 1464.27461(6) | 0.029311141042(2) |
| 3.8 | −0.58385236783512(7) | −1.0604660320200(4) | 1667.510(2) | 0.028220711486(2) |
| 3.9 | −0.58108724022858(7) | −1.056589342884(5) | 1905.53(4) | 0.027073112197(2) |
| 4.0 | −0.57843936615047(9) | −1.05337158460(2) | 2186.20482(9) | 0.025876786926(4) |
| 4.1 | −0.575913326058(2) | −1.05081470268(3) | 2518.7772(8) | 0.024637060838(6) |
| 4.2 | −0.573513324467(2) | −1.04893098751(3) | 2915.543(2) | 0.023356109864(6) |
| 4.3 | −0.571243512561(7) | −1.0477460526(2) | 3391.7(2) | 0.02203278429(6) |
| 4.4 | −0.569108334546(3) | −1.04730246712(6) | 3967.671(3) | 0.02066231863(2) |
| 4.5 | −0.5671129053971(4) | −1.04766372527(6) | 4666.929(3) | 0.01923601901(2) |
| 4.6 | −0.565263411923(5) | −1.0489174690(2) | 5519.01(6) | 0.01774116408(3) |
| 4.7 | −0.563567493774(7) | −1.0511753560(2) | 6557.4919(2) | 0.01616162374(4) |
| 4.8 | −0.56203448904(2) | −1.0545642493(5) | 7815.4358(6) | 0.01448015183(9) |
| 4.9 | −0.56067530774(2) | −1.0591999694(3) | 9317.460(2) | 0.01268380532(6) |
| 5.0 | −0.559501546185(2) | −1.0651338718(3) | 11063.43(2) | 0.01077384411(4) |

| $3^3\Pi_u$ continued | | | | |
|---|---|---|---|---|
| $R$ | $E$ | $\langle V\rangle$ | $10^6\cdot\langle\nabla_1\cdot\nabla_2\rangle$ | $\mathrm{d}E/\mathrm{d}R$ |
| 5.1 | −0.55852340305(3) | −1.0722723195(2) | 13007.53(7) | 0.00877931109(5) |
| 5.2 | −0.55774628400(3) | −1.08029864685(10) | 15042.66(6) | 0.00676806175(3) |
| 5.3 | −0.55716691445(3) | −1.088663240174(10) | 17006.75(5) | 0.004843507293(10) |
| 5.4 | −0.55677086362(3) | −1.09669587688(9) | 18722.96(4) | 0.003119601917(9) |
| 5.5 | −0.556533310016(2) | −1.10380226580(3) | 20054.675(10) | 0.001684428042(3) |
| 5.6 | −0.55642303456(3) | −1.1096214112(3) | 20940.17(3) | 0.00057583178(4) |
| 5.7 | −0.55640761437(3) | −1.1140575306(4) | 21390.23(2) | −0.00021794769(5) |
| 5.8 | −0.55645756958(4) | −1.1172097784(5) | 21460.84(2) | −0.00074045504(6) |
| 5.9 | −0.55654851161(4) | −1.1192746870(5) | 21224.60(2) | −0.00104706166(7) |
| 6.0 | −0.5566615832277(4) | −1.120471693419(5) | 20751.9800(10) | −0.0011914211605(5) |
| 6.5 | −0.5571976881284(5) | −1.119337563057(6) | 16549.4090(4) | −0.0007603364306(6) |
| 7.0 | −0.5573678766096(5) | −1.114291796186(5) | 11685.406468(10) | 0.0000634224333(3) |
| 7.5 | −0.5571787286781(3) | −1.1096549596025(5) | 8572.7378(2) | 0.0006269997002(2) |
| 8.0 | −0.5568167473350(2) | −1.1076182605094(10) | 8607.9430(6) | 0.0007519042699(3) |
| 8.5 | −0.5564710224949(2) | −1.107746149547(5) | 9977.6354(5) | 0.0006112818163(9) |
| 9.0 | −0.55621022322396(10) | −1.1084979781440(10) | 11194.4591(7) | 0.0004358298114(2) |
| 9.5 | −0.5560284445625(4) | −1.109217355762(3) | 12019.8866(7) | 0.0002988982484(5) |
| 10.0 | −0.55590423140963(5) | −1.1097665061842(6) | 12531.0757(7) | 0.00020419566346(9) |
| 11.0 | −0.55575951572416(3) | −1.1104239175269(3) | 12959.4769(2) | 0.00009955581098(6) |
| 12.0 | −0.55568609559565(2) | −1.1107324734532(3) | 12948.9260(4) | 0.00005330981150(3) |
| 13.0 | −0.55564496618165(2) | −1.1108806943325(5) | 12715.79383(3) | 0.00003147984851(5) |
| 14.0 | −0.555619726267830(10) | −1.1109576365463(2) | 12355.235372(3) | 0.00002012971352(2) |
| 15.0 | −0.555603120814325(8) | −1.11100171972292(5) | 11902.07027(8) | 0.000013634793710(7) |
| 16.0 | −0.555591642141235(10) | −1.11102932956862(3) | 11356.2501(3) | 0.000009622169611(4) |
| 17.0 | −0.555583416701015(2) | −1.11104774440(3) | 10693.864(6) | 0.000007005231(3) |
| 18.0 | −0.55557735193609(2) | −1.1110604726(2) | 9872.84(2) | 0.000005235066(2) |
| 19.0 | −0.55557276709809(2) | −1.1110693993(4) | 8840.42(6) | 0.000004007098(4) |
| 20.0 | −0.55556921894044(2) | −1.1110756876(9) | 7553.4(2) | 0.00000313751(2) |

TABLE S16. Calculated BO energies, expectation value of potential, $\langle\nabla_1\cdot\nabla_2\rangle$, and $\mathrm{d}E/\mathrm{d}R$ of the $4^3\Pi_u$ state in atomic units (hartree). Uncertainties originate purely from extrapolation to the complete basis set limit. United atom values at $R=0$ are taken from Ref. [1].

| $4^3\Pi_\mathrm{u}$ | | | | |
|---|---|---|---|---|
| $R$ | $E$ | $\langle V\rangle$ | $10^6\cdot\langle\nabla_1\cdot\nabla_2\rangle$ | $\mathrm{d}E/\mathrm{d}R$ |
| 0.0 | −2.031255144381749(1) | – | 9.6696396 | – |
| 0.01 | 97.96900618942(5) | 95.9385298243(3) | 9.671(3) | −9999.94825545(2) |
| 0.05 | 17.974768101(3) | 15.96096723(2) | 9.797(5) | −399.7713795(2) |
| 0.1 | 7.990502264(5) | 6.02010620(3) | 10.160(6) | −99.6089833(2) |
| 0.15 | 4.679688825(7) | 2.76808275(5) | 10.722(4) | −43.9419660(3) |
| 0.2 | 3.040122589(3) | 1.19548329(2) | 11.463(4) | −24.42380941(5) |
| 0.3 | 1.4353698795(4) | −0.267933132(2) | 11.3(5) | −10.462242970(2) |
| 0.4 | 0.667983504(2) | −0.898695376(10) | 15.8(3) | −5.58665596(2) |
| 0.5 | 0.23374572287(9) | −1.2082112364(8) | 19.16(7) | −3.351405364(2) |
| 0.6 | −0.03608894287(4) | −1.3669192657(3) | 23.04(8) | −2.1579022999(4) |
| 0.7 | −0.213901128076(6) | −1.44670967544(5) | 27.69(4) | −1.45558202755(5) |
| 0.8 | −0.335762565642(3) | −1.48239404759(3) | 33.02(2) | −1.01358614538(3) |
| 0.9 | −0.4215599335484(10) | −1.49242259240(3) | 39.133(9) | −0.72144747256(2) |
| 1.0 | −0.4830835402668(2) | −1.48721116854(2) | 46.099(7) | −0.52104408800(2) |
| 1.1 | −0.5277176991384(6) | −1.47291598011(2) | 53.994(6) | −0.37952780167(2) |
| 1.2 | −0.5602898055072(3) | −1.45330108893(2) | 62.904(5) | −0.277267898262(9) |
| 1.3 | −0.5840662193884(8) | −1.43072591192(2) | 72.922(5) | −0.201994979341(8) |
| 1.4 | −0.6013203377653(5) | −1.40669542353(2) | 84.154(5) | −0.145753391430(7) |
| 1.5 | −0.61367215601928(8) | −1.382179911621(8) | 96.719(5) | −0.103223733054(4) |
| 1.6 | −0.62229928302782(7) | −1.357807353976(5) | 110.751(5) | −0.070755492449(2) |
| 1.7 | −0.62807244783221(4) | −1.333982543620(4) | 126.399(5) | −0.045786851738(2) |
| 1.8 | −0.63164499585127(5) | −1.310962662578(5) | 143.839676(3) | −0.026484817153(3) |
| 1.9 | −0.63351345185437(10) | −1.288906215923(5) | 163.25155(9) | −0.011515427481(3) |
| 2.0 | −0.63405938392257(5) | −1.267905267247(4) | 184.848(6) | 0.000106750299(2) |
| 2.1 | −0.63357888915233(7) | −1.248006982407(6) | 208.887(8) | 0.009119426618(2) |
| 2.2 | −0.63230370955222(4) | −1.229228198672(5) | 235.640(5) | 0.016081463833(2) |
| 2.3 | −0.6304165804424(5) | −1.211565366088(5) | 265.41421(2) | 0.021420780347(2) |
| 2.4 | −0.6280625362610(7) | −1.195001360578(2) | 298.553(5) | 0.025468213309(4) |
| 2.5 | −0.62535733780281(10) | −1.179510101449(10) | 335.5333(7) | 0.028481829663(4) |
| 2.6 | −0.6223938153247(3) | −1.16505933598(2) | 377.18558(2) | 0.030664728719(7) |
| 2.7 | −0.6192466480779(8) | −1.15160975853(6) | 427.27644(4) | 0.03217908801(2) |
| 2.8 | −0.6159754877121(7) | −1.1390636818(5) | 550.437(2) | 0.0331740335(2) |
| 2.9 | −0.61258993159(2) | −1.1245481385(3) | 4697.85(10) | 0.0347005946(2) |
| 3.0 | −0.60910147533(2) | −1.113279029676(5) | 4982.86(8) | 0.034974640313(10) |
| 3.1 | −0.60560614404(2) | −1.10306161859(3) | 4902.78(10) | 0.034887312724(6) |
| 3.2 | −0.60213193105(2) | −1.093666570131(6) | 4804.30(9) | 0.034561653684(8) |
| 3.3 | −0.59870014421(2) | −1.085049290070(8) | 4705.82(7) | 0.034045757009(8) |
| 3.4 | −0.59532785642(2) | −1.07717277441(4) | 4610.73(3) | 0.033377334831(4) |
| 3.5 | −0.59202872508(2) | −1.07000189273(2) | 4521.28(10) | 0.032587302068(5) |
| 3.6 | −0.58881359131(2) | −1.06350261764(2) | 4437.34(10) | 0.031701268030(8) |
| 3.7 | −0.585690956612(10) | −1.05764182627(3) | 4359.77(4) | 0.030740564043(2) |
| 3.8 | −0.58266736954(2) | −1.05238720974(5) | 4288.42(3) | 0.029723034037(7) |
| 3.9 | −0.57974774201(2) | −1.04770721178(6) | 4223.78(3) | 0.02866365952(2) |
| 4.0 | −0.57693560962(2) | −1.04357097927(4) | 4166.00(9) | 0.027575059986(4) |
| 4.1 | −0.57423334705(2) | −1.039948325815(9) | 4115.90(6) | 0.026467894695(8) |
| 4.2 | −0.57164234718(3) | −1.03680970154(3) | 4073.41(7) | 0.025351188818(7) |
| 4.3 | −0.56916317088(2) | −1.034126175118(10) | 4039.15(6) | 0.02423259692(2) |
| 4.4 | −0.56679567295(2) | −1.031869427504(2) | 4013.54(6) | 0.023118617849(8) |
| 4.5 | −0.56453910868(2) | −1.03001175342(3) | 3997.13(3) | 0.022014769813(6) |
| 4.6 | −0.562392224448(10) | −1.02852607261(3) | 3990.28(6) | 0.020925733966(9) |
| 4.7 | −0.56035333538(3) | −1.02738594937(5) | 3993.855(9) | 0.01985547268(3) |
| 4.8 | −0.55842039212(3) | −1.02656561414(6) | 4008.18(2) | 0.01880732715(3) |
| 4.9 | −0.556591038834(10) | −1.02603999172(4) | 4033.86(6) | 0.01778409916(2) |
| 5.0 | −0.55486266354(2) | −1.02578472765(4) | 4071.56(8) | 0.01678811985(2) |

| $4^3\Pi_u$ continued | | | | |
|---|---|---|---|---|
| $R$ | $E$ | $\langle V \rangle$ | $10^6 \cdot \langle \nabla_1 \cdot \nabla_2 \rangle$ | $\mathrm{d}E/\mathrm{d}R$ |
| 5.1 | −0.553232443(2) | −1.02577623(2) | 4121.5(2) | 0.015821306(4) |
| 5.2 | −0.551697379(2) | −1.02599161(3) | 4184.7(2) | 0.014885221(4) |
| 5.3 | −0.550254333(2) | −1.02640881(3) | 4261.2(2) | 0.013981106(5) |
| 5.4 | −0.548900059(3) | −1.02700650(4) | 4350.9(2) | 0.013109929(6) |
| 5.5 | −0.547631222148(4) | −1.02776409927(6) | 4454.34(5) | 0.01227242636(2) |
| 5.6 | −0.546444435(4) | −1.02866185(5) | 4569.4(2) | 0.011469110(8) |
| 5.8 | −0.544303204(5) | −1.03080147(8) | 4834.2(3) | 0.00996637(2) |
| 5.9 | −0.543341814(6) | −1.03200686(9) | 4980.2(3) | 0.00926725(2) |
| 6.0 | −0.542448585689(4) | −1.03327914821(6) | 5132.72(5) | 0.00860300386(2) |
| 6.5 | −0.538883842724(2) | −1.04008265029(3) | 5870.88(2) | 0.005797697717(4) |
| 7.0 | −0.536515978508(2) | −1.04644266100(8) | 6302.00(2) | 0.003798470860(9) |
| 7.5 | −0.534974925145(4) | −1.051494656893(10) | 6284.01(7) | 0.002460692450(3) |
| 8.0 | −0.533975596442(6) | −1.05513476482(5) | 5891.01(9) | 0.00160205350(2) |
| 8.5 | −0.533319775267(6) | −1.05760097659(6) | 5267.96(10) | 0.00106336163(2) |
| 9.0 | −0.532879029864(5) | −1.05923111522(4) | 4571.03(9) | 0.000725216051(8) |
| 9.5 | −0.532574738980(6) | −1.06033221777(6) | 3916.99(10) | 0.000507080014(9) |
| 10.0 | −0.532360127292(5) | −1.06111408116(5) | 3363.90(9) | 0.000360617338(8) |
| 11.0 | −0.532095168365(4) | −1.06209449800(5) | 2584.14(8) | 0.000190530790(6) |
| 12.0 | −0.531947810466(4) | −1.06251299724(4) | 2116.25(7) | 0.000115218638(5) |
| 13.0 | −0.531849836075(3) | −1.06259045015(3) | 1806.79(6) | 0.000085324767(4) |
| 14.0 | −0.531771562618(3) | −1.06252417142(3) | 1573.12(5) | 0.000072782414(3) |
| 15.0 | −0.531702494600(3) | −1.06241794050(3) | 1382.06(4) | 0.000065803245(3) |
| 16.0 | −0.531639507384(3) | −1.06231496805(3) | 1221.38(4) | 0.000060252918(3) |
| 17.0 | −0.531581960211(2) | −1.06223201796(4) | 1086.69(4) | 0.000054817791(3) |
| 18.0 | −0.531529939877(2) | −1.06217447078(4) | 976.26(3) | 0.000049189387(3) |
| 19.0 | −0.531483627425(2) | −1.06214214987(4) | 889.02(3) | 0.000043426577(3) |
| 20.0 | −0.531443071566(2) | −1.06213195421(4) | 823.67(3) | 0.000037709445(3) |

TABLE S17. Calculated BO energies, expectation value of potential, $\langle \nabla_1 \cdot \nabla_2 \rangle$, and $\mathrm{d}E/\mathrm{d}R$ of the $1^1\Delta_g$ state in atomic units (hartree). Uncertainties originate purely from extrapolation to the complete basis set limit. United atom values at $R = 0$ are taken from Ref. [1].

| $1^1\Delta_g$ | | | | |
|---|---|---|---|---|
| $R$ | $E$ | $\langle V \rangle$ | $10^6 \cdot \langle \nabla_1 \cdot \nabla_2 \rangle$ | $\mathrm{d}E/\mathrm{d}R$ |
| 0.0 | −2.055620732852246(6) | – | 249.3999921(1) | – |
| 0.01 | 97.94464063225(8) | 95.8897987253(4) | 249.495(5) | −9999.94825392(3) |
| 0.05 | 17.950402758(2) | 15.91223701(2) | 251.715(2) | −399.7713702(3) |
| 0.1 | 7.966137799(2) | 5.971379772(8) | 257.7675(3) | −99.60895827(6) |
| 0.15 | 4.655326122(10) | 2.71936403(9) | 266.582(4) | −43.9419215(5) |
| 0.2 | 3.0157626470(4) | 1.146776579(3) | 277.4901(10) | −24.42374358(2) |
| 0.3 | 1.4110187858(2) | −0.316601808(2) | 303.983(2) | −10.462131266(4) |
| 0.4 | 0.64364598011(10) | −0.9473064696(9) | 334.9933(8) | −5.586496075(2) |
| 0.5 | 0.20942662468(5) | −1.2567450891(5) | 369.2268(7) | −3.3511966770(9) |
| 0.6 | −0.06038473758(7) | −1.4153564736(8) | 405.8327(4) | −2.157644997(2) |
| 0.7 | −0.238168788667(6) | −1.4950313299(3) | 444.1652(7) | −1.4552767894(4) |
| 0.8 | −0.359997345352(5) | −1.5305818482(3) | 483.6862(6) | −1.0132339469(3) |
| 0.9 | −0.445757193490(3) | −1.5404589218(3) | 523.9099(3) | −0.7210494831(2) |
| 1.0 | −0.507238765568(2) | −1.5350791419(2) | 564.38021(3) | −0.5206016107(2) |
| 1.1 | −0.551826510264(2) | −1.5205994788(2) | 604.65916(9) | −0.3790422348(2) |
| 1.2 | −0.584347966331(2) | −1.5007847822(2) | 644.3213(2) | −0.2767407079(2) |
| 1.3 | −0.608069642915(2) | −1.4779952685(2) | 682.9511(2) | −0.20142767898(10) |
| 1.4 | −0.625265089996(2) | −1.4537367149(2) | 720.1432(3) | −0.14514752492(9) |
| 1.5 | −0.637554458244(2) | −1.4289802064(2) | 755.50399(9) | −0.10258085994(8) |
| 1.6 | −0.646115512699(2) | −1.4043545041(2) | 788.6509(10) | −0.07007717418(7) |
| 1.7 | −0.651819138081(2) | −1.3802651611(2) | 819.2249(3) | −0.04507463820(6) |
| 1.8 | −0.655318833653(2) | −1.3569700867(2) | 846.8729(2) | −0.02574023302(6) |
| 1.9 | −0.6571112747985(9) | −1.3346284697(2) | 871.2699(2) | −0.01073995792(5) |
| 2.0 | −0.657578175515(2) | −1.3133330016(2) | 892.1116(2) | 0.00091167472(5) |
| 2.1 | −0.6570157725599(9) | −1.2931314085(2) | 909.118451(5) | 0.00995244599(5) |
| 2.2 | −0.655655939719(2) | −1.2740410080(2) | 922.0376(2) | 0.01694130518(4) |
| 2.3 | −0.6536815346421(8) | −1.2560586436(2) | 930.6464(2) | 0.02230627202(4) |
| 2.4 | −0.651237703586(2) | −1.2391675119(2) | 934.75261(10) | 0.02637828968(4) |
| 2.5 | −0.648440309661(2) | −1.22334187472(10) | 934.1976(2) | 0.02941549784(4) |
| 2.6 | −0.645382285520(2) | −1.20855031659(10) | 928.8582(2) | 0.03162086710(4) |
| 2.7 | −0.642138469418(2) | −1.19475799353(2) | 918.6476(2) | 0.03315516493(4) |
| 2.8 | −0.6387693202308(8) | −1.1819281760(2) | 903.5176(2) | 0.03414659445(4) |
| 2.9 | −0.635323795042(2) | −1.1700232967(2) | 883.4601(2) | 0.03469803220(3) |
| 3.0 | −0.6318415950686(8) | −1.1590056488(2) | 858.5083(2) | 0.03489251378(3) |
| 3.1 | −0.628354930861(2) | −1.1488378379(2) | 828.7376(2) | 0.03479742705(3) |
| 3.2 | −0.624889918637(2) | −1.1394830604(2) | 794.2667(2) | 0.03446774277(3) |
| 3.3 | −0.621467691419(2) | −1.1309052612(2) | 755.2582(2) | 0.03394852171(3) |
| 3.4 | −0.6181052881259(8) | −1.1230692072(2) | 711.91896(9) | 0.03327687324(3) |
| 3.5 | −0.614816368695(2) | −1.1159405055(2) | 664.4998(2) | 0.03248349484(3) |
| 3.6 | −0.611611792070(2) | −1.1094855841(2) | 613.2956(2) | 0.03159388889(3) |
| 3.7 | −0.608500085550(2) | −1.1036716527(2) | 558.6440(2) | 0.03062932930(3) |
| 3.8 | −0.605487827630(2) | −1.0984666501(2) | 500.9243(2) | 0.02960763294(3) |
| 3.9 | −0.602579961668(2) | −1.0938391903(2) | 440.5554(2) | 0.02854377771(3) |
| 4.0 | −0.599780054032(2) | −1.0897585092(2) | 377.9932(2) | 0.02745039972(4) |
| 4.1 | −0.59709050752(2) | −1.0861944183(2) | 313.7279(2) | 0.02633819432(4) |
| 4.2 | −0.59451273861(2) | −1.0831172663(2) | 248.2795(2) | 0.02521624070(4) |
| 4.3 | −0.59204732551(2) | −1.0804979108(2) | 182.1937(2) | 0.02409226517(4) |
| 4.4 | −0.58969413232(2) | −1.0783077013(2) | 116.0364(2) | 0.02297285531(4) |
| 4.5 | −0.587452413905(2) | −1.0765184726(2) | 50.3879(2) | 0.02186363450(4) |
| 4.6 | −0.58532090495(2) | −1.0751025488(2) | −14.1644(2) | 0.02076940458(4) |
| 4.7 | −0.58329789605(2) | −1.0740327578(2) | −77.0331(2) | 0.01969426262(4) |
| 4.8 | −0.58138129929(2) | −1.0732824534(2) | −137.6389(2) | 0.01864169692(3) |
| 4.9 | −0.57956870499(2) | −1.0728255467(2) | −195.4192(2) | 0.01761466598(3) |
| 5.0 | −0.5778574313451(9) | −1.07263654358(4) | −249.8371(2) | 0.016615663821(6) |

| $1^1\Delta_g$ continued | | | | |
|---|---|---|---|---|
| $R$ | $E$ | $\langle V\rangle$ | $10^6\cdot\langle\nabla_1\cdot\nabla_2\rangle$ | $\mathrm{d}E/\mathrm{d}R$ |
| 5.1 | −0.57624456807(2) | −1.0726905879(2) | −300.39034(6) | 0.01564677417(3) |
| 5.2 | −0.57472701512(2) | −1.0729635094(2) | −346.62071(6) | 0.01470971554(3) |
| 5.3 | −0.57330151724(2) | −1.0734318762(2) | −388.12233(6) | 0.01380587891(3) |
| 5.4 | −0.57196469513(2) | −1.0740730496(2) | −424.55003(6) | 0.01293635939(2) |
| 5.5 | −0.5707130736461(10) | −1.0748652412(2) | −455.62660(7) | 0.01210198292(3) |
| 5.6 | −0.56954310754(2) | −1.0757875721(2) | −481.14855(5) | 0.01130332911(2) |
| 5.7 | −0.56845120509(2) | −1.0768201322(2) | −500.99099(5) | 0.01054075052(2) |
| 5.8 | −0.56743374995(2) | −1.07794403860(10) | −515.10989(5) | 0.00981438988(2) |
| 5.9 | −0.56648712138(2) | −1.07914149229(10) | −523.54296(4) | 0.00912419500(2) |
| 6.0 | −0.5656077130156(8) | −1.0803958311(2) | −526.40821(6) | 0.00846993250(2) |
| 6.5 | −0.5620958545227(7) | −1.08702241688(2) | −466.342356(8) | 0.005718352641(3) |
| 7.0 | −0.5597588069529(6) | −1.09327995541(2) | −319.624503(7) | 0.003748236927(2) |
| 7.5 | −0.5582430041811(6) | −1.09844500090(2) | −143.919569(6) | 0.002405467662(2) |
| 8.0 | −0.5572765084694(5) | −1.10235713531(7) | 16.25444(4) | 0.001524485205(7) |
| 8.5 | −0.5566657784146(4) | −1.10516157937(5) | 139.17337(3) | 0.000961173819(5) |
| 9.0 | −0.5562807673480(4) | −1.10710387325(5) | 221.20754(3) | 0.000606406828(4) |
| 9.5 | −0.5560373516877(3) | −1.10842077012(4) | 268.18138(2) | 0.000384624554(3) |
| 10.0 | −0.5558823395249(3) | −1.10930212830(3) | 288.86959(2) | 0.000246255076(2) |
| 11.0 | −0.5557172626635(2) | −1.11027501915(2) | 283.074177(10) | 0.0001054096526(8) |
| 12.0 | −0.5556442468329(2) | −1.11070175639(2) | 249.94157(2) | 0.0000488947732(7) |
| 13.0 | −0.55560891584507(8) | −1.11089271310(2) | 211.74911(2) | 0.0000250091226(6) |
| 14.0 | −0.55559002375800(7) | −1.110982666208(10) | 176.94278(2) | 0.0000140986650(3) |
| 15.0 | −0.55557895352912(6) | −1.111028620149(9) | 147.72163(2) | 0.0000086191274(2) |
| 16.0 | −0.55557198533841(5) | −1.111054497715(4) | 123.921656(7) | 0.00000559206019(3) |
| 17.0 | −0.55556737127515(3) | −1.111070483806(2) | 104.691749(8) | 0.00000377992608(6) |
| 18.0 | −0.55556420810772(2) | −1.1110811031163(5) | 89.121911(6) | 0.00000262850542(7) |
| 19.0 | −0.55556198592162(2) | −1.1110885180730(4) | 76.434402(4) | 0.0000018659878(2) |
| 20.0 | −0.555560395819745(10) | −1.1110938651653(7) | 66.013132(3) | 0.00000134632363(9) |

TABLE S18. Calculated BO energies, expectation value of potential, $\langle\nabla_1 \cdot \nabla_2\rangle$, and $\mathrm{d}E/\mathrm{d}R$ of the $2^1\Delta_g$ state in atomic units (hartree). Uncertainties originate purely from extrapolation to the complete basis set limit. United atom values at $R = 0$ are taken from Ref. [1].

| $2^1\Delta_\mathrm{g}$ | | | | |
|---|---|---|---|---|
| $R$ | $E$ | $\langle V\rangle$ | $10^6 \cdot \langle\nabla_1 \cdot \nabla_2\rangle$ | $\mathrm{d}E/\mathrm{d}R$ |
| 0.0 | −2.031279846178687(7) | – | 129.1751887(8) | – |
| 0.01 | 97.9689815171(6) | 95.938480492(7) | 129.1(2) | −9999.9482542(6) |
| 0.05 | 17.974743568(4) | 15.96091845(3) | 130.27(9) | −399.7713737(5) |
| 0.1 | 7.990478260(5) | 6.02005964(4) | 133.49(10) | −99.6089688(3) |
| 0.15 | 4.679665835(4) | 2.76804054(3) | 138.20(10) | −43.9419408(2) |
| 0.2 | 3.040101130(3) | 1.19544761(3) | 144.05(10) | −24.42377326(9) |
| 0.3 | 1.435353191(2) | −0.26794865(2) | 158.34(9) | −10.46218345(4) |
| 0.4 | 0.667973981(2) | −0.89868087(2) | 175.20(9) | −5.58657208(3) |
| 0.5 | 0.233745815(3) | −1.20815680(3) | 194.058(5) | −3.35129687(5) |
| 0.6 | −0.036076769(3) | −1.36681506(3) | 214.249(5) | −2.15776921(4) |
| 0.7 | −0.2138744247(7) | −1.446546050(7) | 235.6(5) | −1.455424573(9) |
| 0.8 | −0.3357189126(6) | −1.482161560(7) | 257.7(2) | −1.013404669(7) |
| 0.9 | −0.4214969484(5) | −1.492112037(6) | 280.31(7) | −0.721242378(6) |
| 1.0 | −0.4829988831(5) | −1.486813583(6) | 303.37(7) | −0.520815817(5) |
| 1.1 | −0.5276090751(4) | −1.472422645(5) | 326.53(6) | −0.379276813(4) |
| 1.2 | −0.5601549662(4) | −1.452703523(5) | 349.58(6) | −0.276994659(4) |
| 1.3 | −0.5839029627(4) | −1.430015856(5) | 372.29(5) | −0.201699947(3) |
| 1.4 | −0.6011265066(3) | −1.405864824(4) | 394.44(5) | −0.145437007(3) |
| 1.5 | −0.6134456363(3) | −1.381220891(4) | 415.83(4) | −0.102886412(3) |
| 1.6 | −0.6220380003(3) | −1.356712180(4) | 436.23(4) | −0.070397612(2) |
| 1.7 | −0.6277743631(2) | −1.332743588(4) | 455.47(3) | −0.045408742(2) |
| 1.8 | −0.6313081002(2) | −1.309572348(4) | 473.35(3) | −0.026086749(2) |
| 1.9 | −0.6331357600(2) | −1.287356959(4) | 489.68(3) | −0.011097600(2) |
| 2.0 | −0.6336389265(2) | −1.266189406(4) | 504.31(2) | 0.000544224(2) |
| 2.1 | −0.6331137032(2) | −1.246116692(4) | 516.63(10) | 0.009576531(2) |
| 2.2 | −0.6317918279(2) | −1.227155397(4) | 527.4(2) | 0.016558299(2) |
| 2.3 | −0.6298560197(2) | −1.209301614(4) | 535.9(2) | 0.021917576(2) |
| 2.4 | −0.6274512833(2) | −1.192537773(4) | 542.2(2) | 0.025985331(2) |
| 2.5 | −0.62469333803(10) | −1.176837358(4) | 546.1(2) | 0.029019727(2) |
| 2.6 | −0.62167497012(10) | −1.162168163(4) | 547.6(2) | 0.031223761(2) |
| 2.7 | −0.61847086911(9) | −1.148494542(4) | 546.5(2) | 0.032758221(2) |
| 2.8 | −0.61514134299(8) | −1.135778956(4) | 542.9(2) | 0.0337513320(10) |
| 2.9 | −0.61173519588(8) | −1.123983019(4) | 536.6(2) | 0.0343059907(10) |
| 3.0 | −0.60829197421(7) | −1.113068200(4) | 527.7(2) | 0.0345052495(10) |
| 3.1 | −0.60484373213(7) | −1.102996279(4) | 516.1(2) | 0.0344165114(10) |
| 3.2 | −0.60141642811(7) | −1.093729629(4) | 502.0(2) | 0.0340947587(10) |
| 3.3 | −0.59803103643(6) | −1.085231374(4) | 485.2(2) | 0.0335850603(9) |
| 3.4 | −0.59470443667(6) | −1.077465474(4) | 466.1(2) | 0.0329245293(9) |
| 3.5 | −0.59145012934(6) | −1.070396743(4) | 444.6(2) | 0.0321438617(9) |
| 3.6 | −0.58827881435(5) | −1.063990841(4) | 420.7(2) | 0.0312685523(9) |
| 3.7 | −0.58519886109(5) | −1.058214239(4) | 394.6(2) | 0.0303198605(9) |
| 3.8 | −0.58221669200(5) | −1.053034178(4) | 366.5(3) | 0.0293155805(8) |
| 3.9 | −0.57933709708(5) | −1.048418626(5) | 336.9(2) | 0.0282706585(9) |
| 4.0 | −0.57656349303(5) | −1.044336233(5) | 305.3(2) | 0.0271976883(10) |
| 4.1 | −0.5738981379(4) | −1.040756299(5) | 272.4(2) | 0.0261073114(9) |
| 4.2 | −0.5713423091(4) | −1.037648749(5) | 238.2(2) | 0.0250085404(9) |
| 4.3 | −0.5688964534(4) | −1.034984119(4) | 203.1(2) | 0.0239090205(8) |
| 4.4 | −0.5665603124(4) | −1.032733554(4) | 167.3(2) | 0.0228152434(8) |
| 4.5 | −0.56433302860(4) | −1.030868818(4) | 131.1(2) | 0.0217327198(7) |
| 4.6 | −0.5622132368(4) | −1.029362313(4) | 94.7(2) | 0.0206661219(7) |
| 4.7 | −0.5601991410(4) | −1.028187105(4) | 58.4(2) | 0.0196193993(6) |
| 4.8 | −0.5582885830(3) | −1.027316968(4) | 22.5(2) | 0.0185958747(6) |
| 4.9 | −0.5564790998(3) | −1.026726416(4) | −12.6(2) | 0.0175983232(6) |
| 5.0 | −0.55476797555(3) | −1.026390758(4) | −46.485(2) | 0.0166290386(6) |

## $2^1\Delta_g$ continued

| $R$ | $E$ | $\langle V\rangle$ | $10^6 \cdot \langle\nabla_1 \cdot \nabla_2\rangle$ | $\mathrm{d}E/\mathrm{d}R$ |
|---|---|---|---|---|
| 5.1 | −0.5531522871(2) | −1.026286143(2) | −79.4315(7) | 0.0156898885(3) |
| 5.2 | −0.5516289434(2) | −1.026389605(2) | −110.8608(7) | 0.0147823619(3) |
| 5.3 | −0.5501947219(2) | −1.026679113(2) | −140.5207(6) | 0.0139076095(3) |
| 5.4 | −0.5488463004(2) | −1.027133611(2) | −168.1766(6) | 0.0130664796(3) |
| 5.5 | −0.54758028570(3) | −1.027733055(2) | −193.6151(6) | 0.0122595485(2) |
| 5.6 | −0.5463932394(2) | −1.028458445(2) | −216.6473(6) | 0.0114871488(2) |
| 5.7 | −0.5452817009(2) | −1.029291853(2) | −237.1121(5) | 0.0107493945(2) |
| 5.8 | −0.5442422082(2) | −1.030216435(2) | −254.8786(5) | 0.0100462036(2) |
| 5.9 | −0.5432713164(2) | −1.031216447(2) | −269.8489(5) | 0.0093773196(2) |
| 6.0 | −0.54236561426(2) | −1.032277247(2) | −281.9597(5) | 0.0087423303(2) |
| 6.5 | −0.53869960442(2) | −1.0380567891(7) | −299.9114(4) | 0.00605267996(9) |
| 7.0 | −0.53619200485(2) | −1.0437716053(6) | −256.6901(3) | 0.00408748635(6) |
| 7.5 | −0.53451438596(3) | −1.0487145211(4) | −176.8895(3) | 0.00270856678(4) |
| 8.0 | −0.533409627363(7) | −1.0526346196(3) | −87.8654(3) | 0.00177307939(3) |
| 8.5 | −0.532688724014(5) | −1.0555684285(2) | −8.9711(2) | 0.00115400230(2) |
| 9.0 | −0.532219837300(4) | −1.05768436195(10) | 51.4683(2) | 0.000750590296(7) |
| 9.5 | −0.531914529402(2) | −1.05917808133(5) | 93.2808(2) | 0.000489576577(3) |
| 10.0 | −0.531714996043(2) | −1.06022288149(3) | 120.2700(2) | 0.0003207110602(6) |
| 11.0 | −0.5314981603599(7) | −1.06147956779(7) | 147.16930(8) | 0.000137886631(5) |
| 12.0 | −0.531405525917(3) | −1.0620946507(4) | 138.12363(8) | 0.00005970010(3) |
| 13.0 | −0.531361214888(5) | −1.0622847559(4) | 98.81519(9) | 0.00003366722(3) |
| 14.0 | −0.531333519958(5) | −1.0623473884(3) | 70.29746(9) | 0.00002283225(2) |
| 15.0 | −0.531314154695(5) | −1.0623827543(3) | 53.13734(9) | 0.00001637034(2) |
| 16.0 | −0.531300061427(5) | −1.0624066413(3) | 42.10912(9) | 0.00001209260(2) |
| 17.0 | −0.531289529900(4) | −1.0624236023(3) | 34.38081(9) | 0.000009144559(9) |
| 18.0 | −0.531281491309(4) | −1.0624361620(2) | 28.59996(9) | 0.000007045589(8) |
| 19.0 | −0.531275253649(3) | −1.0624459037(2) | 24.09626(6) | 0.000005505454(4) |
| 20.0 | −0.531270354143(3) | −1.06245378378(9) | 20.50273(5) | 0.000004346226(3) |

TABLE S19. Calculated BO energies, expectation value of potential, $\langle \nabla_1 \cdot \nabla_2 \rangle$, and $\mathrm{d}E/\mathrm{d}R$ of the $3^1\Delta_g$ state in atomic units (hartree). Uncertainties originate purely from extrapolation to the complete basis set limit. United atom values at $R = 0$ are taken from Ref. [1].

| $3^1\Delta_\mathrm{g}$ | | | | |
|---|---|---|---|---|
| $R$ | $E$ | $\langle V \rangle$ | $10^6 \cdot \langle \nabla_1 \cdot \nabla_2 \rangle$ | $\mathrm{d}E/\mathrm{d}R$ |
| 0.0 | −2.020015836159984(4) | – | 71.883131(6) | – |
| 0.01 | 97.980245529(5) | 95.96100853(5) | 71.86(4) | −9999.948252(4) |
| 0.05 | 17.98600758(2) | 15.98344649(9) | 72.51(4) | −399.771373(2) |
| 0.1 | 8.00174219(3) | 6.0425873(2) | 74.28(6) | −99.608970(4) |
| 0.15 | 4.69092953(2) | 2.7905671(2) | 76.90(7) | −43.9419463(6) |
| 0.2 | 3.05136446(2) | 1.21797248(10) | 80.19(7) | −24.4237822(4) |
| 0.3 | 1.446615227(10) | −0.24542957(8) | 88.25(6) | −10.4622001(3) |
| 0.4 | 0.679233933(8) | −0.87617091(7) | 97.78(6) | −5.5865969(2) |
| 0.5 | 0.245002857(8) | −1.18565933(7) | 108.37(6) | −3.35133009(10) |
| 0.6 | −0.02482075981(3) | −1.3443566609(3) | 3.258(2) | −2.1578585688(4) |
| 0.7 | −0.20262823114(3) | −1.42412848659(2) | 3.8803(6) | −1.45553146343(9) |
| 0.8 | −0.324484267791(10) | −1.45979147600(5) | 4.58869(5) | −1.01352867552(4) |
| 0.9 | −0.410275539110(6) | −1.46979576992(4) | 5.40304(3) | −0.72138299077(3) |
| 1.0 | −0.471792341600(3) | −1.46455714368(2) | 6.326945(5) | −0.520972460483(9) |
| 1.1 | −0.516418973735(4) | −1.45023169847(3) | 7.368367(9) | −0.37944886454(2) |
| 1.2 | −0.548982812872(3) | −1.43058337193(3) | 8.536557(8) | −0.27718145515(2) |
| 1.3 | −0.572750197621(2) | −1.40797143246(2) | 9.841779(7) | −0.20190079786(2) |
| 1.4 | −0.589994499745(3) | −1.38390067775(3) | 11.295451(8) | −0.14565119875(2) |
| 1.5 | −0.602335685102(2) | −1.35934118596(3) | 12.910269(8) | −0.10311321051(2) |
| 1.6 | −0.610951328144(2) | −1.33492068687(3) | 14.700317(7) | −0.07063626912(2) |
| 1.7 | −0.616712117902(2) | −1.31104368066(2) | 16.681248(6) | −0.045658496972(10) |
| 1.8 | −0.620271353389(2) | −1.28796700419(2) | 18.870468(5) | −0.026346831894(8) |
| 1.9 | −0.622125505637(2) | −1.26584875641(2) | 21.287345(4) | −0.011367234282(7) |
| 2.0 | −0.6226560805980(7) | −1.244780524050(7) | 23.95346839(2) | 0.000265818573(3) |
| 2.1 | −0.622159103652(2) | −1.22480891484(2) | 26.892898(3) | 0.009290139270(7) |
| 2.2 | −0.620866234232(2) | −1.20595011697(2) | 30.132527(3) | 0.016264705222(7) |
| 2.3 | −0.618960112991(2) | −1.18819983612(3) | 33.702399(3) | 0.021617560808(8) |
| 2.4 | −0.616585666905(3) | −1.17154012524(3) | 37.636135(4) | 0.025679670239(9) |
| 2.5 | −0.613858537891(3) | −1.15594410005(3) | 41.971406(4) | 0.028709190293(10) |
| 2.6 | −0.610871435917(3) | −1.14137920080(4) | 46.750460(5) | 0.03090910424(2) |
| 2.7 | −0.607698975532(4) | −1.12780944559(4) | 52.020736(5) | 0.03244018721(2) |
| 2.8 | −0.604401391425(2) | −1.115196979360(4) | 57.835574(2) | 0.03343064410335(5) |
| 2.9 | −0.601027416646(4) | −1.10350312872(6) | 64.254979(7) | 0.03398334640(2) |
| 3.0 | −0.597616529274(10) | −1.0926891085(2) | 71.34661(2) | 0.03418131668(4) |
| 3.1 | −0.59420071848(2) | −1.0827164840(2) | 79.1862(4) | 0.03409192033(5) |
| 3.2 | −0.59080588190(2) | −1.0735474610(2) | 87.8620(9) | 0.03377009463(5) |
| 3.3 | −0.58745293793(2) | −1.0651450579(2) | 97.46971(6) | 0.03326085393(5) |
| 3.4 | −0.58415871625(2) | −1.0574731960(2) | 108.1208(4) | 0.03260124604(5) |
| 3.5 | −0.58093667459(2) | −1.0504967369(3) | 119.94097(4) | 0.03182188922(6) |
| 3.6 | −0.57779747858(2) | −1.0441814875(3) | 133.07352(3) | 0.03094818602(6) |
| 3.7 | −0.57474947340(2) | −1.0384941867(3) | 147.68172(5) | 0.03000128651(6) |
| 3.8 | −0.57179906915(2) | −1.0334024864(3) | 163.95228(5) | 0.02899885575(6) |
| 3.9 | −0.56895105754(2) | −1.0288749346(3) | 182.09917(5) | 0.02795568731(5) |
| 4.0 | −0.56620887362(2) | −1.0248809676(3) | 202.36831(5) | 0.02688419490(5) |
| 4.1 | −0.563574813217(5) | −1.02139091720(8) | 225.0414(10) | 0.02579480713(2) |
| 4.2 | −0.561050215121(5) | −1.01837603642(8) | 250.4518(2) | 0.02469628424(2) |
| 4.3 | −0.558635614663(5) | −1.01580854864(8) | 278.9745(8) | 0.02359597225(2) |
| 4.4 | −0.556330874661(6) | −1.01366172450(8) | 311.0542(2) | 0.02250000564(2) |
| 4.5 | −0.55413529822(2) | −1.0119099911(3) | 347.21066(6) | 0.02141346786(5) |
| 4.6 | −0.552047727289(5) | −1.01052907920(8) | 388.05181(6) | 0.02034051639(2) |
| 4.7 | −0.550066630351(5) | −1.00949621840(9) | 434.29629(2) | 0.01928447709(2) |
| 4.8 | −0.548190181945(5) | −1.00879038834(9) | 486.79518(3) | 0.01824791157(2) |
| 4.9 | −0.546416336826(6) | −1.00839264490(9) | 546.56083(3) | 0.01723265893(2) |
| 5.0 | −0.54474290121(6) | −1.0082865417(10) | 614.8017(3) | 0.0162398521(2) |

| $3^1\Delta_g$ continued | | | | |
|---|---|---|---|---|
| $R$ | $E$ | $\langle V\rangle$ | $10^6\cdot\langle\nabla_1\cdot\nabla_2\rangle$ | $\mathrm{d}E/\mathrm{d}R$ |
| 5.1 | −0.54316760344(2) | −1.0084586730(3) | 692.96548(5) | 0.01526990861(4) |
| 5.2 | −0.54168816772(2) | −1.0088993914(3) | 782.78671(5) | 0.01432248924(4) |
| 5.3 | −0.54030239268(2) | −1.0096037279(3) | 886.34353(5) | 0.01339642594(4) |
| 5.4 | −0.53900823979(2) | −1.0105725927(3) | 1006.11187(4) | 0.01248960867(5) |
| 5.5 | −0.53780393483(2) | −1.0118142927(3) | 1145.00707(4) | 0.01159883217(5) |
| 5.6 | −0.53668808661(2) | −1.0133463660(3) | 1306.38205(3) | 0.01071960844(5) |
| 5.7 | −0.53565982494(2) | −1.0151975807(4) | 1493.92352(2) | 0.00984597705(5) |
| 5.8 | −0.53471895438(3) | −1.0174095824(4) | 1711.336777(8) | 0.00897040111(6) |
| 5.9 | −0.53386610648(3) | −1.0200369111(6) | 1961.636077(6) | 0.00808394947(8) |
| 6.0 | −0.53310284405(3) | −1.0231427458(6) | 2245.78077(3) | 0.00717715704(10) |
| 6.5 | −0.53071320415(6) | −1.045964723(2) | 3768.18470(9) | 0.0023787208(3) |
| 7.0 | −0.53036271505(8) | −1.063480641(2) | 3646.6948(2) | −0.0003936016(2) |
| 7.5 | −0.53069709275(8) | −1.066977502(2) | 2672.5991(2) | −0.0007444422(2) |
| 8.0 | −0.53102272770(7) | −1.0663320411(8) | 1869.1923(2) | −0.00053582321(9) |
| 8.5 | −0.53123243163(6) | −1.0651220685(7) | 1297.1556(2) | −0.00031261239(7) |
| 9.0 | −0.53134699728(6) | −1.0641086033(7) | 897.6494(2) | −0.00015717874(6) |
| 9.5 | −0.53139969576(6) | −1.0633887598(6) | 619.7807(2) | −0.00006203877(6) |
| 10.0 | −0.53141584831(6) | −1.0629109010(6) | 426.3823(2) | −0.00000792044(5) |
| 11.0 | −0.53139704439(5) | −1.0623979304(5) | 195.2441(2) | 0.00003601440(3) |
| 12.0 | −0.53135574744(4) | −1.06220947639(9) | 95.2160(2) | 0.000041834873(2) |
| 13.0 | −0.53132000903(2) | −1.06226615858(4) | 72.0434(2) | 0.00002875842243(2) |
| 14.0 | −0.53129727480(2) | −1.06234791395(4) | 61.5091(2) | 0.0000176168325(10) |
| 15.0 | −0.531283198196(8) | −1.06239921337(3) | 52.0714(2) | 0.0000111455346(10) |
| 16.0 | −0.531274082048(7) | −1.06242958327(3) | 43.7143(2) | 0.0000074113018(8) |
| 17.0 | −0.531267896346(5) | −1.06244848971(2) | 36.6592(3) | 0.0000051354697(6) |
| 18.0 | −0.531263544934(4) | −1.06246106290(2) | 30.8478(3) | 0.0000036681647(4) |
| 19.0 | −0.531260402126(3) | −1.062469898203(10) | 26.1040(2) | 0.0000026792658(3) |
| 20.0 | −0.531258087002(3) | −1.062476355620(8) | 22.2333(2) | 0.0000019909192(2) |

TABLE S20. Calculated BO energies, expectation value of potential, $\langle\nabla_1 \cdot \nabla_2\rangle$, and $\mathrm{d}E/\mathrm{d}R$ of the $1^3\Delta_g$ state in atomic units (hartree). Uncertainties originate purely from extrapolation to the complete basis set limit. United atom values at $R = 0$ are taken from Ref. [1].

| $1^3\Delta_\mathrm{g}$ | | | | |
|---|---|---|---|---|
| $R$ | $E$ | $\langle V\rangle$ | $10^6 \cdot \langle\nabla_1 \cdot \nabla_2\rangle$ | $\mathrm{d}E/\mathrm{d}R$ |
| 0.0 | −2.055620732852246(6) | – | −25.322839(1) | – |
| 0.01 | 97.94462504930(8) | 95.8897675464(9) | −25.35573(6) | −9999.94825522(7) |
| 0.05 | 17.950387042(5) | 15.91220533(4) | −26.09617(10) | −399.7713751(5) |
| 0.1 | 7.966121699(10) | 5.97134665(7) | −28.2619(3) | −99.6089675(5) |
| 0.15 | 4.6553094399(8) | 2.719328728(6) | −31.674(5) | −43.94193434(3) |
| 0.2 | 3.0157452463(4) | 1.146738665(3) | −36.223(6) | −24.42375914(2) |
| 0.3 | 1.4109996263(2) | −0.316645940(2) | −48.556(2) | −10.462150644(3) |
| 0.4 | 0.64362474137(7) | −0.9473577703(7) | −65.07352(2) | −5.586518132(2) |
| 0.5 | 0.20940307854(4) | −1.2568041734(4) | −85.694007(5) | −3.3512206610(7) |
| 0.6 | −0.06041075435(4) | −1.4154237141(5) | −110.38069(8) | −2.1576703423(7) |
| 0.7 | −0.23819738850(2) | −1.4951069019(2) | −139.1039(4) | −1.4553030355(3) |
| 0.8 | −0.360028598215(2) | −1.5306657564(7) | −171.8273(5) | −1.013260701(2) |
| 0.9 | −0.445791132413(2) | −1.5405510218(10) | −208.490(3) | −0.7210763965(7) |
| 1.0 | −0.507275390884(2) | −1.5351791582(9) | −249.014(4) | −0.5206283763(6) |
| 1.1 | −0.551865793188(2) | −1.5207070223(4) | −293.314(2) | −0.3790685784(6) |
| 1.2 | −0.584389852239(6) | −1.5008993679(4) | −341.2821(7) | −0.2767663864(5) |
| 1.3 | −0.6081140544401(10) | −1.4781163328(3) | −392.790(3) | −0.2014524802(4) |
| 1.4 | −0.625311930040(2) | −1.4538636329(10) | −447.7023(3) | −0.1451712662(6) |
| 1.5 | −0.637603612891(2) | −1.4291123072(10) | −505.8724(3) | −0.1026033875(5) |
| 1.6 | −0.646166854039(2) | −1.4044910871(10) | −567.1388(8) | −0.0700983618(5) |
| 1.7 | −0.651872526918(2) | −1.3804055102(2) | −631.3291(2) | −0.04509438610(6) |
| 1.8 | −0.655374122083(2) | −1.3571134842(10) | −698.274(2) | −0.0257584667(5) |
| 1.9 | −0.6571683086315(8) | −1.3347742060(2) | −767.784(4) | −0.0107566258(2) |
| 2.0 | −0.657636796522(2) | −1.3134803887(10) | −839.663(2) | 0.0008966022(5) |
| 2.1 | −0.6570758205306(7) | −1.29327978465(10) | −913.7167(2) | 0.00993897925(4) |
| 2.2 | −0.6557172543224(7) | −1.27418974794(10) | −989.7472(2) | 0.01692943668(4) |
| 2.3 | −0.653743957076(2) | −1.25620716262(10) | −1067.5422(2) | 0.02229597893(4) |
| 2.4 | −0.6513010780162(7) | −1.23931526982(9) | −1146.892(5) | 0.02636953583(10) |
| 2.5 | −0.6485044844504(7) | −1.22348837915(8) | −1227.565(5) | 0.02940823581(9) |
| 2.6 | −0.6454471142490(7) | −1.20869512355(6) | −1309.340(5) | 0.03161504027(9) |
| 2.7 | −0.6422038117048(7) | −1.19490070783(10) | −1391.97425(7) | 0.03315070947(3) |
| 2.8 | −0.6388350423590(8) | −1.1820684492(3) | −1475.2380(5) | 0.0341434412(2) |
| 2.9 | −0.6353897704070(7) | −1.17016082620(3) | −1558.879(6) | 0.03469610840(7) |
| 3.0 | −0.631907704457(2) | −1.159140176(2) | −1642.623(4) | 0.0348917445(3) |
| 3.1 | −0.628421062577(2) | −1.148969140(2) | −1726.208(5) | 0.0347977370(3) |
| 3.2 | −0.624955968495(3) | −1.139610953(2) | −1809.350(5) | 0.0344690574(3) |
| 3.3 | −0.6215335626069(8) | −1.13102958908(2) | −1891.755(6) | 0.03395076845(6) |
| 3.4 | −0.618170890977(2) | −1.123189844(2) | −1973.113(5) | 0.0332799818(3) |
| 3.5 | −0.6148816203646(8) | −1.11605734361(5) | −2053.110(7) | 0.03248739912(5) |
| 3.6 | −0.611676616151(2) | −1.109598538(2) | −2131.407(6) | 0.0315985263(3) |
| 3.7 | −0.608564411632(2) | −1.103780647(2) | −2207.662(6) | 0.0306346424(4) |
| 3.8 | −0.605551590831(2) | −1.098571620(2) | −2281.517(6) | 0.0296135689(4) |
| 3.9 | −0.602643102140(2) | −1.093940079(2) | −2352.600(6) | 0.0285502886(4) |
| 4.0 | −0.599842516471(2) | −1.089855263(2) | −2420.532(6) | 0.0274574425(4) |
| 4.1 | −0.597152240675(7) | −1.08628698426(9) | −2484.91710(7) | 0.02634573100(2) |
| 4.2 | −0.594573694841(7) | −1.08320559281(9) | −2545.37141(7) | 0.02522423735(2) |
| 4.3 | −0.592107460330(7) | −1.08058194455(8) | −2601.49028(7) | 0.02410069212(2) |
| 4.4 | −0.589743404029(7) | −1.07838738733302(5) | −2652.87520(7) | 0.022977141068(4) |
| 4.5 | −0.5875107832469(10) | −1.076593756(2) | −2699.140(7) | 0.0218728469(4) |
| 4.6 | −0.585368334828(4) | −1.07517346(6) | −2739.883(4) | 0.02077461(2) |
| 4.7 | −0.583354351324(4) | −1.07409906378(5) | −2774.743295(6) | 0.019704178482(8) |
| 4.8 | −0.581436746574(4) | −1.07334419028(5) | −2803.381918(7) | 0.018651938097(7) |
| 4.9 | −0.579623112577(4) | −1.07288266639(4) | −2825.475753(8) | 0.017625216075(7) |
| 5.0 | −0.5779107691510(7) | −1.0726890053(2) | −2840.742633(4) | 0.01662650660(4) |

| $1^3\Delta_g$ continued | | | | |
|---|---|---|---|---|
| $R$ | $E$ | $\langle V\rangle$ | $10^6\cdot\langle\nabla_1\cdot\nabla_2\rangle$ | $\mathrm{d}E/\mathrm{d}R$ |
| 5.1 | −0.576296807654(6) | −1.07273836078(6) | −2848.9437(2) | 0.015657893045(10) |
| 5.2 | −0.574778129728(6) | −1.07300657564(6) | −2849.8905(2) | 0.014721093041(9) |
| 5.3 | −0.573351481941(6) | −1.07347023344(6) | −2843.4525(2) | 0.013817496310(9) |
| 5.4 | −0.572013486940(5) | −1.07410671348(6) | −2829.5632(2) | 0.012948196370(8) |
| 5.5 | −0.5707606716936(8) | −1.0748942480(2) | −2808.22564(3) | 0.01211401735(2) |
| 5.6 | −0.569589493266(5) | −1.07581198016(5) | −2779.5176(2) | 0.011315536853(7) |
| 5.7 | −0.568496362453(5) | −1.07684002364(5) | −2743.5929(2) | 0.010553105485(6) |
| 5.8 | −0.567477665622(5) | −1.07795951993(5) | −2700.6835(2) | 0.009826864019(6) |
| 5.9 | −0.566529784916(4) | −1.07915269460(4) | −2651.0982(2) | 0.009136758514(6) |
| 6.0 | −0.5656491170275(6) | −1.0804029094(2) | −2595.21896(6) | 0.00848255411(3) |
| 6.5 | −0.5621309641209(6) | −1.087011918600(7) | −2239.09406(2) | 0.0057307707138(8) |
| 7.0 | −0.5597879212474(5) | −1.09325801162(3) | −1811.0158(6) | 0.003759690125(3) |
| 7.5 | −0.5582667435321(5) | −1.098417534964(6) | −1385.58400(3) | 0.0024154602799(6) |
| 8.0 | −0.5572956569909(4) | −1.102328492734(6) | −1013.92884(5) | 0.0015328526558(5) |
| 8.5 | −0.5566811365466(3) | −1.105134321154(3) | −716.962011(5) | 0.0009679943456(3) |
| 9.0 | −0.5562930619288(3) | −1.107079221805(4) | −493.75996(4) | 0.0006118780057(4) |
| 9.5 | −0.5560472002632(3) | −1.10839913564(3) | −332.87618(5) | 0.000388975251(3) |
| 10.0 | −0.5558902474374(3) | −1.10928348864(3) | −220.21685(3) | 0.000249700624(2) |
| 11.0 | −0.5557224198360(2) | −1.110261603490(8) | −90.6807789(4) | 0.0001075669258(5) |
| 12.0 | −0.55564767706476(2) | −1.110692286359(5) | −32.667748551(3) | 0.0000502556477(3) |
| 13.0 | −0.55561124984318(9) | −1.110886058163(9) | −7.645756(7) | 0.0000258801173(5) |
| 14.0 | −0.55559165020191(7) | −1.110977966709(6) | 2.71341(6) | 0.0000146666925(2) |
| 15.0 | −0.55558011398760(5) | −1.111025264127(4) | 6.68030(4) | 0.00000899758997(10) |
| 16.0 | −0.55557283203673(4) | −1.111052064170(3) | 7.89325(2) | 0.00000584999403(7) |
| 17.0 | −0.55556800184259(3) | −1.111068688028(2) | 7.938663(3) | 0.00000395974459(2) |
| 18.0 | −0.55556468643292(2) | −1.1110797536846(5) | 7.50969(4) | 0.00000275662117(2) |
| 19.0 | −0.55556235472174(2) | −1.1110874859744(4) | 6.91140(2) | 0.00000195912994(2) |
| 20.0 | −0.555560684284435(9) | −1.1110930626904(3) | 6.2781(2) | 0.00000141529389(4) |

TABLE S21. Calculated BO energies, expectation value of potential, $\langle \nabla_1 \cdot \nabla_2 \rangle$, and $\mathrm{d}E/\mathrm{d}R$ of the $2^3\Delta_g$ state in atomic units (hartree). Uncertainties originate purely from extrapolation to the complete basis set limit. United atom values at $R = 0$ are taken from Ref. [1].

| $2^3\Delta_\mathrm{g}$ | | | | |
|---|---|---|---|---|
| $R$ | $E$ | $\langle V \rangle$ | $10^6 \cdot \langle \nabla_1 \cdot \nabla_2 \rangle$ | $\mathrm{d}E/\mathrm{d}R$ |
| 0.0 | −2.031279846178687(7) | – | −29.442651(2) | – |
| 0.01 | 97.9689725121(7) | 95.938462474(8) | −29.469(3) | −9999.9482550(6) |
| 0.05 | 17.974734485(4) | 15.96090013(4) | −30.01(5) | −399.7713769(5) |
| 0.1 | 7.990468955(6) | 6.02004048(4) | −31.46(2) | −99.6089743(3) |
| 0.15 | 4.679656209(10) | 2.76802020(7) | −33.7075(9) | −43.9419481(3) |
| 0.2 | 3.040091094(3) | 1.19542577(3) | −36.68(2) | −24.42378207(10) |
| 0.3 | 1.435342162(2) | −0.26797399(2) | −44.50(2) | −10.46219438(5) |
| 0.4 | 0.667961781(2) | −0.89871023(2) | −54.65(2) | −5.58658448(3) |
| 0.5 | 0.2337323229(10) | −1.208190492(10) | −66.996(10) | −3.35131028(2) |
| 0.6 | −0.0360916399(7) | −1.366853264(8) | −81.468(10) | −2.157783306(10) |
| 0.7 | −0.2138907282(6) | −1.446588820(7) | −97.996(10) | −1.455439091(8) |
| 0.8 | −0.3357366789(5) | −1.482208857(6) | −116.517(7) | −1.013419374(6) |
| 0.9 | −0.4215161861(4) | −1.492163735(5) | −136.969(4) | −0.721257070(5) |
| 1.0 | −0.4830195816(3) | −1.486869480(5) | −159.282(3) | −0.520830317(4) |
| 1.1 | −0.5276312074(3) | −1.472482477(5) | −183.379(2) | −0.379290966(4) |
| 1.2 | −0.5601784906(2) | −1.452766973(4) | −209.1785(9) | −0.277008326(3) |
| 1.3 | −0.5839278245(2) | −1.430082564(4) | −236.5913(7) | −0.201713011(3) |
| 1.4 | −0.6011526405(2) | −1.405934398(4) | −265.5248(7) | −0.145449369(3) |
| 1.5 | −0.6134729678(2) | −1.381292919(4) | −295.8820(8) | −0.102897989(2) |
| 1.6 | −0.6220664474(2) | −1.356786237(4) | −327.58(2) | −0.070408339(2) |
| 1.7 | −0.62780383818(2) | −1.332819244(3) | −360.4655(9) | −0.045418569(2) |
| 1.8 | −0.63133851155(10) | −1.309649179(3) | −394.4858(9) | −0.026095642(2) |
| 1.9 | −0.63316701315(9) | −1.287434551(3) | −429.5186(10) | −0.011105539(2) |
| 2.0 | −0.63367092550(8) | −1.266267361(3) | −465.4583(10) | 0.000537245(2) |
| 2.1 | −0.63314635209(7) | −1.246194635(3) | −502.1985(10) | 0.009570509(2) |
| 2.2 | −0.63182503171(7) | −1.227232979(3) | −539.6328(10) | 0.016553220(2) |
| 2.3 | −0.62988968521(6) | −1.209378513(4) | −577.6546(10) | 0.021913416(2) |
| 2.4 | −0.62748532021(6) | −1.192613701(4) | −616.1572(9) | 0.025982058(2) |
| 2.5 | −0.62472765933(6) | −1.176912056(4) | −655.0335(9) | 0.029017305(2) |
| 2.6 | −0.62170949287(5) | −1.162241406(4) | −694.1763(9) | 0.031222146(2) |
| 2.7 | −0.61850551483(5) | −1.148566136(4) | −733.4775(10) | 0.032757368(2) |
| 2.8 | −0.61517603792(5) | −1.135848738(4) | −772.8280(8) | 0.0337511920(10) |
| 2.9 | −0.61176987127(4) | −1.124050855(4) | −812.1178(8) | 0.0343065130(10) |
| 3.0 | −0.60832656637(4) | −1.11313399(2) | −851.25(2) | 0.034506381(4) |
| 3.1 | −0.60487818243(4) | −1.103059926(4) | −890.0658(8) | 0.0344182061(10) |
| 3.2 | −0.60145068294(4) | −1.093791078(4) | −928.4939(8) | 0.0340969651(10) |
| 3.3 | −0.59806504702(4) | −1.085290582(4) | −966.4002(6) | 0.0335877309(9) |
| 3.4 | −0.59473815889(4) | −1.077522413(4) | −1003.666(5) | 0.0329276190(10) |
| 3.5 | −0.59148352338(3) | −1.070451397(4) | −1040.158(2) | 0.0321473285(10) |
| 3.6 | −0.58831184448(3) | −1.064043203(5) | −1075.756(5) | 0.0312723574(10) |
| 3.7 | −0.58523149528(3) | −1.058264307(5) | −1110.318(2) | 0.0303239686(10) |
| 3.8 | −0.58224890156(3) | −1.053081955(5) | −1143.717(2) | 0.0293199600(10) |
| 3.9 | −0.57936885630(3) | −1.048464116(5) | −1175.812(3) | 0.0282752813(10) |
| 4.0 | −0.57659477884(3) | −1.044379438(5) | −1206.450(3) | 0.0272025301(10) |
| 4.1 | −0.5739289295(5) | −1.040797219(6) | −1235.497(6) | 0.026112351(2) |
| 4.2 | −0.5713725875(5) | −1.037687381(6) | −1262.795(6) | 0.025013760(2) |
| 4.3 | −0.5689262015(5) | −1.035020456(6) | −1288.197(5) | 0.023914406(2) |
| 4.4 | −0.5665895141(5) | −1.032767585(6) | −1311.552(5) | 0.022820783(2) |
| 4.5 | −0.56436166909(3) | −1.030900528(6) | −1332.708(5) | 0.0217384024(10) |
| 4.6 | −0.5622413022(4) | −1.029391681(5) | −1351.516(5) | 0.0206719399(10) |
| 4.7 | −0.5602266182(4) | −1.028214111(5) | −1367.831(5) | 0.0196253458(9) |
| 4.8 | −0.5583154593(4) | −1.027341588(5) | −1381.513(5) | 0.0186019439(9) |
| 4.9 | −0.5565053632(4) | −1.026748628(5) | −1392.426(5) | 0.0176045099(8) |
| 5.0 | −0.55479361463(2) | −1.026410541(4) | −1400.44484(10) | 0.0166353376(6) |

| $2^3\Delta_g$ continued | | | | |
|---|---|---|---|---|
| $R$ | $E$ | $\langle V\rangle$ | $10^6\cdot\langle\nabla_1\cdot\nabla_2\rangle$ | $\mathrm{d}E/\mathrm{d}R$ |
| 5.1 | −0.5531772909(2) | −1.026303479(2) | −1405.4641(2) | 0.0156962946(2) |
| 5.2 | −0.5516533014(2) | −1.026404484(2) | −1407.3816(2) | 0.0147888689(2) |
| 5.3 | −0.5502184245(2) | −1.026691531(2) | −1406.1164(2) | 0.0139142109(2) |
| 5.4 | −0.54886933846(10) | −1.027143573(2) | −1401.6063(2) | 0.0130731674(2) |
| 5.5 | −0.54760265103(2) | −1.0277405768(10) | −1393.8112(2) | 0.0122663137(2) |
| 5.6 | −0.54641492477(9) | −1.0284635559(10) | −1382.7146(2) | 0.0114939810(2) |
| 5.7 | −0.54530270018(9) | −1.0292945940(10) | −1368.3266(2) | 0.0107562818(2) |
| 5.8 | −0.54426251653(9) | −1.0302168624(9) | −1350.6849(2) | 0.0100531329(2) |
| 5.9 | −0.54329093035(8) | −1.0312146314(9) | −1329.8563(2) | 0.0093842762(2) |
| 6.0 | −0.54238453182(2) | −1.0322732727(8) | −1305.9379(2) | 0.0087492985(2) |
| 6.5 | −0.53871507082(2) | −1.0380437812(6) | −1145.4508(2) | 0.00605944007(8) |
| 7.0 | −0.536204237204(9) | −1.0437533092(5) | −937.8097(2) | 0.00409359503(6) |
| 7.5 | −0.534523796106(7) | −1.0486947488(4) | −717.6113(2) | 0.00271371246(4) |
| 8.0 | −0.533416729668(5) | −1.0526161254(3) | −515.4714(2) | 0.00177716675(3) |
| 8.5 | −0.532694032132(4) | −1.0555525791(2) | −348.8171(2) | 0.00115711590(2) |
| 9.0 | −0.532223797072(3) | −1.0576714852(2) | −221.4210(2) | 0.000752900992(9) |
| 9.5 | −0.531917496946(2) | −1.05916800312(7) | −128.38712(10) | 0.000491262187(5) |
| 10.0 | −0.5317172469052(10) | −1.06021538919(4) | −61.39762(9) | 0.000321910462(2) |
| 11.0 | −0.5314996327340(6) | −1.06147873220(5) | 25.43585(7) | 0.000138230297(4) |
| 12.0 | −0.531407019747(2) | −1.0620995850(3) | 55.14599(6) | 0.00005953787(2) |
| 13.0 | −0.531362675665(4) | −1.0622850013(3) | 35.41638(5) | 0.00003387308(2) |
| 14.0 | −0.531334713043(4) | −1.0623456789(3) | 21.79898(5) | 0.00002312480(2) |
| 15.0 | −0.531315067671(4) | −1.0623806803(2) | 16.47654(3) | 0.000016630336(9) |
| 16.0 | −0.531300740548(3) | −1.0624046820(2) | 14.51684(2) | 0.000012299941(7) |
| 17.0 | −0.531290026783(3) | −1.0624219029(2) | 13.59824(2) | 0.000009302982(6) |
| 18.0 | −0.531281850639(3) | −1.06243475293(10) | 12.87428(2) | 0.000007163798(4) |
| 19.0 | −0.531275511183(2) | −1.06244477030(9) | 12.09832(2) | 0.000005592215(3) |
| 20.0 | −0.531270537434(2) | −1.06245289313(7) | 11.23870(2) | 0.000004409087(3) |

TABLE S22. Calculated BO energies, expectation value of potential, $\langle \nabla_1 \cdot \nabla_2 \rangle$, and $\mathrm{d}E/\mathrm{d}R$ of the $3^3\Delta_g$ state in atomic units (hartree). Uncertainties originate purely from extrapolation to the complete basis set limit. United atom values at $R = 0$ are taken from Ref. [1].

| $3^3\Delta_\mathrm{g}$ | | | | |
|---|---|---|---|---|
| $R$ | $E$ | $\langle V \rangle$ | $10^6 \cdot \langle \nabla_1 \cdot \nabla_2 \rangle$ | $\mathrm{d}E/\mathrm{d}R$ |
| 0.0 | −2.020015836159984(4) | – | −19.56885(1) | – |
| 0.01 | 97.980240336(6) | 95.96099815(6) | −19.66(4) | −9999.948252(5) |
| 0.05 | 17.98600234(2) | 15.9834359(2) | −19.97(4) | −399.771375(2) |
| 0.1 | 8.00173682(3) | 6.0425762(2) | −20.90(6) | −99.608974(2) |
| 0.15 | 4.69092398(3) | 2.7905554(2) | −22.38(4) | −43.9419503(8) |
| 0.2 | 3.05135868(2) | 1.2179599(2) | −24.03(7) | −24.4237871(6) |
| 0.3 | 1.44660888(2) | −0.2454441(2) | −28.63(6) | −10.4622063(4) |
| 0.4 | 0.67922692(2) | −0.87618769(6) | −34.56(6) | −5.5866038(2) |
| 0.5 | 0.2450098726(6) | −1.185664469(2) | 2.72786(4) | −3.351368428(2) |
| 0.6 | −0.02482075993(2) | −1.3443566621(2) | 3.25513(2) | −2.1578585705(2) |
| 0.7 | −0.20262823103(2) | −1.4241284873(2) | 3.87182(2) | −1.4555314646(2) |
| 0.8 | −0.32448426727(7) | −1.459791455(6) | 4.541(8) | −1.013528650(7) |
| 0.9 | −0.41027553947(2) | −1.46979576872(4) | 5.3951(2) | −0.721382988716(8) |
| 1.0 | −0.471792341884(4) | −1.46455714418(2) | 6.321800(10) | −0.520972460410(9) |
| 1.1 | −0.516418974033(5) | −1.45023169936(4) | 7.363100(6) | −0.37944886481(2) |
| 1.2 | −0.548982813206(3) | −1.43058337311(3) | 8.530611(4) | −0.27718145558(2) |
| 1.3 | −0.572750198003(3) | −1.40797143393(3) | 9.834862(3) | −0.20190079841(2) |
| 1.4 | −0.589994500187(3) | −1.38390067954(3) | 11.287318(3) | −0.14565119940(2) |
| 1.5 | −0.602335685614(3) | −1.35934118812(3) | 12.900662(3) | −0.10311321126(2) |
| 1.6 | −0.610951328737(3) | −1.33492068945(3) | 14.688959(3) | −0.07063626998(2) |
| 1.7 | −0.616712118588(3) | −1.31104368370(3) | 16.667831(4) | −0.04565849796(2) |
| 1.8 | −0.620271354180(2) | −1.28796700777(3) | 18.854643(5) | −0.026346833004(10) |
| 1.9 | −0.622125506546(2) | −1.26584876060(2) | 21.268721(5) | −0.011367235528(9) |
| 2.0 | −0.6226560816383(9) | −1.244780528913(9) | 23.931594(3) | 0.000265817182(4) |
| 2.1 | −0.622159104839(2) | −1.22480892046(3) | 26.867283(6) | 0.009290137724(8) |
| 2.2 | −0.620866235582(3) | −1.20595012344(3) | 30.102592(6) | 0.016264703510(9) |
| 2.3 | −0.618960114521(3) | −1.18819984353(3) | 33.667497(5) | 0.021617558919(9) |
| 2.4 | −0.616585668633(3) | −1.17154013368(3) | 37.595537(6) | 0.025679668162(10) |
| 2.5 | −0.613858539837(3) | −1.15594410963(4) | 41.924287(6) | 0.02870918802(2) |
| 2.6 | −0.610871438101(4) | −1.14137921164(4) | 46.695893(6) | 0.03090910175(2) |
| 2.7 | −0.607698977976(4) | −1.12780945780(5) | 51.957680(5) | 0.03244018450(2) |
| 2.8 | −0.604401394151(2) | −1.115196993063(6) | 57.762856(3) | 0.0334306411570(6) |
| 2.9 | −0.601027419679(5) | −1.10350314404(6) | 64.171318(5) | 0.03398334321(2) |
| 3.0 | −0.59761653264(2) | −1.0926891256(2) | 71.250577(8) | 0.03418131323(4) |
| 3.1 | −0.59420072221(2) | −1.0827165029(2) | 79.069(5) | 0.03409191662(5) |
| 3.2 | −0.59080588601(2) | −1.0735474819(2) | 87.74(2) | 0.03377009065(5) |
| 3.3 | −0.58745294245(2) | −1.0651450810(2) | 97.3262(4) | 0.03326084967(5) |
| 3.4 | −0.58415872121(2) | −1.0574732213(3) | 107.958(6) | 0.03260124151(5) |
| 3.5 | −0.58093668001(2) | −1.0504967646(3) | 119.755627(3) | 0.03182188442(6) |
| 3.6 | −0.57779748450(2) | −1.0441815176(3) | 132.8631(3) | 0.03094818095(6) |
| 3.7 | −0.57474947984(2) | −1.0384942193(3) | 147.444688(6) | 0.03000128119(6) |
| 3.8 | −0.57179907613(2) | −1.0334025214(3) | 163.68533(6) | 0.02899885021(6) |
| 3.9 | −0.56895106509(2) | −1.0288749720(3) | 181.79943(2) | 0.02795568158(6) |
| 4.0 | −0.56620888174(2) | −1.0248810073(3) | 202.03283(2) | 0.02688418904(6) |
| 4.1 | −0.563574821934(5) | −1.02139095893(9) | 224.63(3) | 0.02579480120(2) |
| 4.2 | −0.561050224431(5) | −1.01837607986(8) | 250.036(6) | 0.02469627833(2) |
| 4.3 | −0.558635624559(5) | −1.01580859333(9) | 278.51(2) | 0.02359596646(2) |
| 4.4 | −0.556330885125(5) | −1.01366176988(9) | 310.542(3) | 0.02250000008(2) |
| 4.5 | −0.55413530922(2) | −1.0119100365(3) | 346.65317(3) | 0.02141346266(5) |
| 4.6 | −0.552047738789(5) | −1.01052912393(9) | 387.4423(4) | 0.02034051166(2) |
| 4.7 | −0.550066642295(6) | −1.00949626186(9) | 433.63260(5) | 0.01928447292(2) |
| 4.8 | −0.548190194278(6) | −1.00879043036(10) | 486.07540(5) | 0.01824790796(2) |
| 4.9 | −0.546416349499(6) | −1.00839268615(10) | 545.78230(4) | 0.01723265568(2) |
| 5.0 | −0.54474291421(7) | −1.0082865847(10) | 613.9605(2) | 0.0162398488(2) |

| $3^3\Delta_g$ continued | | | | |
|---|---|---|---|---|
| $R$ | $E$ | $\langle V\rangle$ | $10^6\cdot\langle\nabla_1\cdot\nabla_2\rangle$ | $\mathrm{d}E/\mathrm{d}R$ |
| 5.1 | −0.54316761682(2) | −1.0084587230(3) | 692.05452(4) | 0.01526990404(5) |
| 5.2 | −0.54168818170(2) | −1.0088994598(3) | 781.79311(4) | 0.01432248147(5) |
| 5.3 | −0.54030240773(2) | −1.0096038350(3) | 885.24361(4) | 0.01339641141(5) |
| 5.4 | −0.53900825687(2) | −1.0105727748(3) | 1004.86318(4) | 0.01248958129(5) |
| 5.5 | −0.53780395569(2) | −1.0118146116(3) | 1143.53539(4) | 0.01159878178(5) |
| 5.6 | −0.53668811432(2) | −1.0133469251(4) | 1304.56053(3) | 0.01071951849(5) |
| 5.7 | −0.53565986467(3) | −1.0151985489(4) | 1491.53991(3) | 0.00984582113(6) |
| 5.8 | −0.53471901464(3) | −1.0174112285(5) | 1708.043105(9) | 0.00897013806(7) |
| 5.9 | −0.53386620088(3) | −1.0200396499(6) | 1956.874302(8) | 0.00808351726(8) |
| 6.0 | −0.53310299371(3) | −1.0231471870(6) | 2238.68008(3) | 0.00717646674(9) |
| 6.5 | −0.53071433556(6) | −1.045989737(2) | 3719.45614(7) | 0.0023752206(3) |
| 7.0 | −0.53036577326(7) | −1.063510617(2) | 3516.44777(6) | −0.0003970101(2) |
| 7.5 | −0.53070140753(6) | −1.0669989292(9) | 2492.69263(5) | −0.00074614856(10) |
| 8.0 | −0.53102760234(5) | −1.0663467826(7) | 1669.88804(4) | −0.00053644723(7) |
| 8.5 | −0.53123744011(5) | −1.0651317884(6) | 1095.46340(4) | −0.00031257744(6) |
| 9.0 | −0.53135188012(5) | −1.0641144711(6) | 702.96166(4) | −0.00015674566(5) |
| 9.5 | −0.53140429877(5) | −1.0633916497(5) | 436.81907(4) | −0.00006137391(5) |
| 10.0 | −0.53142008190(5) | −1.0629113374(5) | 256.79895(5) | −0.00000711736(4) |
| 11.0 | −0.53140034308(4) | −1.0623922987(4) | 49.83448(9) | 0.00003712613(3) |
| 12.0 | −0.53135777423(3) | −1.0621987740(2) | −27.0889(2) | 0.000043064539(5) |
| 13.0 | −0.53132114819(2) | −1.06226085837(6) | −23.6165(2) | 0.000029341385(2) |
| 14.0 | −0.531297999916(10) | −1.06234527030(5) | −14.1428(2) | 0.000017909252(2) |
| 15.0 | −0.531283697742(8) | −1.06239760563(4) | −8.8833(2) | 0.000011319324(2) |
| 16.0 | −0.531274440851(6) | −1.06242848435(3) | −6.0545(2) | 0.0000075248344(10) |
| 17.0 | −0.531268160774(5) | −1.06244769217(3) | −4.4091(2) | 0.0000052134928(7) |
| 18.0 | −0.531263743501(4) | −1.06246046509(2) | −3.3601(2) | 0.0000037234398(5) |
| 19.0 | −0.531260553538(3) | −1.06246944097(2) | −2.6373(2) | 0.0000027192686(3) |
| 20.0 | −0.531258204003(2) | −1.062476000706(8) | −2.1102(2) | 0.0000020203650(2) |

TABLE S23. Calculated BO energies, expectation value of potential, $\langle\nabla_1\cdot\nabla_2\rangle$, and $\mathrm{d}E/\mathrm{d}R$ of the $1^1\Delta_u$ state in atomic units (hartree). Uncertainties originate purely from extrapolation to the complete basis set limit. United atom values at $R=0$ are taken from Ref. [1].

| $1^1\Delta_\mathrm{u}$ | | | | |
|---|---|---|---|---|
| $R$ | $E$ | $\langle V\rangle$ | $10^6\cdot\langle\nabla_1\cdot\nabla_2\rangle$ | $\mathrm{d}E/\mathrm{d}R$ |
| 0.0 | −2.031255144381749(1) | – | 10.0242694(2) | – |
| 0.01 | 97.9690062215(9) | 95.93850(2) | 10.06(3) | −9999.951(2) |
| 0.05 | 17.974768201(3) | 15.9609672(4) | 10.083(9) | −399.771385(8) |
| 0.1 | 7.990502596(4) | 6.02010742(3) | 10.404697(2) | −99.6089776(2) |
| 0.15 | 4.679689561(4) | 2.76808562(2) | 10.819212(8) | −43.94195659(4) |
| 0.2 | 3.04012386(2) | 1.1954878(5) | 11.31(3) | −24.423800(3) |
| 0.3 | 1.4353727318(6) | −0.2679224(6) | 12.66(3) | −10.462226(2) |
| 0.4 | 0.6679885497(2) | −0.8986760(7) | 14.34(3) | −5.586633(2) |
| 0.5 | 0.23375357935(8) | −1.208179919(2) | 16.370(3) | −3.351374156(4) |
| 0.6 | −0.03607765666(3) | −1.3668742649(2) | 18.654(2) | −2.1578649194(2) |
| 0.7 | −0.213885795914(4) | −1.4466485349(2) | 21.2968(10) | −1.4555384901(2) |
| 0.8 | −0.335742572079(5) | −1.4823143080(2) | 24.2450(4) | −1.0135364547(2) |
| 0.9 | −0.42153466310(2) | −1.4923217876(4) | 27.542(2) | −0.7213916238(4) |
| 1.0 | −0.483052376483(2) | −1.4870868193(3) | 31.215(2) | −0.5209820664(2) |
| 1.1 | −0.527680023498(3) | −1.4727655857(3) | 35.26(2) | −0.3794595807(2) |
| 1.2 | −0.560244996210(2) | −1.4531221184(3) | 39.8032(9) | −0.2771934383(2) |
| 1.3 | −0.5840136499432(10) | −1.4305157935(3) | 44.7910(5) | −0.2019142258(2) |
| 1.4 | −0.601259375370(4) | −1.4064515320(2) | 50.29691(5) | −0.1456662723(2) |
| 1.5 | −0.613602159689(2) | −1.3818995538(3) | 56.36880(6) | −0.1031301563(2) |
| 1.6 | −0.622219601438(2) | −1.3574877512(2) | 63.06233(4) | −0.07065534268(9) |
| 1.7 | −0.627982416814(2) | −1.3336208112(3) | 70.43936(6) | −0.0456799868(2) |
| 1.8 | −0.631543935499(2) | −1.3105557856(2) | 78.5696(3) | −0.02637106367(8) |
| 1.9 | −0.633400663171(2) | −1.2884510211(2) | 87.5325(3) | −0.01139457618(7) |
| 2.0 | −0.6339341449639(10) | −1.2673983899(2) | 97.417179(9) | 0.00023495004(6) |
| 2.1 | −0.6334404506109(10) | −1.2474448293(2) | 108.3239(2) | 0.00925527233(6) |
| 2.2 | −0.6321512898081(5) | −1.2286069088(2) | 120.36757(2) | 0.01622530492(5) |
| 2.3 | −0.6302493602476(7) | −1.2108807752(2) | 133.67740(5) | 0.02157301970(5) |
| 2.4 | −0.6278796537133(5) | −1.1942489931(2) | 148.4007(2) | 0.02562929763(5) |
| 2.5 | −0.6251578858732(5) | −1.1786852727(2) | 164.7049(2) | 0.02865219961(4) |
| 2.6 | −0.6221768507539(10) | −1.1641577462(2) | 182.7808(2) | 0.03084459820(4) |
| 2.7 | −0.6190112588871(10) | −1.1506312391(2) | 202.84595(6) | 0.03236714025(4) |
| 2.8 | −0.6157214547842(6) | −1.13806884120(2) | 225.149057(7) | 0.03334788156(4) |
| 2.9 | −0.6123562974337(10) | −1.12643298788(10) | 249.9749(2) | 0.03388951965(3) |
| 3.0 | −0.608955409700(2) | −1.1156862000(2) | 277.65094(5) | 0.03407487315(3) |
| 3.1 | −0.6055509476900(7) | −1.1057915868(2) | 308.5530(2) | 0.03397106730(3) |
| 3.2 | −0.6021690021118(7) | −1.0967131881(2) | 343.1154(2) | 0.03363275503(3) |
| 3.3 | −0.598830715508(2) | −1.0884162111(2) | 381.8397(2) | 0.03310461208(3) |
| 3.4 | −0.5955531787935(5) | −1.0808672039(3) | 425.30830(3) | 0.03242328049(8) |
| 3.5 | −0.592350155523(2) | −1.0740341990(2) | 474.1980(2) | 0.03161888915(4) |
| 3.6 | −0.589232671193(2) | −1.0678868580(3) | 529.29969(3) | 0.03071624567(6) |
| 3.7 | −0.586209496693(2) | −1.0623966370(2) | 591.53929(7) | 0.02973577200(4) |
| 3.8 | −0.583287548851(2) | −1.0575370076(3) | 662.00586(2) | 0.02869423425(7) |
| 3.9 | −0.580472226530(2) | −1.0532837537(3) | 741.98433(4) | 0.02760530753(5) |
| 4.0 | −0.577767697396(3) | −1.0496153895(3) | 832.99621(8) | 0.02648000131(6) |
| 4.1 | −0.57517714819(3) | −1.0465137343(5) | 936.8489(3) | 0.0253269664(2) |
| 4.2 | −0.57270300980(4) | −1.0439647094(6) | 1055.6943(3) | 0.0241526929(2) |
| 4.3 | −0.57034716783(4) | −1.0419594391(7) | 1192.0964(3) | 0.0229616039(2) |
| 4.4 | −0.56811116901(5) | −1.0404957531(9) | 1349.1058(4) | 0.0217560420(2) |
| 4.5 | −0.5659964346176(7) | −1.039580229(2) | 1530.3327(5) | 0.0205361424(3) |
| 4.6 | −0.56400449281(6) | −1.039230917(2) | 1739.9972(6) | 0.0192995801(3) |
| 4.7 | −0.56213724247(7) | −1.039480884(2) | 1982.9156(7) | 0.0180411916(3) |
| 4.8 | −0.56039726043(8) | −1.040382531(2) | 2264.3379(9) | 0.0167524978(4) |
| 4.9 | −0.55878815724(9) | −1.042012243(2) | 2589.4757(8) | 0.0154212391(4) |
| 5.0 | −0.557314967322(2) | −1.044473803(3) | 2962.4477(10) | 0.0140312264(5) |

| $1^1\Delta_u$ continued | | | | |
|---|---|---|---|---|
| $R$ | $E$ | $\langle V \rangle$ | $10^6 \cdot \langle \nabla_1 \cdot \nabla_2 \rangle$ | $\mathrm{d}E/\mathrm{d}R$ |
| 5.1 | −0.55598451220(2) | −1.0478967533(4) | 3384.221(9) | 0.01256319040(7) |
| 5.2 | −0.55480557796(2) | −1.0524220088(5) | 3849.173(8) | 0.01099791291(8) |
| 5.3 | −0.55378858966(3) | −1.0581627304(6) | 4340.116(6) | 0.00932348094(10) |
| 5.4 | −0.55294429515(3) | −1.0651302729(7) | 4823.567(5) | 0.0075478366(2) |
| 5.5 | −0.552281020395(6) | −1.0731365176(8) | 5249.445(4) | 0.0057137315(2) |
| 5.6 | −0.55180072019(4) | −1.0817308097(9) | 5560.935(3) | 0.0039054698(2) |
| 5.7 | −0.55149536294(5) | −1.0902582112(10) | 5714.5482(9) | 0.0022337745(2) |
| 5.8 | −0.55134599995(5) | −1.0980552082(10) | 5698.61866(2) | 0.0007994468(2) |
| 5.9 | −0.55132561055(6) | −1.1046623373(10) | 5535.5912(7) | −0.0003408672(2) |
| 6.0 | −0.551404212282(3) | −1.1099102658(3) | 5267.7377(2) | −0.00118364021(4) |
| 6.5 | −0.552457242666(2) | −1.1207431144(2) | 3570.4699(5) | −0.00243517370(2) |
| 7.0 | −0.553570837250(2) | −1.12068767251(9) | 2319.5660(3) | −0.001935142572(10) |
| 7.5 | −0.5543760645948(6) | −1.11852171002(4) | 1527.9872(2) | −0.001302610777(4) |
| 8.0 | −0.5548993990952(5) | −1.11635144667(3) | 1017.97888(9) | −0.000819081059(3) |
| 8.5 | −0.5552214294901(4) | −1.11462656199(2) | 681.77655(7) | −0.000492200354(2) |
| 9.0 | −0.5554112429334(4) | −1.11337238662(2) | 457.44891(7) | −0.000283322305(2) |
| 9.5 | −0.5555180750562(3) | −1.11250600870(2) | 307.25722(5) | −0.0001547219569(10) |
| 10.0 | −0.5555745677120(3) | −1.111929535416(10) | 206.88872(3) | −0.0000780399992(7) |
| 11.0 | −0.5556116632044(2) | −1.111326455803(7) | 95.928484(10) | −0.0000093753994(5) |
| 12.0 | −0.5556094183824(2) | −1.111106750184(5) | 47.706156(4) | 0.0000093405484(3) |
| 13.0 | −0.55559818668317(10) | −1.111043171085(3) | 26.881845(10) | 0.0000117847909(2) |
| 14.0 | −0.55558722244837(6) | −1.111036302095(2) | 17.665346(3) | 0.00000986734301(7) |
| 15.0 | −0.55557861625837(4) | −1.1110465948261(10) | 13.266111(2) | 0.00000737584605(3) |
| 16.0 | −0.55557232288398(4) | −1.1110597914484(7) | 10.862844(3) | 0.00000530339498(2) |
| 17.0 | −0.55556782624247(3) | −1.1110714817502(4) | 9.313753(2) | 0.000003774749106(3) |
| 18.0 | −0.55556462424462(3) | −1.1110807713516(2) | 8.1634812(4) | 0.00000269317430(2) |
| 19.0 | −0.55556233179299(2) | −1.11108786405500(2) | 7.2296381(8) | 0.00000193681740(2) |
| 20.0 | −0.55556067537094(2) | −1.11109320801738(3) | 6.436203(3) | 0.000001407136212(10) |

TABLE S24. Calculated BO energies, expectation value of potential, $\langle\nabla_1\cdot\nabla_2\rangle$, and $\mathrm{d}E/\mathrm{d}R$ of the $2^1\Delta_u$ state in atomic units (hartree). Uncertainties originate purely from extrapolation to the complete basis set limit. United atom values at $R=0$ are taken from Ref. [1].

| $2^1\Delta_\mathrm{u}$ | | | | |
|---|---|---|---|---|
| $R$ | $E$ | $\langle V\rangle$ | $10^6\cdot\langle\nabla_1\cdot\nabla_2\rangle$ | $\mathrm{d}E/\mathrm{d}R$ |
| 0.0 | −2.0200029371587427(5) | – | 5.7042946(4) | – |
| 0.01 | 97.9802584250(2) | 95.9610343042(7) | 5.71(2) | −9999.94825457(5) |
| 0.05 | 17.986020428(3) | 15.98347205(2) | 5.728(10) | −399.7713762(3) |
| 0.1 | 8.001754885(6) | 6.04261216(4) | 5.88(3) | −99.6089761(3) |
| 0.15 | 4.690941940(4) | 2.79059070(2) | 6.03(5) | −43.94195451(9) |
| 0.2 | 3.051376373(3) | 1.21799389(2) | 6.415(4) | −24.42379425(5) |
| 0.3 | 1.446625532(2) | −0.245415170(7) | 7.173(8) | −10.46222078(2) |
| 0.4 | 0.6792417239(6) | −0.876167283(3) | 8.12(2) | −5.586626827(5) |
| 0.5 | 0.2450071975(3) | −1.185670290(2) | 9.308(2) | −3.351369370(3) |
| 0.6 | −0.0248235261(2) | −1.3443627192(9) | 10.6164(3) | −2.1578594450(10) |
| 0.7 | −0.2026310824(2) | −1.4241347733(10) | 12.098(6) | −1.4555322979(10) |
| 0.8 | −0.32448720197(10) | −1.4597980084(10) | 13.768(6) | −1.0135295057(9) |
| 0.9 | −0.41027855831(6) | −1.469802597(2) | 15.634(7) | −0.7213838676(9) |
| 1.0 | −0.47179545330(10) | −1.464564349(2) | 17.711(8) | −0.5209734423(10) |
| 1.1 | −0.51642219173(7) | −1.450239404(2) | 20.013(9) | −0.3794500184(10) |
| 1.2 | −0.5489861580(2) | −1.430591744(2) | 22.561(9) | −0.2771828570(2) |
| 1.3 | −0.5727536989(2) | −1.407980691(2) | 25.374(4) | −0.201902533(2) |
| 1.4 | −0.5899981953(2) | −1.383911100(3) | 28.4756(7) | −0.145653364(2) |
| 1.5 | −0.6023396232(2) | −1.359353116(3) | 31.81(6) | −0.103115913(2) |
| 1.6 | −0.61095556851(6) | −1.334934547(3) | 35.646(5) | −0.070639631(2) |
| 1.7 | −0.6167167331(2) | −1.311059981(3) | 39.74(3) | −0.045662656(2) |
| 1.8 | −0.62027643075(4) | −1.287986357(4) | 44.328(9) | −0.026351942(2) |
| 1.9 | −0.62213114877(2) | −1.265871891(4) | 49.335(5) | −0.011373470(2) |
| 2.0 | −0.62266241179(3) | −1.244808306(4) | 54.846(10) | 0.000258259(2) |
| 2.1 | −0.62216626631(3) | −1.224842369(4) | 60.918(10) | 0.009281030(2) |
| 2.2 | −0.62087439576(5) | −1.205990450(5) | 67.611(10) | 0.016253792(2) |
| 2.3 | −0.61896946815(6) | −1.188248471(5) | 74.998(3) | 0.021604550(2) |
| 2.4 | −0.61659644175(10) | −1.171598736(5) | 83.153(4) | 0.025664228(2) |
| 2.5 | −0.6138709943(2) | −1.156014657(6) | 92.170(3) | 0.028690933(2) |
| 2.6 | −0.6108858770(2) | −1.141464022(6) | 102.137(10) | 0.030887589(2) |
| 2.7 | −0.60771575189(5) | −1.127911266(7) | 113.21(2) | 0.032414903(3) |
| 2.8 | −0.60442090900(5) | −1.115319028(7) | 125.502(6) | 0.033400997(3) |
| 2.9 | −0.60105014550(5) | −1.103649227(8) | 139.168(6) | 0.033948643(3) |
| 3.0 | −0.59764301454(3) | −1.092863796(8) | 154.381(10) | 0.034140744(3) |
| 3.1 | −0.59423159359(4) | −1.082925172(9) | 171.384(9) | 0.034044521(3) |
| 3.2 | −0.59084188475(4) | −1.073796630(9) | 190.35(5) | 0.033714731(3) |
| 3.3 | −0.58749493087(6) | −1.065442509(10) | 211.7347(5) | 0.033196168(3) |
| 3.4 | −0.58420771064(4) | −1.057828379(9) | 235.701(7) | 0.032525601(3) |
| 3.5 | −0.5809938625(2) | −1.05092118(2) | 262.7296(10) | 0.031733298(3) |
| 3.6 | −0.5778642720(2) | −1.04468937(2) | 293.267(3) | 0.030844215(3) |
| 3.7 | −0.57482755547(4) | −1.03910310(2) | 327.876(4) | 0.029878922(3) |
| 3.8 | −0.57189046072(4) | −1.03413449(2) | 367.0(2) | 0.028854324(4) |
| 3.9 | −0.56905820467(4) | −1.02975800(2) | 412.11(8) | 0.027784208(4) |
| 4.0 | −0.56633476490(5) | −1.02595101(2) | 463.707(3) | 0.026679629(3) |
| 4.1 | −0.5637231394(8) | −1.02269474(2) | 522.975(4) | 0.025549155(3) |

| $2^1\Delta_u$ continued | | | | |
|---|---|---|---|---|
| $R$ | $E$ | $\langle V\rangle$ | $10^6\cdot\langle\nabla_1\cdot\nabla_2\rangle$ | $\mathrm{d}E/\mathrm{d}R$ |
| 4.2 | −0.5612255888(9) | −1.01997557(2) | 591.4735(6) | 0.024398954(4) |
| 4.3 | −0.558843881(2) | −1.01778716(3) | 670.957(2) | 0.023232698(6) |
| 4.4 | −0.556579553(2) | −1.01613380(3) | 763.611(6) | 0.022051205(6) |
| 4.5 | −0.5544342336(4) | −1.01503575(4) | 871.919(4) | 0.020851714(8) |
| 4.6 | −0.552410057(2) | −1.01453785(4) | 998.66(3) | 0.019626580(8) |
| 4.7 | −0.550510252(3) | −1.01472351(6) | 1146.44(2) | 0.01836106(2) |
| 4.8 | −0.548740018(3) | −1.01573692(6) | 1316.34(2) | 0.01702982(2) |
| 4.9 | −0.547107820(4) | −1.01781520(9) | 1504.60(5) | 0.01559193(2) |
| 5.0 | −0.5456271965(2) | −1.0213220(2) | 1694.79(3) | 0.01398648(3) |
| 5.1 | −0.5443186361(10) | −1.02673184(3) | 1841.454(5) | 0.012138319(5) |
| 5.2 | −0.543209274(2) | −1.03440445(4) | 1846.834(5) | 0.010002712(7) |
| 5.3 | −0.542324503(2) | −1.04391901(5) | 1561.970(5) | 0.007684905(8) |
| 5.4 | −0.541666251(3) | −1.05334652(5) | 879.629(5) | 0.005552960(8) |
| 5.5 | −0.54119190728(7) | −1.06000091(2) | −119.2819(8) | 0.004069618(3) |
| 5.6 | −0.540824448(3) | −1.06255765(3) | −1190.551(4) | 0.003409150(5) |
| 5.7 | −0.540488775(3) | −1.06168831(2) | −2111.479(4) | 0.003384077(3) |
| 5.8 | −0.540136970(2) | −1.05892056(2) | −2780.598(3) | 0.003681618(2) |
| 5.9 | −0.539750144(2) | −1.055591451(9) | −3197.414(3) | 0.0040523452(10) |
| 6.0 | −0.53932875809(2) | −1.0525079096(6) | −3410.568(4) | 0.00435826778(6) |
| 6.5 | −0.53706500341(2) | −1.0459524996(7) | −3120.9978(3) | 0.00433500112(7) |
| 7.0 | −0.53516264823(2) | −1.0476809760(6) | −2413.6087(2) | 0.00323490293(7) |
| 7.5 | −0.53381654251(2) | −1.0512110784(6) | −1789.4912(2) | 0.00218960088(6) |
| 8.0 | −0.53292651986(2) | −1.0545151815(6) | −1275.7014(2) | 0.00141723228(6) |
| 8.5 | −0.532356879819(10) | −1.0570783293(6) | −871.4457(2) | 0.00089828592(5) |
| 9.0 | −0.531997121138(10) | −1.0588975861(5) | −569.2333(2) | 0.00056629513(5) |
| 9.5 | −0.531769855665(10) | −1.0601266972(5) | −353.9179(2) | 0.00035926464(4) |
| 10.0 | −0.531624732783(10) | −1.0609345138(5) | −206.6814(2) | 0.00023149518(4) |
| 11.0 | −0.531467232329(8) | −1.0617971680(4) | −46.4463(2) | 0.00010339061(3) |
| 12.0 | −0.531393202225(7) | −1.0621616214(4) | 18.39651(10) | 0.00005206526(3) |
| 13.0 | −0.531353596798(7) | −1.0623155779(3) | 41.64360(9) | 0.00003012428(2) |
| 14.0 | −0.531329076802(6) | −1.0623767103(3) | 45.56992(8) | 0.00002010309(2) |
| 15.0 | −0.531311891879(5) | −1.0624029108(3) | 41.70288(8) | 0.000014724867(10) |
| 16.0 | −0.531299010885(6) | −1.0624180411(3) | 35.76210(8) | 0.00001124879(2) |
| 17.0 | −0.531289073605(4) | −1.0624293881(2) | 29.93463(6) | 0.000008750536(7) |
| 18.0 | −0.531281304700(4) | −1.0624389031(2) | 24.88175(6) | 0.000006872572(5) |
| 19.0 | −0.531275183021(3) | −1.0624471402(2) | 20.70012(5) | 0.000005432939(4) |
| 20.0 | −0.531270331255(3) | −1.06245432054(9) | 17.30076(5) | 0.000004317099(3) |

TABLE S25. Calculated BO energies, expectation value of potential, $\langle \nabla_1 \cdot \nabla_2 \rangle$, and $\mathrm{d}E/\mathrm{d}R$ of the $3^1\Delta_u$ state in atomic units (hartree). Uncertainties originate purely from extrapolation to the complete basis set limit. United atom values at $R = 0$ are taken from Ref. [1].

| $3^1\Delta_\mathrm{u}$ | | | | |
|---|---|---|---|---|
| $R$ | $E$ | $\langle V \rangle$ | $10^6 \cdot \langle \nabla_1 \cdot \nabla_2 \rangle$ | $\mathrm{d}E/\mathrm{d}R$ |
| 0.0 | −2.0138906838155497(3) | − | 3.482257(7) | − |
| 0.01 | 97.9863706789(2) | 95.973258814(2) | 3.4845(9) | −9999.94825443(8) |
| 0.05 | 17.992132698(6) | 15.99569663(4) | 3.520(2) | −399.7713753(6) |
| 0.1 | 8.00786719(2) | 6.05483686(7) | 3.616(2) | −99.6089751(5) |
| 0.15 | 4.697054287(9) | 2.80281557(6) | 3.760(2) | −43.9419534(3) |
| 0.2 | 3.057488778(6) | 1.23021897(4) | 3.944(2) | −24.4237929(2) |
| 0.3 | 1.452738091(3) | −0.23318953(2) | 4.410(2) | −10.46221904(4) |
| 0.4 | 0.685354474(8) | −0.86394094(5) | 4.994(2) | −5.58662473(8) |
| 0.5 | 0.251120177(5) | −1.17344310(4) | 5.684(3) | −3.35136692(5) |
| 0.6 | −0.018710282(2) | −1.33213454(2) | 6.480(2) | −2.15785663(2) |
| 0.7 | −0.196517540(3) | −1.41190546(2) | 7.386(3) | −1.45552912(3) |
| 0.8 | −0.3183733219(10) | −1.447567399(9) | 8.403(3) | −1.013525944(8) |
| 0.9 | −0.404164302(3) | −1.45757051(2) | 9.542(4) | −0.72137990(2) |
| 1.0 | −0.4656807788(3) | −1.452330595(2) | 10.805(3) | −0.520969038(2) |
| 1.1 | −0.5103070537(3) | −1.438003765(3) | 12.207(3) | −0.379445143(2) |
| 1.2 | −0.5428705074(3) | −1.418353981(3) | 13.757(3) | −0.277177472(2) |
| 1.3 | −0.5666374826(4) | −1.395740536(3) | 15.466(3) | −0.201896593(2) |
| 1.4 | −0.5838813553(4) | −1.371668256(4) | 17.350(4) | −0.145646818(2) |
| 1.5 | −0.5962220960(5) | −1.347107249(4) | 19.423(4) | −0.103108704(2) |
| 1.6 | −0.6048372847(5) | −1.322685279(5) | 21.68(2) | −0.070631694(3) |
| 1.7 | −0.6105976163(6) | −1.298806888(5) | 24.17(3) | −0.045653915(3) |
| 1.8 | −0.6141563963(6) | −1.275728957(6) | 26.95(2) | −0.026342314(3) |
| 1.9 | −0.6160101034(7) | −1.253609638(7) | 29.94(5) | −0.011362859(3) |
| 2.0 | −0.6165402518(7) | −1.232540580(8) | 33.30(3) | 0.000269962(3) |
| 2.1 | −0.6160428765(8) | −1.212568460(8) | 36.96(3) | 0.009293949(4) |
| 2.2 | −0.6147496477(9) | −1.193709550(9) | 41.030(10) | 0.016268066(4) |
| 2.3 | −0.6128432184(9) | −1.175959654(10) | 45.47(5) | 0.021620340(4) |
| 2.4 | −0.6104685299(10) | −1.15930094(2) | 50.37(4) | 0.025681716(4) |
| 2.5 | −0.6077412403(10) | −1.14370666(2) | 55.80(3) | 0.028710327(4) |
| 2.6 | −0.604754079(2) | −1.12914443(2) | 61.83(2) | 0.030909126(5) |
| 2.7 | −0.601581682(2) | −1.11557846(2) | 68.494(9) | 0.032438854(5) |
| 2.8 | −0.598284310(2) | −1.10297114(2) | 75.890(2) | 0.033427673(5) |
| 2.9 | −0.594910728(2) | −1.09128409(2) | 84.08(3) | 0.033978401(5) |
| 3.0 | −0.591500451(2) | −1.08047892(2) | 93.23(3) | 0.034173994(5) |
| 3.1 | −0.588085511(2) | −1.07051765(2) | 103.45(2) | 0.034081734(5) |
| 3.2 | −0.584691860(2) | −1.06136308(2) | 114.900(8) | 0.033756452(5) |
| 3.3 | −0.581340483(2) | −1.05297898(2) | 127.732(2) | 0.033243025(5) |
| 3.4 | −0.578048291(2) | −1.04533028(2) | 142.164(10) | 0.032578325(5) |
| 3.5 | −0.574828842(2) | −1.03838311(3) | 158.463(10) | 0.031792736(5) |
| 3.6 | −0.571692932(2) | −1.03210500(3) | 176.92(2) | 0.030911351(6) |
| 3.7 | −0.568649070(2) | −1.02646500(3) | 197.90(2) | 0.029954902(6) |
| 3.8 | −0.565703880(2) | −1.02143393(3) | 221.845(10) | 0.028940481(6) |
| 3.9 | −0.562862436(2) | −1.01698475(3) | 249.289(9) | 0.027882083(6) |
| 4.0 | −0.560128550(2) | −1.01309315(3) | 280.898(8) | 0.026790987(6) |
| 4.1 | −0.557505033(2) | −1.00973856(3) | 317.488(7) | 0.025675978(7) |
| 4.2 | −0.554993938(2) | −1.00690571(4) | 360.077(5) | 0.024543373(8) |
| 4.3 | −0.552596820(2) | −1.00458743(4) | 409.89(3) | 0.023396792(9) |
| 4.4 | −0.550315030(2) | −1.00278941(4) | 468.48(2) | 0.022236511(9) |
| 4.5 | −0.548150116(3) | −1.00153902(7) | 537.46(4) | 0.02105805(2) |
| 4.6 | −0.546104413(4) | −1.00090155(8) | 618.48(4) | 0.01984941(2) |
| 4.7 | −0.544182053(4) | −1.0010124(2) | 711.72(5) | 0.01858546(3) |
| 4.8 | −0.542390760(6) | −1.0021402(2) | 812.62(7) | 0.01721694(3) |
| 4.9 | −0.540745177(7) | −1.0048019(3) | 900.96(6) | 0.01565070(4) |
| 5.0 | −0.53927242(2) | −1.0098994(6) | 910.5(4) | 0.0137291(2) |

| $3^1\Delta_u$ continued | | | | |
|---|---|---|---|---|
| $R$ | $E$ | $\langle V \rangle$ | $10^6 \cdot \langle \nabla_1 \cdot \nabla_2 \rangle$ | $\mathrm{d}E/\mathrm{d}R$ |
| 5.1 | −0.538016806(7) | −1.0184245(2) | 673.69(4) | 0.01129591(4) |
| 5.2 | −0.537022853(9) | −1.0292670(3) | −53.08(4) | 0.00861128(4) |
| 5.3 | −0.536266717(10) | −1.0367730(2) | −1184.57(4) | 0.00674725(3) |
| 5.4 | −0.535621928(9) | −1.03684041(3) | −2142.23(4) | 0.006371009(3) |
| 5.5 | −0.534963991(7) | −1.03225380(3) | −2570.29(3) | 0.006849846(7) |
| 5.6 | −0.534251065(5) | −1.02720191(4) | −2568.51(3) | 0.007375035(8) |
| 5.7 | −0.533498616(4) | −1.02355641(3) | −2351.60(2) | 0.007621194(6) |
| 5.8 | −0.532736666(3) | −1.02154336(3) | −2057.460(10) | 0.007574132(5) |
| 5.9 | −0.531991304(2) | −1.02090673(2) | −1743.876(6) | 0.007300995(4) |
| 6.0 | −0.5312820635(4) | −1.021410847(5) | −1425.0905(4) | 0.0068588798(9) |
| 6.5 | −0.5288103544(2) | −1.04245138(2) | 512.7440(4) | 0.002333743(2) |
| 7.0 | −0.5288765327(2) | −1.068388550(2) | 1194.3729(4) | −0.0015193550(3) |
| 7.5 | −0.5296762085(2) | −1.070450782(2) | 788.0294(6) | −0.0014797819(2) |
| 8.0 | −0.53030077042(6) | −1.0687730069(5) | 492.4044(3) | −0.00102143326(5) |
| 8.5 | −0.53071413808(4) | −1.0669769046(4) | 307.7319(3) | −0.00065277982(3) |
| 9.0 | −0.53097318465(3) | −1.0655538013(3) | 192.2463(3) | −0.00040082577(2) |
| 9.5 | −0.53112974957(2) | −1.0645175269(2) | 120.1860(2) | −0.000237687133(9) |
| 10.0 | −0.53122092310(2) | −1.06379300113(8) | 75.64031(10) | −0.000135115493(6) |
| 11.0 | −0.531297076365(7) | −1.06296751572(5) | 30.98206(6) | −0.000033942090(3) |
| 12.0 | −0.53131019485(2) | −1.0626058774(2) | 11.0989(2) | 0.000001209356(10) |
| 13.0 | −0.531302926288(5) | −1.06246509850(5) | 0.50351(4) | 0.000010827237(3) |
| 14.0 | −0.531291562605(5) | −1.06242762606(4) | −3.79490(5) | 0.000011107082(2) |
| 15.0 | −0.531281477286(4) | −1.06242881069(3) | −4.68382(5) | 0.0000089429252(10) |
| 16.0 | −0.531273682281(3) | −1.06244004176(2) | −4.35421(4) | 0.0000067076753(6) |
| 17.0 | −0.531267903022(3) | −1.062451914015(9) | −3.71557(4) | 0.0000049348253(3) |
| 18.0 | −0.531263656125(2) | −1.062461991741(6) | −3.07409(4) | 0.0000036289172(2) |
| 19.0 | −0.531260523877(2) | −1.062469989263(4) | −2.51771(3) | 0.00000268728899(6) |
| 20.0 | −0.5312581938707(8) | −1.062476197047(2) | −2.05942(3) | 0.00000200953471(2) |

TABLE S26. Calculated BO energies, expectation value of potential, $\langle\nabla_1\cdot\nabla_2\rangle$, and $\mathrm{d}E/\mathrm{d}R$ of the $1^3\Delta_u$ state in atomic units (hartree). Uncertainties originate purely from extrapolation to the complete basis set limit. United atom values at $R=0$ are taken from Ref. [1].

| $1^3\Delta_\mathrm{u}$ | | | | |
|---|---|---|---|---|
| $R$ | $E$ | $\langle V\rangle$ | $10^6\cdot\langle\nabla_1\cdot\nabla_2\rangle$ | $\mathrm{d}E/\mathrm{d}R$ |
| 0.0 | −2.031255144381749(1) | – | 9.6696396 | – |
| 0.01 | 97.9690061972(7) | 95.938522(5) | 9.67(2) | −9999.9490(5) |
| 0.05 | 17.974768177(3) | 15.9609670(4) | 9.763(9) | −399.771387(9) |
| 0.1 | 7.990502571(4) | 6.0201070(4) | 10.026(9) | −99.608983(5) |
| 0.15 | 4.679689534(3) | 2.76808560(7) | 10.42540(2) | −43.9419565(3) |
| 0.2 | 3.040123847(2) | 1.1954878(5) | 10.922(10) | −24.423800(3) |
| 0.3 | 1.4353726991(6) | −0.2679225(5) | 12.20(2) | −10.462226(2) |
| 0.4 | 0.6679885115(2) | −0.8986760(6) | 13.79(2) | −5.586633(2) |
| 0.5 | 0.2337535344(2) | −1.2081808(7) | 15.68(2) | −3.351376(2) |
| 0.6 | −0.03607770954(10) | −1.3668744214(6) | 17.859(2) | −2.1578650039(7) |
| 0.7 | −0.213885857835(6) | −1.4466487259(5) | 20.329(2) | −1.4555385861(5) |
| 0.8 | −0.335742644206(3) | −1.48231453851(9) | 23.1102(7) | −1.01353656262(9) |
| 0.9 | −0.421534746601(4) | −1.4923220623(2) | 26.215(2) | −0.7213917434(2) |
| 1.0 | −0.483052472506(3) | −1.4870871424(2) | 29.674(2) | −0.5209821974(2) |
| 1.1 | −0.527680133189(3) | −1.4727659616(2) | 33.511(2) | −0.3794597229(2) |
| 1.2 | −0.560245120680(3) | −1.4531225511(2) | 37.7655(9) | −0.2771935915(2) |
| 1.3 | −0.584013790252(5) | −1.4305162866(2) | 42.4725(2) | −0.2019143893(2) |
| 1.4 | −0.601259532509(2) | −1.4064520884(2) | 47.6749(6) | −0.14566644528(9) |
| 1.5 | −0.613602334566(2) | −1.3819001758(2) | 53.4251(6) | −0.10313033778(8) |
| 1.6 | −0.622219794846(2) | −1.3574884401(2) | 59.7800(2) | −0.07065553152(8) |
| 1.7 | −0.627982629417(2) | −1.3336215674(2) | 66.8034(6) | −0.04568018150(8) |
| 1.8 | −0.631544167799(2) | −1.3105566082(2) | 74.5703(2) | −0.02637126257(7) |
| 1.9 | −0.633400915489(2) | −1.2884519077(2) | 83.1631(4) | −0.01139477725(7) |
| 2.0 | −0.6339344174044(8) | −1.2673993366(2) | 92.6771(6) | 0.00023474908(7) |
| 2.1 | −0.633440743036(2) | −1.2474458305(2) | 103.2210(2) | 0.00925507409(6) |
| 2.2 | −0.632151601801(2) | −1.2286079564(2) | 114.9162(2) | 0.01622511234(6) |
| 2.3 | −0.63024969107(2) | −1.2108818591(2) | 127.90297(8) | 0.02157283612(6) |
| 2.4 | −0.627880002297(2) | −1.1942501003(2) | 142.3400660(10) | 0.02562912680(5) |
| 2.5 | −0.625158250729(2) | −1.1786863871(2) | 158.40868(5) | 0.02865204574(5) |
| 2.6 | −0.622177229955(2) | −1.1641588483(2) | 176.315952(5) | 0.03084446601(5) |
| 2.7 | −0.619011650005(2) | −1.1506323054(2) | 196.29833(6) | 0.03236703505(5) |
| 2.8 | −0.615721854827(2) | −1.1380698436(2) | 218.62686(8) | 0.03334780932(5) |
| 2.9 | −0.6123567027750(10) | −1.1264338930(3) | 243.61238(2) | 0.03388948710(7) |
| 3.0 | −0.608955815994(2) | −1.1156869681(2) | 271.61185(10) | 0.03407488797(5) |
| 3.1 | −0.605551349778(2) | −1.1057921712(2) | 303.0369(2) | 0.03397113816(5) |
| 3.2 | −0.602169393902(2) | −1.0967135337(2) | 338.3626(3) | 0.03363289189(5) |
| 3.3 | −0.598831089842(3) | −1.0884162526(3) | 378.1391(3) | 0.03310482637(6) |
| 3.4 | −0.595553527284(3) | −1.0808668639(3) | 423.0052(2) | 0.03242358550(6) |
| 3.5 | −0.592350468349(3) | −1.0740333859(3) | 473.7049(3) | 0.03161930023(6) |
| 3.6 | −0.589232936864(2) | −1.0678854621(3) | 531.1085(3) | 0.03071678100(7) |
| 3.7 | −0.5862097017438(7) | −1.0623945276(3) | 596.2369(3) | 0.02973645295(7) |
| 3.8 | −0.583287677482(3) | −1.0575340266(4) | 670.2926(4) | 0.02869508640(8) |
| 3.9 | −0.580472260143(2) | −1.0532797109(4) | 754.6982(4) | 0.02760636137(8) |
| 4.0 | −0.577767614025(2) | −1.0496100525(5) | 851.1424(4) | 0.02648129388(9) |
| 4.1 | −0.57517692178(4) | −1.0465068186(7) | 961.6374(3) | 0.0253285427(2) |
| 4.2 | −0.57270260933(5) | −1.0439558647(7) | 1088.5875(6) | 0.0241546081(2) |
| 4.3 | −0.57034655613(5) | −1.0419482315(9) | 1234.870(2) | 0.0229639258(2) |
| 4.4 | −0.56811030137(6) | −1.0404816429(10) | 1403.9309(5) | 0.0217588545(3) |
| 4.5 | −0.5659952569707(9) | −1.039562543(2) | 1599.8717(6) | 0.0205395491(3) |
| 4.6 | −0.56400293958(7) | −1.039208820(2) | 1827.5351(6) | 0.0193037085(3) |
| 4.7 | −0.56213523395(8) | −1.039453341(2) | 2092.5193(8) | 0.0180461972(4) |
| 4.8 | −0.56039469994(9) | −1.040348290(2) | 2401.0474(9) | 0.0167585646(4) |
| 4.9 | −0.55878492842(10) | −1.041969841(3) | 2759.515(2) | 0.0154285748(5) |
| 5.0 | −0.557310932621(2) | −1.044421656(3) | 3173.415(2) | 0.0140400418(5) |

| $1^3\Delta_u$ continued | | | | |
|---|---|---|---|---|
| $R$ | $E$ | $\langle V \rangle$ | $10^6 \cdot \langle \nabla_1 \cdot \nabla_2 \rangle$ | $\mathrm{d}E/\mathrm{d}R$ |
| 5.1 | −0.5559795149(4) | −1.04783343(2) | 3644.9(3) | 0.012573648(3) |
| 5.2 | −0.5547994504(3) | −1.05234669(2) | 4170.0(3) | 0.011010040(3) |
| 5.3 | −0.5537811750(3) | −1.058076179(8) | 4731.8(3) | 0.009337013(2) |
| 5.4 | −0.5529354845(2) | −1.065035853(6) | 5295.1(2) | 0.007562058(2) |
| 5.5 | −0.552270801744(5) | −1.073040750(5) | 5805.6(2) | 0.0057274279(9) |
| 5.6 | −0.55178921992(10) | −1.081642333(3) | 6199.4(2) | 0.0039171619(6) |
| 5.7 | −0.55148284732(9) | −1.090184966(3) | 6424.6(2) | 0.0022422331(5) |
| 5.8 | −0.55133282504(8) | −1.098001533(2) | 6463.2(2) | 0.0008041581(4) |
| 5.9 | −0.55131214327(7) | −1.104628130(2) | 6335.4(2) | −0.0003396345(3) |
| 6.0 | −0.551390765309(2) | −1.10989234515(6) | 6085.1296(2) | −0.001185135754(7) |
| 6.5 | −0.552445964036(2) | −1.12075438028(9) | 4335.37950(10) | −0.00244037726(2) |
| 7.0 | −0.5535618672438(8) | −1.12069717962(5) | 2986.8741(2) | −0.001939063589(6) |
| 7.5 | −0.5543687420831(5) | −1.11852767170(3) | 2114.45541(5) | −0.001305358338(4) |
| 8.0 | −0.5548932494056(5) | −1.11635517878(3) | 1539.98381(5) | −0.000821084996(3) |
| 8.5 | −0.5552161581127(3) | −1.11462915363(2) | 1150.57100(3) | −0.000493745577(2) |
| 9.0 | −0.5554066658714(3) | −1.11337450547(2) | 880.667066(10) | −0.000284574858(2) |
| 9.5 | −0.5555140718032(3) | −1.11250801819(2) | 690.37336(2) | −0.0001557762721(9) |
| 10.0 | −0.5555710538164(2) | −1.111931605329(9) | 554.136254(10) | −0.0000789497696(6) |
| 11.0 | −0.5556089487667(2) | −1.111328746937(7) | 381.542549572(6) | −0.0000100772184(5) |
| 12.0 | −0.5556073253122(2) | −1.111109129406(5) | 282.851826(4) | 0.0000087934349(3) |
| 13.0 | −0.55559657674945(8) | −1.111045458700(3) | 220.9128920(10) | 0.0000113611384(2) |
| 14.0 | −0.55558598493495(7) | −1.111038377196(3) | 178.4156600(3) | 0.00000954233391(9) |
| 15.0 | −0.55557766341943(4) | −1.111048403025(2) | 147.17447(2) | 0.00000712825429(4) |
| 16.0 | −0.55557158647196(3) | −1.1110613254747(7) | 123.129210(2) | 0.00000511546683(2) |
| 17.0 | −0.55556725402419(2) | −1.1110727609832(3) | 104.088093(8) | 0.000003632180311287(10) |
| 18.0 | −0.55556417668809(2) | −1.1110818270817(2) | 88.737289(7) | 0.000002584794136(3) |
| 19.0 | −0.55556197917279(2) | −1.1110887305460(2) | 76.208782(3) | 0.000001854094711(6) |
| 20.0 | −0.555560395394540(9) | −1.111093917775096(3) | 65.886691(2) | 0.000001343650688(8) |

TABLE S27. Calculated BO energies, expectation value of potential, $\langle\nabla_1 \cdot \nabla_2\rangle$, and $\mathrm{d}E/\mathrm{d}R$ of the $2^3\Delta_u$ state in atomic units (hartree). Uncertainties originate purely from extrapolation to the complete basis set limit. United atom values at $R = 0$ are taken from Ref. [1].

| $2^3\Delta_\mathrm{u}$ | | | | |
|---|---|---|---|---|
| $R$ | $E$ | $\langle V\rangle$ | $10^6 \cdot \langle\nabla_1 \cdot \nabla_2\rangle$ | $\mathrm{d}E/\mathrm{d}R$ |
| 0.0 | −2.0200029371587427(5) | – | 5.4064900(5) | – |
| 0.01 | 97.98025840474(10) | 95.9610342638(7) | 5.400(3) | −9999.94825457(5) |
| 0.05 | 17.986020408(3) | 15.98347201(2) | 5.35(6) | −399.7713762(3) |
| 0.1 | 8.001754864(7) | 6.04261212(4) | 5.45(8) | −99.6089760(3) |
| 0.15 | 4.690941918(4) | 2.79059065(2) | 5.80(2) | −43.94195454(9) |
| 0.2 | 3.051376349(3) | 1.21799384(2) | 6.08(2) | −24.42379428(7) |
| 0.3 | 1.446625504(2) | −0.245415237(7) | 6.79(3) | −10.46222082(2) |
| 0.4 | 0.6792416918(7) | −0.876167368(4) | 7.618(9) | −5.586626880(7) |
| 0.5 | 0.2450071597(3) | −1.185670396(2) | 8.730(2) | −3.351369432(3) |
| 0.6 | −0.0248235704(2) | −1.3443628501(10) | 9.9345(5) | −2.157859516(2) |
| 0.7 | −0.20263113416(9) | −1.4241349329(8) | 11.291(6) | −1.4555323780(8) |
| 0.8 | −0.32448726218(9) | −1.4597982005(7) | 12.821(6) | −1.0135295952(7) |
| 0.9 | −0.41027862788(8) | −1.4698028255(8) | 14.529(7) | −0.7213839664(7) |
| 1.0 | −0.47179553320(8) | −1.4645646166(9) | 16.429(8) | −0.5209735504(7) |
| 1.1 | −0.51642228284(9) | −1.4502397144(10) | 18.537(8) | −0.3794501353(7) |
| 1.2 | −0.54898626128(4) | −1.430592101(2) | 20.871(10) | −0.2771829823(7) |
| 1.3 | −0.57275381512(9) | −1.407981096(2) | 23.456(2) | −0.2019026664(8) |
| 1.4 | −0.58999832516(4) | −1.383911556(2) | 26.313(3) | −0.1456535042(8) |
| 1.5 | −0.6023397673(2) | −1.359353625(2) | 29.467(5) | −0.1031160600(9) |
| 1.6 | −0.6109557277(2) | −1.334935108(2) | 32.942(3) | −0.0706397832(10) |
| 1.7 | −0.6167169077(2) | −1.311060594(3) | 36.78(2) | −0.0456628114(10) |
| 1.8 | −0.62027662088(3) | −1.287987021(3) | 41.04(2) | −0.026352100(2) |
| 1.9 | −0.6221313547(3) | −1.265872604(3) | 45.787(3) | −0.011373629(2) |
| 2.0 | −0.6226626335(3) | −1.244809063(3) | 51.003(2) | 0.000258102(2) |
| 2.1 | −0.6221665036(2) | −1.224843164(4) | 56.793(3) | 0.009280877(2) |
| 2.2 | −0.62087464802(2) | −1.205991277(4) | 63.226(4) | 0.016253645(2) |
| 2.3 | −0.6189697346(3) | −1.188249319(4) | 70.370(9) | 0.021604413(2) |
| 2.4 | −0.6165967213(4) | −1.171599594(5) | 78.319(6) | 0.025664104(2) |
| 2.5 | −0.61387128547(7) | −1.156015509(5) | 87.1906(8) | 0.028690825(2) |
| 2.6 | −0.61088617795(6) | −1.141464851(6) | 97.076(6) | 0.030887502(2) |
| 2.7 | −0.60771606041(6) | −1.127912049(6) | 108.134(6) | 0.032414841(2) |
| 2.8 | −0.6044212223(5) | −1.115319740(7) | 120.517(7) | 0.033400966(2) |
| 2.9 | −0.60105045996(5) | −1.103649837(7) | 134.403(9) | 0.033948649(2) |
| 3.0 | −0.5976433263(4) | −1.092864268(7) | 149.997(10) | 0.034140795(2) |
| 3.1 | −0.5942318977(4) | −1.082925462(9) | 167.549(3) | 0.034044624(3) |
| 3.2 | −0.59084217558(5) | −1.073796685(9) | 187.340(4) | 0.033714896(3) |
| 3.3 | −0.58749520168(5) | −1.065442268(9) | 209.722(8) | 0.033196405(3) |
| 3.4 | −0.58420795369(5) | −1.057827768(10) | 235.06(2) | 0.032525923(3) |
| 3.5 | −0.58099406834(5) | −1.050920110(10) | 263.844(10) | 0.031733722(3) |
| 3.6 | −0.57786442972(2) | −1.04468773(2) | 296.612(9) | 0.030844758(3) |
| 3.7 | −0.57482765208(5) | −1.03910076(2) | 334.041(7) | 0.029879607(4) |
| 3.8 | −0.57189048062(5) | −1.03413128(2) | 376.915(8) | 0.028855179(4) |
| 3.9 | −0.56905812924(5) | −1.02975372(2) | 426.20(2) | 0.027785267(3) |
| 4.0 | −0.56633457162(4) | −1.02594540(2) | 483.089(2) | 0.026680935(4) |
| 4.1 | −0.5637228009(10) | −1.02268747(2) | 548.99(3) | 0.025550764(4) |
| 4.2 | −0.5612250713(10) | −1.01996620(2) | 625.75(3) | 0.024400938(4) |
| 4.3 | −0.558843142(2) | −1.01777514(3) | 715.52(3) | 0.023235150(6) |
| 4.4 | −0.556578541(2) | −1.01611839(4) | 821.03(3) | 0.022054247(7) |
| 4.5 | −0.55443288138(7) | −1.01501597(4) | 945.54(4) | 0.020855510(8) |
| 4.6 | −0.552408279(3) | −1.01451236(5) | 1092.89(4) | 0.019631347(10) |
| 4.7 | −0.550507937(3) | −1.01469059(6) | 1267.09(5) | 0.01836708(2) |
| 4.8 | −0.548737024(3) | −1.01569440(8) | 1471.16(5) | 0.01703743(2) |
| 4.9 | −0.547103972(4) | −1.01776075(10) | 1703.80(6) | 0.01560147(2) |
| 5.0 | −0.5456222913(2) | −1.0212544(2) | 1951.02(7) | 0.01399804(3) |

| $2^3\Delta_u$ continued | | | | |
|---|---|---|---|---|
| $R$ | $E$ | $\langle V \rangle$ | $10^6 \cdot \langle \nabla_1 \cdot \nabla_2 \rangle$ | $\mathrm{d}E/\mathrm{d}R$ |
| 5.1 | −0.5443125008(3) | −1.026654426(4) | 2168.1587(8) | 0.0121510932(5) |
| 5.2 | −0.5432019101(4) | −1.034332090(7) | 2251.1194(10) | 0.010013794(2) |
| 5.3 | −0.5423163386(5) | −1.043882162(10) | 2030.4070(10) | 0.007688776(2) |
| 5.4 | −0.5416582835(5) | −1.05337508(2) | 1366.2142(8) | 0.005544720(2) |
| 5.5 | −0.54118535897(9) | −1.060094589(9) | 320.3920(6) | 0.004050205(2) |
| 5.6 | −0.5408201582(6) | −1.062687141(7) | −848.8310(4) | 0.0033844956(10) |
| 5.7 | −0.5404869603(5) | −1.061821924(5) | −1887.7004(3) | 0.0033599994(7) |
| 5.8 | −0.5401373893(5) | −1.059039050(4) | −2669.3601(3) | 0.0036613326(4) |
| 5.9 | −0.5397523584(4) | −1.055687939(3) | −3180.5427(2) | 0.0040367420(3) |
| 6.0 | −0.53933231324(3) | −1.0525829857(9) | −3466.8979(2) | 0.00434694015(9) |
| 6.5 | −0.53707110149(2) | −1.0459742782(6) | −3331.4207(2) | 0.00433352690(6) |
| 7.0 | −0.535168928190(10) | −1.0476915121(5) | −2647.22195(9) | 0.00323519204(6) |
| 7.5 | −0.533822550330(8) | −1.0512176861(5) | −2017.61725(8) | 0.00219032194(5) |
| 8.0 | −0.532932119480(8) | −1.0545192649(5) | −1489.29614(7) | 0.00141812176(5) |
| 8.5 | −0.532362013692(8) | −1.0570804210(5) | −1066.85193(7) | 0.00089924781(4) |
| 9.0 | −0.532001768368(7) | −1.0588980901(4) | −745.18404(6) | 0.00056727185(4) |
| 9.5 | −0.531774019695(7) | −1.0601259994(4) | −510.55708(5) | 0.00036021474(4) |
| 10.0 | −0.531628435154(7) | −1.0609329979(4) | −345.09012(5) | 0.00023238724(3) |
| 11.0 | −0.531470123399(6) | −1.0617949711(3) | −153.75884(4) | 0.00010411597(3) |
| 12.0 | −0.531395443869(5) | −1.0621590777(3) | −64.80720(4) | 0.00005265084(2) |
| 13.0 | −0.531355299016(5) | −1.0623125574(3) | −20.85826(4) | 0.00003061851(2) |
| 14.0 | −0.531330336053(4) | −1.0623737718(2) | 0.88590(4) | 0.000020492880(2) |
| 15.0 | −0.531312811720(4) | −1.0624003621(2) | 10.63407(3) | 0.000015017422(9) |
| 16.0 | −0.531299677372(3) | −1.0624158907(2) | 14.54654(3) | 0.000011466501(7) |
| 17.0 | −0.53128955193(2) | −1.0624276037(2) | 15.79426(3) | 0.000008911773(6) |
| 18.0 | −0.531281644216(3) | −1.06243745234(10) | 15.80708(2) | 0.000006990894(4) |
| 19.0 | −0.531275421228(3) | −1.06244598589(9) | 15.22318(2) | 0.000005518767(4) |
| 20.0 | −0.531270496395(2) | −1.06245342067(7) | 14.34616(2) | 0.000004378607(3) |

TABLE S28. Calculated BO energies, expectation value of potential, $\langle\nabla_1 \cdot \nabla_2\rangle$, and $\mathrm{d}E/\mathrm{d}R$ of the $3^3\Delta_u$ state in atomic units (hartree). Uncertainties originate purely from extrapolation to the complete basis set limit. United atom values at $R = 0$ are taken from Ref. [1].

| $3^3\Delta_\mathrm{u}$ | | | | |
|---|---|---|---|---|
| $R$ | $E$ | $\langle V\rangle$ | $10^6 \cdot \langle\nabla_1 \cdot \nabla_2\rangle$ | $\mathrm{d}E/\mathrm{d}R$ |
| 0.0 | −2.0138906838155497(3) | − | 3.2684586(8) | − |
| 0.01 | 97.9863706646(5) | 95.973258786(4) | 3.2687(4) | −9999.9482544(3) |
| 0.05 | 17.99213269(2) | 15.99569665(9) | 3.297(2) | −399.771375(2) |
| 0.1 | 8.00786718(4) | 6.0548369(2) | 3.384(3) | −99.608975(2) |
| 0.15 | 4.69705428(4) | 2.8028156(2) | 3.515(3) | −43.9419533(9) |
| 0.2 | 3.05748876(3) | 1.2302189(2) | 3.682(3) | −24.4237929(5) |
| 0.3 | 1.45273807(2) | −0.23318959(8) | 4.107(3) | −10.4622191(2) |
| 0.4 | 0.685354452(3) | −0.86394100(2) | 4.635(2) | −5.58662476(4) |
| 0.5 | 0.251120150(2) | −1.17344318(2) | 5.265(2) | −3.35136696(2) |
| 0.6 | −0.018710314(2) | −1.332134638(9) | 5.986(2) | −2.15785668(2) |
| 0.7 | −0.1965175762(5) | −1.411905576(5) | 6.74(4) | −1.455529177(5) |
| 0.8 | −0.3183733651(9) | −1.447567537(7) | 7.720(2) | −1.013526008(7) |
| 0.9 | −0.404164352(2) | −1.45757068(2) | 8.741(4) | −0.72137997(2) |
| 1.0 | −0.4656808360(2) | −1.452330787(2) | 9.885(3) | −0.520969115(2) |
| 1.1 | −0.5103071188(2) | −1.438003987(2) | 11.148(3) | −0.379445226(2) |
| 1.2 | −0.5428705811(3) | −1.418354235(2) | 12.547(4) | −0.277177561(2) |
| 1.3 | −0.5666375654(3) | −1.395740825(3) | 14.094(4) | −0.201896688(2) |
| 1.4 | −0.5838814477(3) | −1.371668580(3) | 15.803(4) | −0.145646918(2) |
| 1.5 | −0.5962221986(3) | −1.347107609(3) | 17.705(4) | −0.103108808(2) |
| 1.6 | −0.6048373977(4) | −1.322685677(4) | 19.7861(7) | −0.070631801(2) |
| 1.7 | −0.6105977400(4) | −1.298807321(4) | 21.4(4) | −0.045654024(2) |
| 1.8 | −0.6141565310(5) | −1.275729425(5) | 24.636(9) | −0.026342424(2) |
| 1.9 | −0.6160102490(5) | −1.253610139(5) | 27.44(4) | −0.011362969(3) |
| 2.0 | −0.6165404084(6) | −1.232541110(6) | 30.57(4) | 0.000269854(3) |
| 2.1 | −0.6160430437(6) | −1.212569015(7) | 34.06(3) | 0.009293844(3) |
| 2.2 | −0.6147498251(7) | −1.193710124(7) | 37.92(4) | 0.016267966(3) |
| 2.3 | −0.6128434054(7) | −1.175960240(8) | 42.259(3) | 0.021620248(3) |
| 2.4 | −0.6104687255(8) | −1.159301529(9) | 47.033(7) | 0.025681634(4) |
| 2.5 | −0.6077414435(9) | −1.143707244(10) | 52.376(2) | 0.028710257(4) |
| 2.6 | −0.6047542881(9) | −1.12914499(2) | 58.339(8) | 0.030909073(4) |
| 2.7 | −0.6015818955(10) | −1.11557898(2) | 64.97(5) | 0.032438820(4) |
| 2.8 | −0.5982845264(10) | −1.10297160(2) | 72.46(5) | 0.033427663(4) |
| 2.9 | −0.594910944(2) | −1.09128447(2) | 80.893(7) | 0.033978419(4) |
| 3.0 | −0.591500663(2) | −1.08047919(2) | 90.32(3) | 0.034174045(5) |
| 3.1 | −0.588085716(2) | −1.07051778(2) | 100.99(2) | 0.034081825(5) |
| 3.2 | −0.584692054(2) | −1.06136302(2) | 113.05(2) | 0.033756589(5) |
| 3.3 | −0.581340661(2) | −1.05297870(2) | 126.70(2) | 0.033243218(5) |
| 3.4 | −0.578048446(2) | −1.04532971(2) | 142.220(2) | 0.032578583(5) |
| 3.5 | −0.574828967(2) | −1.03838218(2) | 159.88(2) | 0.031793072(5) |
| 3.6 | −0.571693019(2) | −1.03210363(3) | 180.07(3) | 0.030911780(5) |
| 3.7 | −0.568649109(2) | −1.02646308(3) | 203.24(2) | 0.029955443(5) |
| 3.8 | −0.565703858(2) | −1.02143132(3) | 229.91(2) | 0.028941156(6) |
| 3.9 | −0.562862339(2) | −1.01698128(3) | 260.76(2) | 0.027882923(6) |
| 4.0 | −0.560128360(2) | −1.01308860(3) | 296.62(3) | 0.026792030(6) |
| 4.1 | −0.557504726(2) | −1.00973263(4) | 338.53(3) | 0.025677274(7) |
| 4.2 | −0.554993486(2) | −1.00689800(4) | 387.80(4) | 0.024544992(8) |
| 4.3 | −0.552596186(3) | −1.00457741(5) | 446.10(4) | 0.023398827(9) |
| 4.4 | −0.550314168(3) | −1.00277635(5) | 515.51(5) | 0.022239088(10) |
| 4.5 | −0.548148960(3) | −1.00152181(7) | 598.58(4) | 0.02106136(2) |
| 4.6 | −0.546102879(4) | −1.00087870(8) | 698.07(5) | 0.01985371(2) |
| 4.7 | −0.544180025(4) | −1.0009819(2) | 816.11(6) | 0.01859110(3) |
| 4.8 | −0.542388083(6) | −1.0020994(2) | 950.73(9) | 0.01722433(4) |
| 4.9 | −0.540741664(7) | −1.0047493(3) | 1084.92(9) | 0.01566000(5) |
| 5.0 | −0.53926793(2) | −1.0098416(7) | 1153.4(2) | 0.0137388(2) |

$3^3\Delta_u$ continued

| $R$ | $E$ | $\langle V \rangle$ | $10^6 \cdot \langle \nabla_1 \cdot \nabla_2 \rangle$ | $\mathrm{d}E/\mathrm{d}R$ |
|---|---|---|---|---|
| 5.1 | −0.538011562(7) | −1.0183961(2) | 973.95(4) | 0.01129943(4) |
| 5.2 | −0.537018090(9) | −1.0293351(3) | 251.49(4) | 0.00859636(4) |
| 5.3 | −0.536264444(10) | −1.0369413(2) | −981.61(4) | 0.00671463(2) |
| 5.4 | −0.535623036(9) | −1.03701510(3) | −2100.95(4) | 0.006339069(2) |
| 5.5 | −0.534967735(7) | −1.03237217(3) | −2664.83(3) | 0.006829687(7) |
| 5.6 | −0.534256245(5) | −1.02726386(4) | −2743.35(3) | 0.007365824(8) |
| 5.7 | −0.533504346(4) | −1.02358183(3) | −2563.04(2) | 0.007618745(6) |
| 5.8 | −0.532742439(3) | −1.02154790(3) | −2279.371(8) | 0.007575340(5) |
| 5.9 | −0.531996845(2) | −1.02089845(2) | −1961.418(5) | 0.007304277(4) |
| 6.0 | −0.531287199(3) | −1.02139241(4) | −1628.691(4) | 0.006863664(8) |
| 6.5 | −0.5288103574(3) | −1.04234278(2) | 550.8415(6) | 0.002350451(2) |
| 7.0 | −0.528871363(8) | −1.0683622(2) | 1526.12(5) | −0.00151707(2) |
| 7.5 | −0.52967112981(9) | −1.070450074(2) | 1127.7077(5) | −0.0014810420(2) |
| 8.0 | −0.53029637849(5) | −1.0687751634(4) | 799.3609(3) | −0.00102280080(4) |
| 8.5 | −0.53071038893(8) | −1.0669795932(7) | 580.6234(4) | −0.00065397827(6) |
| 9.0 | −0.53096999340(6) | −1.0655567568(5) | 433.9929(3) | −0.00040186334(4) |
| 9.5 | −0.53112704163(4) | −1.0645206448(4) | 334.0754(3) | −0.00023858542(3) |
| 10.0 | −0.53121863177(2) | −1.06379611019(8) | 264.94184(8) | −0.000135884666(6) |
| 11.0 | −0.531295431753(6) | −1.06297006623(5) | 180.70620(6) | −0.000034472975(4) |
| 12.0 | −0.531308992240(5) | −1.06260792904(5) | 131.68657(5) | 0.000000837953(3) |
| 13.0 | −0.531302051582(4) | −1.06246710374(4) | 97.26417(4) | 0.000010538417(3) |
| 14.0 | −0.531290936650(4) | −1.06242929274(3) | 72.98299(4) | 0.000010898611(2) |
| 15.0 | −0.531281024435(3) | −1.06243003137(2) | 56.70616(4) | 0.0000088011665(10) |
| 16.0 | −0.531273347667(3) | −1.06244094086(2) | 45.49577(4) | 0.0000066096545(6) |
| 17.0 | −0.531267651376(2) | −1.062452598588(9) | 37.32628(4) | 0.0000048649508(4) |
| 18.0 | −0.531263464297(2) | −1.062462525001(6) | 31.09463(4) | 0.0000035779774(2) |
| 19.0 | −0.5312603759944(9) | −1.062470409947(4) | 26.19586(4) | 0.00000264958115(10) |
| 20.0 | −0.5312580787056(7) | −1.062476531526(3) | 22.26884(3) | 0.00000198129426(5) |

TABLE S29. Calculated BO energies, expectation value of potential, $\langle\nabla_1\cdot\nabla_2\rangle$, and $\mathrm{d}E/\mathrm{d}R$ of the $1^1\Phi_g$ state in atomic units (hartree). Uncertainties originate purely from extrapolation to the complete basis set limit. United atom values at $R=0$ are taken from Ref. [1].

| $1^1\Phi_\mathrm{g}$ | | | | |
|---|---|---|---|---|
| $R$ | $E$ | $\langle V\rangle$ | $10^6\cdot\langle\nabla_1\cdot\nabla_2\rangle$ | $\mathrm{d}E/\mathrm{d}R$ |
| 0.0 | −2.02000071089858471(1) | – | 1.4044136 | – |
| 0.01 | 97.98026065229(4) | 95.9610387603(3) | 1.40491(2) | −9999.94825443(2) |
| 0.05 | 17.986022689(5) | 15.98347664(4) | 1.41551(2) | −399.7713747(5) |
| 0.1 | 8.001757228(5) | 6.04261707(3) | 1.44408(2) | −99.6089739(3) |
| 0.15 | 4.690944419(4) | 2.79059613(3) | 1.48486(2) | −43.94195138(10) |
| 0.2 | 3.051379028(2) | 1.21799999(2) | 1.53445(3) | −24.42379033(4) |
| 0.3 | 1.4466286553(7) | −0.245407304(4) | 1.65162(4) | −10.462215383(9) |
| 0.4 | 0.67924545612(9) | −0.8761571126(6) | 1.78444(3) | −5.5866200622(10) |
| 0.5 | 0.24501167300(2) | −1.18565729095(10) | 1.9275(3) | −3.3513612739(2) |
| 0.6 | −0.02481817450(2) | −1.34434636284(9) | 2.07768(4) | −2.1578500231(2) |
| 0.7 | −0.202624721746(3) | −1.4241145201(7) | 2.2338(2) | −1.4555215378(7) |
| 0.8 | −0.324479697169(2) | −1.4597732986(5) | 2.3954(2) | −1.0135173802(5) |
| 0.9 | −0.410269771048(2) | −1.4697728480(4) | 2.5626(2) | −0.7213703398(3) |
| 1.0 | −0.471785241159(2) | −1.4645289484(3) | 2.7362(2) | −0.5209584661(2) |
| 1.1 | −0.516410407148(2) | −1.4501977062(3) | 2.9172(2) | −0.3794335380(2) |
| 1.2 | −0.548972647468(2) | −1.4305430635(3) | 3.1074(2) | −0.2771648071(2) |
| 1.3 | −0.572738301733(2) | −1.4079242927(3) | 3.3088(2) | −0.2018828378(2) |
| 1.4 | −0.589980742602(2) | −1.3838461943(3) | 3.5240(2) | −0.1456319351(2) |
| 1.5 | −0.602319936689(2) | −1.3592788483(3) | 3.7564(2) | −0.1030926499(2) |
| 1.6 | −0.610933459043(2) | −1.3348499848(3) | 4.0100(2) | −0.0706144167(2) |
| 1.7 | −0.616691999088(3) | −1.3109641026(4) | 4.2893(2) | −0.0456353555(2) |
| 1.8 | −0.620248855993(3) | −1.2878780350(4) | 4.6001(2) | −0.0263224016(2) |
| 1.9 | −0.622100500664(3) | −1.2657498749(5) | 4.9489(2) | −0.0113415124(2) |
| 2.0 | −0.622628438589(3) | −1.2446712000(5) | 5.3435(2) | 0.0002928386(2) |
| 2.1 | −0.622128694291(3) | −1.2246886054(6) | 5.7930(2) | 0.0093184682(3) |
| 2.2 | −0.620832925877(3) | −1.2058182621(7) | 6.3080(2) | 0.0162943590(3) |
| 2.3 | −0.618923772129(4) | −1.1880558539(8) | 6.9007(2) | 0.0216485610(3) |
| 2.4 | −0.616546157515(4) | −1.1713834058(10) | 7.5855(2) | 0.0257120456(4) |
| 2.5 | −0.613815720701(4) | −1.155773998(2) | 8.3786(2) | 0.0287429774(4) |
| 2.6 | −0.610825167540(4) | −1.141195028(2) | 9.2991(2) | 0.0309443489(4) |
| 2.7 | −0.607649107462(4) | −1.127610460(2) | 10.3688(2) | 0.0324769462(5) |
| 2.8 | −0.604347768880(4) | −1.114982375(2) | 11.61259(10) | 0.0334689866(5) |
| 2.9 | −0.600969877222(4) | −1.103272022(2) | 13.05932(8) | 0.0340233560(5) |
| 3.0 | −0.597554901390(4) | −1.092440522(2) | 14.74179(5) | 0.0342230937(6) |
| 3.1 | −0.594134819585(4) | −1.082449328(3) | 16.69759(3) | 0.0341355844(6) |
| 3.2 | −0.590735516382(4) | −1.073260512(3) | 18.969626(10) | 0.0338157877(7) |
| 3.3 | −0.587377894736(4) | −1.064836936(3) | 21.60690(5) | 0.0333087437(7) |
| 3.4 | −0.584078766099(4) | −1.057142330(3) | 24.66536(9) | 0.0326515301(7) |
| 3.5 | −0.580851566733(4) | −1.050141334(3) | 28.2088(2) | 0.0318747999(8) |
| 3.6 | −0.577706937097(4) | −1.043799489(4) | 32.3101(2) | 0.0310039959(8) |
| 3.7 | −0.574653192800(4) | −1.038083220(4) | 37.0521(3) | 0.0300603152(8) |
| 3.8 | −0.571696709320(4) | −1.032959804(4) | 42.5297(3) | 0.0290614776(9) |
| 3.9 | −0.568842237817(4) | −1.028397346(4) | 48.8512(4) | 0.0280223410(9) |
| 4.0 | −0.566093165761(4) | −1.024364752(5) | 56.1403(5) | 0.0269553950(10) |
| 4.1 | −0.56345173323(7) | −1.020831717(2) | 64.5395(2) | 0.0258711584(3) |
| 4.2 | −0.560919213324(8) | −1.0177687401(2) | 74.21112(2) | 0.02477849680(3) |
| 4.3 | −0.55849606426(7) | −1.015147128(2) | 85.3426(2) | 0.0236848837(3) |
| 4.4 | −0.55618205758(7) | −1.012939044(2) | 98.1511(3) | 0.0225966071(3) |
| 4.5 | −0.553976388313(4) | −1.011117568(2) | 112.8875(3) | 0.0215189354(3) |
| 4.6 | −0.55187777003(8) | −1.009656784(2) | 129.8438(4) | 0.0204562512(3) |
| 4.7 | −0.54988451766(8) | −1.008531900(2) | 149.3617(4) | 0.0194121565(3) |
| 4.8 | −0.54799462163(8) | −1.007719389(2) | 171.8426(5) | 0.0183895530(3) |
| 4.9 | −0.54620581464(9) | −1.007197193(2) | 197.7611(6) | 0.0173907014(3) |
| 5.0 | −0.544515633620(6) | −1.006944965(2) | 227.6815(7) | 0.0164172605(4) |

## $1^1\Phi_g$ continued

| $R$ | $E$ | $\langle V \rangle$ | $10^6 \cdot \langle \nabla_1 \cdot \nabla_2 \rangle$ | $\mathrm{d}E/\mathrm{d}R$ |
|---|---|---|---|---|
| 5.5 | −0.53745169841(2) | −1.009193370(2) | 466.6326(8) | 0.0119472775(3) |
| 6.0 | −0.53248424182(3) | −1.017252940(7) | 999.878(3) | 0.00795259087(9) |
| 6.5 | −0.52960054618(2) | −1.037603520(2) | 2050.55248(4) | 0.0033227034(3) |
| 7.0 | −0.529133668331(6) | −1.063785059(2) | 2063.5749(2) | −0.0007882461(3) |
| 7.5 | −0.529737835301(5) | −1.069267328(2) | 1301.0201(2) | −0.0013055543(2) |
| 8.0 | −0.530315564838(4) | −1.068455174(2) | 831.6977(2) | −0.0009780056(2) |
| 8.5 | −0.53071710645(2) | −1.0668892857(9) | 557.0363(2) | −0.00064177327(8) |
| 9.0 | −0.530973140362(10) | −1.0655270792(7) | 385.6317(2) | −0.00039786650(6) |
| 9.5 | −0.53112872233(4) | −1.0645015268(6) | 273.6424(2) | −0.00023621918(5) |
| 10.0 | −0.53121917875(6) | −1.0637748(2) | 198.30(9) | −0.000133647(9) |
| 11.0 | −0.531293942136(5) | −1.06294953(9) | 111.7(2) | −0.000032876(6) |
| 12.0 | −0.53130669886(2) | −1.06260356(7) | 70.13(10) | 0.000000820(4) |
| 13.0 | −0.531300340018(3) | −1.06247576(5) | 49.26(8) | 0.000009609(2) |
| 14.0 | −0.531290135317(10) | −1.06243871(3) | 38.02(7) | 0.000010111(2) |
| 15.0 | −0.531280818245(2) | −1.06243583(3) | 31.27(6) | 0.0000083872(9) |
| 16.0 | −0.531273420425(9) | −1.06244381(2) | 26.70(5) | 0.0000064398(6) |
| 17.0 | −0.531267826205(2) | −1.062453805(10) | 23.27(4) | 0.0000048147(3) |
| 18.0 | −0.53126365969(2) | −1.062462895(10) | 20.49(4) | 0.0000035792(4) |
| 19.0 | −0.531260558267(2) | −1.062470374(8) | 18.17(4) | 0.0000026708(3) |
| 20.0 | −0.53125823597(3) | −1.062476306(7) | 16.19(4) | 0.0000020084(3) |

TABLE S30. Calculated BO energies, expectation value of potential, $\langle \nabla_1 \cdot \nabla_2 \rangle$, and $\mathrm{d}E/\mathrm{d}R$ of the $2^1\Phi_g$ state in atomic units (hartree). Uncertainties originate purely from extrapolation to the complete basis set limit. United atom values at $R = 0$ are taken from Ref. [1].

| $2^1\Phi_g$ | | | | |
|---|---|---|---|---|
| $R$ | $E$ | $\langle V \rangle$ | $10^6 \cdot \langle \nabla_1 \cdot \nabla_2 \rangle$ | $\mathrm{d}E/\mathrm{d}R$ |
| 0.0 | −2.01388934538731322(3) | − | .8985799(7) | − |
| 0.01 | 97.98637201788(6) | 95.9732614919(4) | 0.898951(7) | −9999.94825438(3) |
| 0.05 | 17.992134051(4) | 15.99569935(3) | 0.905903(10) | −399.7713750(3) |
| 0.1 | 8.007868591(6) | 6.05483979(4) | 0.9246(2) | −99.6089739(3) |
| 0.15 | 4.697055774(5) | 2.80281882(3) | 0.9516(3) | −43.9419515(2) |
| 0.2 | 3.057490371(3) | 1.23022262(2) | 0.98484(7) | −24.42379059(6) |
| 0.3 | 1.4527399616(7) | −0.233184829(4) | 1.06387(5) | −10.462215840(9) |
| 0.4 | 0.6853567069(2) | −0.8639348723(9) | 1.15465(3) | −5.586620715(2) |
| 0.5 | 0.25112284869(6) | −1.1734353637(3) | 1.253719(6) | −3.3513621221(4) |
| 0.6 | −0.01870709322(3) | −1.3321248240(2) | 1.35929(4) | −2.1578510626(2) |
| 0.7 | −0.196513755(3) | −1.4118937(3) | 1.47039(5) | −1.4555232(4) |
| 0.8 | −0.31836886056(5) | −1.4475529(2) | 1.58731(3) | −1.0135190(3) |
| 0.9 | −0.40415908315(7) | −1.4575528852(4) | 1.70997(3) | −0.7213719099(3) |
| 1.0 | −0.46567471824(4) | −1.45230972(8) | 1.83878(3) | −0.52096029(9) |
| 1.1 | −0.51030006442(4) | −1.43797918(9) | 1.974702(8) | −0.37943551(9) |
| 1.2 | −0.54286249891(3) | −1.41832522(4) | 2.118809(2) | −0.27716685(4) |
| 1.3 | −0.56662836003(6) | −1.3957071745(10) | 2.272502(10) | −0.2018849651(8) |
| 1.4 | −0.58387101883(7) | −1.3716298697(9) | 2.437550(4) | −0.1456341659(8) |
| 1.5 | −0.59621044039(3) | −1.347063332(2) | 2.61608(2) | −0.1030949674(8) |
| 1.6 | −0.60482419797(6) | −1.322635279(2) | 2.810668(8) | −0.0706168021(10) |
| 1.7 | −0.61058297899(3) | −1.298750197(2) | 3.024353(9) | −0.0456377878(8) |
| 1.8 | −0.61414008050(3) | −1.2756649053(10) | 3.26073(2) | −0.0263248580(6) |
| 1.9 | −0.61599197089(5) | −1.2535381(6) | 3.5236(5) | −0.0113443(4) |
| 2.0 | −0.61652015315(4) | −1.232459483(2) | 3.819204(10) | 0.0002904115(7) |
| 2.1 | −0.61602064883(4) | −1.212477492(7) | 4.15198(3) | 0.009316098(4) |
| 2.2 | −0.61472511280(4) | −1.193607646(7) | 4.52909(3) | 0.016292081(4) |
| 2.3 | −0.61281618030(4) | −1.175845608(7) | 4.95830(3) | 0.021646414(4) |
| 2.4 | −0.61043877185(5) | −1.159173374(7) | 5.44857(3) | 0.025710071(4) |
| 2.5 | −0.60770852173(5) | −1.14356405(6) | 6.01023(6) | 0.02874120(3) |
| 2.6 | −0.60471813097(6) | −1.12898486(5) | 6.65530(5) | 0.03094284(2) |
| 2.7 | −0.60154220361(6) | −1.115399787(5) | 7.39750(3) | 0.032475785(2) |
| 2.8 | −0.59824096209(6) | −1.102770923(4) | 8.25256(3) | 0.033468215(2) |
| 2.9 | −0.5948631253(2) | −1.091059429(5) | 9.23859(3) | 0.034023042(2) |
| 3.0 | −0.59144815462(5) | −1.080226359(2) | 10.37635(6) | 0.0342233166(4) |
| 3.1 | −0.58802802026(6) | −1.070233112(2) | 11.68963(9) | 0.0341364287(5) |
| 3.2 | −0.58462859768(6) | −1.061041680(2) | 13.2057(2) | 0.0338173486(5) |
| 3.3 | −0.58127077978(6) | −1.052614840(3) | 14.9558(2) | 0.0333111272(6) |
| 3.4 | −0.57797136688(5) | −1.044916232(3) | 16.9756(2) | 0.0326548536(6) |
| 3.5 | −0.57474378285(5) | −1.037910388(3) | 19.3062(3) | 0.0318791936(7) |
| 3.6 | −0.57159865442(5) | −1.031562734(3) | 21.9945(3) | 0.0310096042(7) |
| 3.7 | −0.56854428203(4) | −1.025839562(4) | 25.0946(4) | 0.0300672978(7) |
| 3.8 | −0.56558702433(4) | −1.020708006(4) | 28.6686(5) | 0.0290700112(8) |
| 3.9 | −0.56273161393(4) | −1.016136008(4) | 32.7881(6) | 0.0280326205(8) |
| 4.0 | −0.55998141784(4) | −1.01209231(2) | 37.535(3) | 0.026967631(4) |
| 4.1 | −0.55733865368(5) | −1.0085463779(8) | 43.0096(2) | 0.0258855926(2) |
| 4.2 | −0.55480457007(5) | −1.0054685366(8) | 49.3190(2) | 0.0247953818(2) |
| 4.3 | −0.55237959847(5) | −1.0028298609(9) | 56.5965(2) | 0.0237044968(2) |
| 4.4 | −0.55006348183(5) | −1.0006022892(9) | 64.9965(3) | 0.0226192442(2) |
| 4.5 | −0.54785538476(6) | −1.000012(2) | 73.89(2) | 0.0215449079(2) |
| 4.6 | −0.54575398915(6) | −0.9972729403(10) | 85.9332(4) | 0.0204858778(2) |
| 4.7 | −0.54375757834(6) | −0.9961201372(10) | 98.9527(4) | 0.0194457488(2) |
| 4.8 | −0.54186411293(6) | −0.995276752(2) | 114.0819(5) | 0.0184273905(3) |
| 4.9 | −0.54007130096(7) | −0.994720959(2) | 131.7154(6) | 0.0174329883(3) |
| 5.0 | −0.53837666558(6) | −0.9944330672(10) | 152.3452(5) | 0.0164640528(2) |

| $2^1\Phi_g$ continued | | | | |
|---|---|---|---|---|
| $R$ | $E$ | $\langle V \rangle$ | $10^6 \cdot \langle \nabla_1 \cdot \nabla_2 \rangle$ | $\mathrm{d}E/\mathrm{d}R$ |
| 5.5 | −0.5312860427(2) | −0.996595489(4) | 329.571(2) | 0.0119957448(6) |
| 6.0 | −0.5263714295(5) | −1.00834125(2) | 793.242(3) | 0.007400268(3) |
| 6.5 | −0.524682454(2) | −1.04765326(3) | −604.268(3) | 0.000263330(3) |
| 7.0 | −0.5240980215(9) | −1.0330771546(6) | −1740.715(2) | 0.0021598407(4) |
| 7.5 | −0.5229454714(4) | −1.029453435(2) | −1306.9467(4) | 0.00219166770(10) |
| 8.0 | −0.5219975528(7) | −1.031262696(5) | −939.2329(3) | 0.0015915512(4) |
| 8.5 | −0.5213382632(2) | −1.033574278(2) | −676.18356(8) | 0.0010708527(2) |
| 9.0 | −0.5209010560(2) | −1.035486370(2) | −480.3716(2) | 0.0007017491(2) |
| 9.5 | −0.5206158686(2) | −1.036895926(2) | −334.2670(2) | 0.0004564011(2) |
| 10.0 | −0.52043025053(2) | −1.0378827587(2) | −227.34718(6) | 0.00029777424(2) |
| 11.0 | −0.52022781909(3) | −1.0390077993(3) | −97.61520(9) | 0.00013162171(3) |
| 12.0 | −0.52013529737(4) | −1.0395121176(4) | −36.4244(2) | 0.00006320643(3) |
| 13.0 | −0.5200564094(2) | −1.039739524(2) | −9.3027(4) | 0.00003369808(8) |
| 14.0 | −0.5200627937(2) | −1.0398464465(9) | 2.2407(4) | 0.00001993864(5) |
| 15.0 | −0.52004672767(4) | −1.0398996486(7) | 6.9592(4) | 0.00001292045(3) |
| 16.0 | −0.52003594428(3) | −1.0399280587(6) | 8.6003(3) | 0.00000898936(3) |
| 17.0 | −0.52002193035(8) | −1.039954(5) | 8.9(9) | – |
| 18.0 | −0.52001710260(2) | −1.039961(3) | 8.1(3) | 0.0000034(8) |
| 19.0 | −0.52001345291(2) | −1.039969(2) | 6.5(8) | 0.0000026(7) |
| 20.0 | −0.520010678621(9) | −1.039975(3) | 5(2) | 0.0000019(6) |

TABLE S31. Calculated BO energies, expectation value of potential, $\langle\nabla_1 \cdot \nabla_2\rangle$, and $\mathrm{d}E/\mathrm{d}R$ of the $1^3\Phi_g$ state in atomic units (hartree). Uncertainties originate purely from extrapolation to the complete basis set limit. United atom values at $R = 0$ are taken from Ref. [1].

| $1^3\Phi_\mathrm{g}$ | | | | |
|---|---|---|---|---|
| $R$ | $E$ | $\langle V\rangle$ | $10^6 \cdot \langle\nabla_1 \cdot \nabla_2\rangle$ | $\mathrm{d}E/\mathrm{d}R$ |
| 0.0 | −2.02000071089858471(1) | − | 1.4040013 | − |
| 0.01 | 97.98026065231(5) | 95.9610387606(4) | 1.404491(3) | −9999.94825440(3) |
| 0.05 | 17.986022684(2) | 15.98347661(2) | 1.41505(3) | −399.7713752(2) |
| 0.1 | 8.001757227(3) | 6.04261706(2) | 1.44361(2) | −99.6089740(2) |
| 0.15 | 4.690944418(3) | 2.79059613(2) | 1.484358(9) | −43.94195139(8) |
| 0.2 | 3.0513790279(7) | 1.217999989(5) | 1.53393(5) | −24.42379033(2) |
| 0.3 | 1.4466286553(2) | −0.245407304(2) | 1.650998(8) | −10.462215383(3) |
| 0.4 | 0.67924545608(8) | −0.8761571128(6) | 1.783686(6) | −5.5866200623(10) |
| 0.5 | 0.24501167293(4) | −1.1856572912(3) | 1.926481(7) | −3.3513612741(4) |
| 0.6 | −0.024818174559(4) | −1.3443463632(2) | 2.07652(2) | −2.1578500235(3) |
| 0.7 | −0.202624721835(2) | −1.4241145204(7) | 2.23241(5) | −1.4555215380(7) |
| 0.8 | −0.324479697276(2) | −1.4597732990(5) | 2.39372(5) | −1.0135173804(5) |
| 0.9 | −0.410269771177(2) | −1.4697728485(3) | 2.56061(5) | −0.7213703401(3) |
| 1.0 | −0.471785241314(2) | −1.4645289490(3) | 2.73375(4) | −0.5209584663(2) |
| 1.1 | −0.516410407332(2) | −1.4501977069(2) | 2.91431(4) | −0.3794335383(2) |
| 1.2 | −0.548972647684(2) | −1.4305430644(3) | 3.10389(5) | −0.2771648075(2) |
| 1.3 | −0.572738301986(2) | −1.4079242937(2) | 3.30466(3) | −0.20188283820(10) |
| 1.4 | −0.589980742896(2) | −1.3838461955(2) | 3.51922(3) | −0.14563193546(10) |
| 1.5 | −0.602319937028(2) | −1.3592788497(3) | 3.75086(3) | −0.1030926504(2) |
| 1.6 | −0.610933459431(2) | −1.3348499864(3) | 4.00352(3) | −0.0706144172(2) |
| 1.7 | −0.616691999530(2) | −1.3109641044(3) | 4.28193(2) | −0.0456353561(2) |
| 1.8 | −0.620248856493(3) | −1.2878780370(3) | 4.59168(2) | −0.0263224022(2) |
| 1.9 | −0.622100501227(3) | −1.2657498773(4) | 4.939401(7) | −0.0113415130(2) |
| 2.0 | −0.622628439218(3) | −1.2446712026(5) | 5.3328446(4) | 0.0002928379(2) |
| 2.1 | −0.622128694991(3) | −1.2246886082(6) | 5.781084(8) | 0.0093184675(2) |
| 2.2 | −0.620832926651(4) | −1.2058182652(6) | 6.29471(2) | 0.0162943582(3) |
| 2.3 | −0.618923772982(4) | −1.1880558574(7) | 6.88602(3) | 0.0216485603(3) |
| 2.4 | −0.616546158449(4) | −1.1713834096(9) | 7.56923(5) | 0.0257120448(4) |
| 2.5 | −0.613815721719(4) | −1.1557740022(10) | 8.36080(7) | 0.0287429765(4) |
| 2.6 | −0.610825168645(4) | −1.141195032(2) | 9.27967(8) | 0.0309443481(4) |
| 2.7 | −0.607649108655(4) | −1.127610465(2) | 10.34766(10) | 0.0324769454(5) |
| 2.8 | −0.604347770163(4) | −1.114982380(2) | 11.5898(2) | 0.0334689857(5) |
| 2.9 | −0.600969878595(4) | −1.103272027(2) | 13.0348(2) | 0.0340233552(5) |
| 3.0 | −0.597554902852(4) | −1.092440527(2) | 14.7156(2) | 0.0342230929(6) |
| 3.1 | −0.594134821136(4) | −1.082449333(3) | 16.6697(2) | 0.0341355836(6) |
| 3.2 | −0.590735518019(4) | −1.073260518(3) | 18.9401(3) | 0.0338157868(6) |
| 3.3 | −0.587377896456(4) | −1.064836942(3) | 21.5759(3) | 0.0333087429(7) |
| 3.4 | −0.584078767897(4) | −1.057142336(3) | 24.6329(4) | 0.0326515294(7) |
| 3.5 | −0.580851568604(4) | −1.050141340(3) | 28.1751(4) | 0.0318747992(8) |
| 3.6 | −0.577706939031(4) | −1.043799495(4) | 32.2753(4) | 0.0310039953(8) |
| 3.7 | −0.574653194791(4) | −1.038083226(4) | 37.0164(5) | 0.0300603147(8) |
| 3.8 | −0.571696711355(4) | −1.032959810(4) | 42.4934(5) | 0.0290614772(9) |
| 3.9 | −0.568842239883(4) | −1.028397351(4) | 48.8145(6) | 0.0280223408(9) |
| 4.0 | −0.566093167843(4) | −1.024364756(5) | 56.1037(6) | 0.0269553950(10) |
| 4.1 | −0.56345173531(7) | −1.020831720(2) | 64.5035(2) | 0.0258711586(3) |
| 4.2 | −0.560919215381(9) | −1.0177687428(2) | 74.17613(2) | 0.02477849714(3) |
| 4.3 | −0.55849606627(7) | −1.015147130(2) | 85.3091(3) | 0.0236848843(3) |
| 4.4 | −0.55618205951(7) | −1.012939044(2) | 98.1198(3) | 0.0225966080(3) |
| 4.5 | −0.553976390142(5) | −1.0111175651(4) | 112.85946(10) | 0.02151893670(8) |
| 4.6 | −0.55187777172(8) | −1.009656780(2) | 129.8195(4) | 0.0204562529(3) |
| 4.7 | −0.54988451915(8) | −1.008531893(2) | 149.3424(4) | 0.0194121586(3) |
| 4.8 | −0.54799462289(9) | −1.007719379(2) | 171.8296(5) | 0.0183895556(3) |
| 4.9 | −0.54620581561(9) | −1.007197179(2) | 197.7558(6) | 0.0173907046(4) |
| 5.0 | −0.544515634232(8) | −1.006944953(9) | 227.684(3) | 0.016417263(2) |

| $1^3\Phi_g$ continued | | | | |
|---|---|---|---|---|
| $R$ | $E$ | $\langle V\rangle$ | $10^6\cdot\langle\nabla_1\cdot\nabla_2\rangle$ | $\mathrm{d}E/\mathrm{d}R$ |
| 5.5 | −0.53745169574(2) | −1.009193310(2) | 466.7247(7) | 0.0119472876(3) |
| 6.0 | −0.53248423099(3) | −1.0172527689(6) | 1000.20982(8) | 0.00795261551(8) |
| 6.5 | −0.52960051946(3) | −1.037603290(2) | 2051.4886(2) | 0.0033227305(2) |
| 7.0 | −0.52913364740(2) | −1.063785291(2) | 2064.7731(2) | −0.0007882852(2) |
| 7.5 | −0.529737831222(6) | −1.069267503(2) | 1301.9094(2) | −0.0013055788(2) |
| 8.0 | −0.530315569157(2) | −1.0684552680(9) | 832.36662(8) | −0.00097801621(9) |
| 8.5 | −0.53071711419(4) | −1.0668893331(7) | 557.57538(5) | −0.00064177702(7) |
| 9.0 | −0.53097314904(5) | −1.0655270998(6) | 386.09105(3) | −0.00039786686(5) |
| 9.5 | −0.531128730660(4) | −1.0645015312(5) | 274.04932(2) | −0.00023621788(4) |
| 10.0 | −0.531219186210(7) | −1.0637748(2) | 198.6(2) | −0.000133644(9) |
| 11.0 | −0.53129394746(2) | −1.06294951(9) | 112.0(2) | −0.000032874(6) |
| 12.0 | −0.531306702177(4) | −1.06260355(7) | 70.39(10) | 0.000000822(4) |
| 13.0 | −0.531300341891(10) | −1.06247575(5) | 49.49(9) | 0.000009610(3) |
| 14.0 | −0.531290136196(2) | −1.06243871(4) | 38.21(7) | 0.000010112(2) |
| 15.0 | −0.531280818530(6) | −1.06243583(3) | 31.43(6) | 0.0000083877(9) |
| 16.0 | −0.5312734203530(8) | −1.06244380(2) | 26.84(5) | 0.0000064400(6) |
| 17.0 | −0.531267825969(5) | −1.062453803(10) | 23.39(4) | 0.0000048148(4) |
| 18.0 | −0.5312636593677(5) | −1.062462894(10) | 20.59(5) | 0.0000035793(4) |
| 19.0 | −0.531260557947(8) | −1.062470373(9) | 18.25(4) | 0.0000026707(3) |
| 20.0 | −0.5312582356315(6) | −1.062476306(7) | 16.25(4) | 0.0000020083(3) |

TABLE S32. Calculated BO energies, expectation value of potential, $\langle\nabla_1 \cdot \nabla_2\rangle$, and $\mathrm{d}E/\mathrm{d}R$ of the $2^3\Phi_g$ state in atomic units (hartree). Uncertainties originate purely from extrapolation to the complete basis set limit. United atom values at $R = 0$ are taken from Ref. [1].

| $2^3\Phi_g$ | | | | |
|---|---|---|---|---|
| $R$ | $E$ | $\langle V\rangle$ | $10^6 \cdot \langle\nabla_1 \cdot \nabla_2\rangle$ | $\mathrm{d}E/\mathrm{d}R$ |
| 0.0 | −2.01388934538731322(3) | − | .8981237(7) | − |
| 0.01 | 97.98637201784(6) | 95.9732614918(4) | 0.89843(2) | −9999.94825439(3) |
| 0.05 | 17.992134053(4) | 15.99569936(3) | 0.90536(4) | −399.7713749(4) |
| 0.1 | 8.007868589(5) | 6.05483978(3) | 0.9240(3) | −99.6089740(2) |
| 0.15 | 4.697055773(3) | 2.80281881(2) | 0.9510(3) | −43.94195157(8) |
| 0.2 | 3.057490371(4) | 1.23022263(2) | 0.9842(2) | −24.42379059(7) |
| 0.3 | 1.4527399616(10) | −0.233184829(6) | 1.06306(10) | −10.46221584(2) |
| 0.4 | 0.6853567068(3) | −0.863934872(2) | 1.15366(8) | −5.586620715(2) |
| 0.5 | 0.25112284862(6) | −1.1734353639(3) | 1.25251(7) | −3.3513621222(4) |
| 0.6 | −0.01870709330(3) | −1.3321248242(2) | 1.35786(5) | −2.1578510627(2) |
| 0.7 | −0.1965137539(2) | −1.4118937(3) | 1.46886(4) | −1.4555232(4) |
| 0.8 | −0.31836886068(4) | −1.4475529(2) | 1.58542(2) | −1.0135190(3) |
| 0.9 | −0.40415908329(6) | −1.4575528857(4) | 1.707661(7) | −0.7213719101(2) |
| 1.0 | −0.46567471841(6) | −1.45230972(8) | 1.83603(2) | −0.52096029(9) |
| 1.1 | −0.51030006462(3) | −1.437984(4) | 1.97141(2) | −0.37943551(9) |
| 1.2 | −0.54286249915(3) | −1.41832522(4) | 2.11491(2) | −0.27716685(4) |
| 1.3 | −0.56662836026(2) | −1.3957071756(10) | 2.267936(3) | −0.2018849655(8) |
| 1.4 | −0.58387101914(3) | −1.3716298710(9) | 2.4322191(5) | −0.1456341664(8) |
| 1.5 | −0.59621044076(3) | −1.347063333(2) | 2.609904(5) | −0.1030949679(8) |
| 1.6 | −0.60482419839(2) | −1.322635281(2) | 2.803561(4) | −0.0706168027(10) |
| 1.7 | −0.61058297952(5) | −1.298750199(2) | 3.016228(4) | −0.0456377884(8) |
| 1.8 | −0.61414008101(3) | −1.2756649076(10) | 3.251502(5) | −0.0263248587(6) |
| 1.9 | −0.61599197151(3) | −1.25353756(7) | 3.51358(2) | −0.01134401(4) |
| 2.0 | −0.61652015384(3) | −1.232459486(2) | 3.807494(5) | 0.0002904107(7) |
| 2.1 | −0.6160206497(2) | −1.212477496(7) | 4.13891(2) | 0.009316097(4) |
| 2.2 | −0.6147251138(2) | −1.193607650(7) | 4.51458(2) | 0.016292080(4) |
| 2.3 | −0.61281618122(6) | −1.175845612(7) | 4.94227(2) | 0.021646413(4) |
| 2.4 | −0.61043877286(8) | −1.159173378(7) | 5.43095(2) | 0.025710070(4) |
| 2.5 | −0.60770852284(5) | −1.14356405(6) | 5.99098(3) | 0.02874120(3) |
| 2.6 | −0.60471813217(5) | −1.12898487(5) | 6.63435(3) | 0.03094284(2) |
| 2.7 | −0.60154220490(9) | −1.115399792(5) | 7.37481(2) | 0.032475784(2) |
| 2.8 | −0.59824096348(5) | −1.102770928(4) | 8.22812(2) | 0.033468214(2) |
| 2.9 | −0.59486312673(10) | −1.091059434(5) | 9.21240(2) | 0.034023041(2) |
| 3.0 | −0.59144815620(10) | −1.080226365(2) | 10.3481(2) | 0.0342233157(4) |
| 3.1 | −0.58802802192(5) | −1.070233118(2) | 11.6597(3) | 0.0341364278(5) |
| 3.2 | −0.58462859943(5) | −1.061041686(2) | 13.1742(3) | 0.0338173478(5) |
| 3.3 | −0.58127078162(6) | −1.052614846(2) | 14.9227(3) | 0.0333111263(6) |
| 3.4 | −0.57797136880(5) | −1.044916238(3) | 16.9411(4) | 0.0326548528(6) |
| 3.5 | −0.57474378484(5) | −1.037910394(3) | 19.2705(4) | 0.0318791930(6) |
| 3.6 | −0.57159865648(5) | −1.031562740(3) | 21.9577(5) | 0.0310096037(7) |
| 3.7 | −0.56854428413(4) | −1.025839568(3) | 25.0570(5) | 0.0300672974(7) |
| 3.8 | −0.56558702647(4) | −1.020708012(4) | 28.6305(6) | 0.0290700109(8) |
| 3.9 | −0.56273161610(5) | −1.016136013(4) | 32.7499(7) | 0.0280326203(8) |
| 4.0 | −0.55998142002(2) | −1.01209230023(5) | 37.49936(2) | 0.02696763494(2) |
| 4.1 | −0.55733865584(5) | −1.0085463810(8) | 42.9727(2) | 0.0258855929(2) |
| 4.2 | −0.55480457218(6) | −1.0054685384(9) | 49.2836(2) | 0.0247953824(2) |
| 4.3 | −0.55237960051(6) | −1.0028298611(9) | 56.5632(3) | 0.0237044977(2) |
| 4.4 | −0.55006348376(6) | −1.0006022876(9) | 64.9662(3) | 0.0226192454(2) |
| 4.5 | −0.54785538653(4) | −0.998758683(8) | 74.674(2) | 0.0215449096(2) |
| 4.6 | −0.54575399074(6) | −0.9972729334(10) | 85.9120(4) | 0.0204858800(2) |
| 4.7 | −0.54375757969(6) | −0.996120127(2) | 98.9380(4) | 0.0194457516(2) |
| 4.8 | −0.54186411396(7) | −0.995276737(2) | 114.0754(5) | 0.0184273940(3) |
| 4.9 | −0.54007130160(7) | −0.994720939(2) | 131.7192(6) | 0.0174329927(3) |
| 5.0 | −0.53837666574(8) | −0.994433041(2) | 152.3610(7) | 0.0164640581(3) |

## $2^3\Phi_g$ continued

| $R$ | $E$ | $\langle V \rangle$ | $10^6 \cdot \langle \nabla_1 \cdot \nabla_2 \rangle$ | $\mathrm{d}E/\mathrm{d}R$ |
|---|---|---|---|---|
| 5.5 | −0.5312860381(2) | −0.996595394(4) | 329.7144(10) | 0.0119957604(6) |
| 6.0 | −0.5263714100(4) | −1.00834093(2) | 793.855(3) | 0.007400315(3) |
| 6.5 | −0.524682462(2) | −1.047659(3) | −603.90(3) | 0.0002625(4) |
| 7.0 | −0.5240980613(10) | −1.03307728(5) | −1741.3659(9) | 0.002159834(7) |
| 7.5 | −0.5229455057(3) | −1.029453421(2) | −1307.624(2) | 0.00219167878(9) |
| 8.0 | −0.5219975826(3) | −1.031262699(2) | −939.8468(10) | 0.0015915582(2) |
| 8.5 | −0.52133829005(2) | −1.0335742894(3) | −676.74532(5) | 0.00107085773(3) |
| 9.0 | −0.52090108068(2) | −1.0354863832(2) | −480.89141(2) | 0.00070175313(2) |
| 9.5 | −0.5206158917(7) | −1.036895941(7) | −334.753(3) | 0.0004564044(6) |
| 10.0 | −0.5204302708(2) | −1.03788282(3) | −227.798(5) | 0.000297772(4) |
| 11.0 | −0.52022783709(2) | −1.0390078012(3) | −97.99697(4) | 0.00013162482(2) |
| 12.0 | −0.52006037370(2) | −1.0401606117(2) | 36.30812(3) | −0.000003322023(10) |
| 13.0 | −0.5200564068(10) | −1.04000143(3) | 24.490(3) | 0.000008567(3) |
| 14.0 | −0.52004645435(2) | −1.039946728(3) | 18.1340(5) | 0.0000104415(3) |
| 15.0 | −0.52003652449(10) | −1.039935388(2) | 14.1943(2) | 0.00000917740(9) |
| 16.0 | −0.520035949525(9) | −1.039928049(2) | 8.48699(2) | 0.00000899064(7) |
| 17.0 | −0.52002192992(4) | −1.0399497528(5) | 9.76319(6) | 0.00000553571(3) |
| 18.0 | −0.520017102222(5) | −1.039958935(2) | 8.40706(8) | 0.00000418166(8) |
| 19.0 | −0.52001345259(2) | −1.0399667138(5) | 7.3313(2) | 0.000003168010(4) |
| 20.0 | −0.520010678359(7) | −1.03997299305(5) | 6.44438(5) | 0.000002418184(2) |

TABLE S33. Calculated BO energies, expectation value of potential, $\langle\nabla_1 \cdot \nabla_2\rangle$, and $\mathrm{d}E/\mathrm{d}R$ of the $1^1\Phi_u$ state in atomic units (hartree). Uncertainties originate purely from extrapolation to the complete basis set limit. United atom values at $R = 0$ are taken from Ref. [1].

| $1^1\Phi_\mathrm{u}$ | | | | |
|---|---|---|---|---|
| $R$ | $E$ | $\langle V\rangle$ | $10^6 \cdot \langle\nabla_1 \cdot \nabla_2\rangle$ | $\mathrm{d}E/\mathrm{d}R$ |
| 0.0 | −2.031255144381749(1) | – | 10.0242694(2) | – |
| 0.01 | 97.969006228(4) | 95.938529907(6) | 10.0265(2) | −9999.9482548(6) |
| 0.05 | 17.974768337(4) | 2.01380025(2) | 10.0724(2) | −399.7713723(3) |
| 0.1 | 7.990503118(6) | 1.97039358(2) | 10.1825(2) | −99.6089674(2) |
| 0.15 | 4.67969074(2) | 2.76809038(8) | 10.3164(2) | −43.9419407(4) |
| 0.2 | 3.040125975(6) | 1.844629191(7) | 10.4476(2) | −24.423775896(5) |
| 0.3 | 1.435377438(3) | −0.267903017(5) | 10.6322(2) | −10.46219298(2) |
| 0.4 | 0.6679968825(8) | 1.5666389000(5) | 10.6355(2) | −5.5865894619(10) |
| 0.5 | 0.2337665670(2) | −1.2081281176(9) | 10.39373(7) | −3.351322503(2) |
| 0.6 | −0.0360589992(2) | −1.3667999170(3) | 9.8601(2) | −2.157803197735(7) |
| 0.7 | −0.21386046443(2) | −1.4465476608(4) | 8.9963(2) | −1.4554667599(5) |
| 0.8 | −0.33570957143(2) | −1.4821829958(4) | 7.7682(2) | −1.0134548162(4) |
| 0.9 | −0.42149300671(2) | −1.4921561585(4) | 6.1441(2) | −0.7213001612(3) |
| 1.0 | −0.48300108593(2) | −1.4868830305(3) | 4.0937(2) | −0.5208808586(3) |
| 1.1 | −0.527618127935(10) | −1.4725198255(3) | 1.5875(2) | −0.3793486996(2) |
| 1.2 | −0.560171531512(9) | −1.4528305984(3) | −1.4037(2) | −0.2770729461(2) |
| 1.3 | −0.583927657587(9) | −1.4301747388(3) | −4.9086(2) | −0.2017841720(2) |
| 1.4 | −0.601159901042(8) | −1.4060571694(3) | −8.95552(10) | −0.1455266910(2) |
| 1.5 | −0.613488251553(8) | −1.3814480964(3) | −13.57236(10) | −0.1029810622(2) |
| 1.6 | −0.622090308009(7) | −1.3569753798(3) | −18.78653(10) | −0.0704967274(2) |
| 1.7 | −0.627836784404(7) | −1.3330436522(2) | −24.62475(9) | −0.04551181378(10) |
| 1.8 | −0.631381005140(7) | −1.3099098837(2) | −31.11288(9) | −0.02619326301(9) |
| 1.9 | −0.633219466975(7) | −1.2877323065(2) | −38.27574(9) | −0.01120703818(9) |
| 2.0 | −0.633733701792(7) | −1.2666026398(2) | −46.13683(8) | 0.00043238191(8) |
| 2.1 | −0.633219760989(6) | −1.2465676214(2) | −54.71807(8) | 0.00946280980(8) |
| 2.2 | −0.631909329935(6) | −1.2276435661(2) | −64.03956(8) | 0.01644322445(7) |
| 2.3 | −0.629985074983(6) | −1.2098263006(5) | −74.1192(2) | 0.0218016736(2) |
| 2.4 | −0.627591948354(6) | −1.1930979915(5) | −84.9725(2) | 0.0258691272(2) |
| 2.5 | −0.624845616542(6) | −1.1774318586(5) | −96.6117(2) | 0.0289037498(2) |
| 2.6 | −0.621838813147(6) | −1.1627954335(5) | −109.0464(2) | 0.0311085357(2) |
| 2.7 | −0.618646175106(6) | −1.1491528103(5) | −122.2820(2) | 0.0326442740(2) |
| 2.8 | −0.615327957908(6) | −1.1364661906(5) | −136.3202(2) | 0.0336391876(2) |
| 2.9 | −0.611932913405(6) | −1.1246969339(5) | −151.1579(2) | 0.0341961700(2) |
| 3.0 | −0.608500536022(6) | −1.1138062594(5) | −166.7872(2) | 0.0343982709(2) |
| 3.1 | −0.605062828290(6) | −1.1037557022(5) | −183.1947(2) | 0.0343128885(2) |
| 3.2 | −0.601645697588(6) | −1.0945073967(5) | −200.3614(2) | 0.0339949995(2) |
| 3.3 | −0.598270067763(6) | −1.0860242399(5) | −218.2617(2) | 0.0334896653(2) |
| 3.4 | −0.594952768802(7) | −1.0782699726(6) | −236.8636(2) | 0.0328339897(2) |
| 3.5 | −0.591707252630(7) | −1.0712092054(6) | −256.1277(2) | 0.0320586571(2) |
| 3.6 | −0.5885441171891(7) | −1.0648074093(6) | −276.0076(2) | 0.0311891485(2) |
| 3.7 | −0.585471850207(7) | −1.0590308864(6) | −296.4488(2) | 0.0302467065(2) |
| 3.8 | −0.582496666060(7) | −1.0538467305(6) | −317.3890(2) | 0.0292491057(2) |
| 3.9 | −0.579623367646(7) | −1.049222787(3) | −338.7581(6) | 0.0282112688(5) |
| 4.0 | −0.576855332331(8) | −1.0451276074(3) | −360.47622(6) | 0.02714576432(6) |
| 4.1 | −0.574194781545(4) | −1.04153043380(2) | −382.457708(5) | 0.026063202266(4) |
| 4.2 | −0.571642959661(4) | −1.03840116230(2) | −404.607126(5) | 0.024972561195(3) |
| 4.3 | −0.569200283754(4) | −1.03571034011(2) | −426.821556(4) | 0.023881448233(2) |
| 4.4 | −0.566866469691(4) | −1.033429165276(8) | −448.990566(3) | 0.0227963122971(5) |
| 4.5 | −0.564640638988(10) | −1.0315294990(4) | −470.99674(5) | 0.02172261753(9) |
| 4.6 | −0.562521409943(4) | −1.029983886282(3) | −492.7160563(7) | 0.020664985563(3) |
| 4.7 | −0.56050697595(3) | −1.0287655903(5) | −514.01922(6) | 0.01962731095(10) |
| 4.8 | −0.558595173062(4) | −1.02784862562(2) | −534.771834(2) | 0.018612858435(6) |
| 4.9 | −0.55678353921(3) | −1.0272078067(5) | −554.83632(6) | 0.0176243411(2) |
| 5.0 | −0.55506936552(2) | −1.026818796(8) | −574.0728(5) | 0.016663987(2) |

## $1^1\Phi_u$ continued

| $R$ | $E$ | $\langle V \rangle$ | $10^6 \cdot \langle \nabla_1 \cdot \nabla_2 \rangle$ | $\mathrm{d}E/\mathrm{d}R$ |
|---|---|---|---|---|
| 5.5 | −0.54785365779(2) | −1.027863434(4) | −652.94263(7) | 0.0123352513(7) |
| 6.0 | −0.54259339941(3) | −1.032109152(6) | −691.5148(3) | 0.0088462746(8) |
| 6.5 | −0.538872121538(4) | −1.03766180854(5) | −679.84118(2) | 0.006166528390(6) |
| 7.0 | −0.536309065021(4) | −1.04326905151(5) | −619.11669(2) | 0.004192725505(5) |
| 7.5 | −0.534583756716(4) | −1.04822199541(4) | −522.59231(2) | 0.002792735736(4) |
| 8.0 | −0.533443121857(3) | −1.05222641596(4) | −410.40869(2) | 0.001832478470(4) |
| 8.5 | −0.532698157459(3) | −1.05526672072(3) | −301.39795(2) | 0.001191716964(3) |
| 9.0 | −0.532214608932(3) | −1.05747608452(3) | −207.534512(10) | 0.000772570371(3) |
| 9.5 | −0.531900994174(3) | −1.05903565893(3) | −133.324224(10) | 0.000501718886(3) |
| 10.0 | −0.531696842363(3) | −1.06011651063(3) | −78.164401(9) | 0.000327717409(2) |
| 11.0 | −0.531474182951(2) | −1.06136161312(2) | −12.328689(7) | 0.000144250253(2) |
| 12.0 | −0.531373678949(2) | −1.061936381977(10) | 16.378487(5) | 0.0000675813268(7) |
| 13.0 | −0.5313249072835(8) | −1.062202643292(6) | 26.738516(3) | 0.0000343977904(4) |
| 14.0 | −0.5312990421541(6) | −1.062329327219(4) | 28.901556(2) | 0.0000191969350(2) |
| 15.0 | −0.5312840134709(4) | −1.062392839129(3) | 27.738573(2) | 0.0000116791875(2) |
| 16.0 | −0.5312745553792(3) | −1.062427186623(2) | 25.4247167(4) | 0.00000762025844(4) |
| 17.0 | −0.5312682254520(3) | −1.0624474744235(7) | 22.87243969(9) | 0.00000523391061(2) |
| 18.0 | −0.5312637986729(2) | −1.0624605131116(6) | 20.4346350(6) | 0.00000372690187(5) |
| 19.0 | −0.5312606060388(2) | −1.062469487543(2) | 18.2274520(9) | 0.00000272234389(9) |
| 20.0 | −0.5312582520459(2) | −1.062475978723(3) | 16.271919(2) | 0.0000020262684(2) |

TABLE S34. Calculated BO energies, expectation value of potential, $\langle\nabla_1 \cdot \nabla_2\rangle$, and $\mathrm{d}E/\mathrm{d}R$ of the $2^1\Phi_u$ state in atomic units (hartree). Uncertainties originate purely from extrapolation to the complete basis set limit. United atom values at $R = 0$ are taken from Ref. [1].

| $2^1\Phi_\mathrm{u}$ | | | | |
|---|---|---|---|---|
| $R$ | $E$ | $\langle V\rangle$ | $10^6 \cdot \langle\nabla_1 \cdot \nabla_2\rangle$ | $\mathrm{d}E/\mathrm{d}R$ |
| 0.0 | −2.0200029371587427(5) | − | 5.7042946(4) | − |
| 0.01 | 97.98025842757(9) | 95.9610343145(7) | 5.631(3) | −9999.94825407(6) |
| 0.05 | 17.986020496(5) | 15.98347232(3) | 5.736(2) | −399.7713735(5) |
| 0.1 | 8.001755150(2) | 6.042613241(5) | 5.8(4) | −99.60897084(9) |
| 0.15 | 4.690942543(3) | 2.79059311(2) | 5.869(3) | −43.94194649(7) |
| 0.2 | 3.0513774442(9) | 1.217998177(6) | 6.0(2) | −24.42378356(2) |
| 0.3 | 1.446627938(3) | −0.24540556(2) | 6.16(2) | −10.46220479(4) |
| 0.4 | 0.6792459979(9) | −0.876150220(7) | 6.240(2) | −5.58660554(2) |
| 0.5 | 0.2450138616(7) | −1.185643704(6) | 6.212(2) | −3.351342855(10) |
| 0.6 | −0.0248139508(7) | −1.344324548(6) | 6.046(2) | −2.157827744(8) |
| 0.7 | −0.2026180795(6) | −1.424082976(6) | 5.719(2) | −1.455495452(7) |
| 0.8 | −0.324470259(2) | −1.45973056(2) | 5.216(4) | −1.01348755(2) |
| 0.9 | −0.4102571668(5) | −1.469717500(6) | 4.516(2) | −0.721336852(5) |
| 1.0 | −0.4717691084(5) | −1.464459612(5) | 3.605(2) | −0.520921395(5) |
| 1.1 | −0.5163903918(5) | −1.450113051(5) | 2.468(2) | −0.379392971(4) |
| 1.2 | −0.5489484043(5) | −1.430441807(5) | 1.089(2) | −0.277120832(4) |
| 1.3 | −0.5727094946(5) | −1.407805203(5) | −0.549(2) | −0.201835549(4) |
| 1.4 | −0.5899470448(5) | −1.383708088(5) | −2.459(2) | −0.145581427(3) |
| 1.5 | −0.6022810312(5) | −1.359120593(5) | −4.658(2) | −0.103039021(3) |
| 1.6 | −0.6108890387(5) | −1.334670501(5) | −7.159(2) | −0.070557765(3) |
| 1.7 | −0.6166417666(4) | −1.310762360(5) | −9.977(2) | −0.045575781(3) |
| 1.8 | −0.6201925240(4) | −1.287653055(5) | −13.126(2) | −0.026260004(3) |
| 1.9 | −0.6220377920(4) | −1.265500728(5) | −16.620(2) | −0.011276392(3) |
| 2.0 | −0.6225590858(4) | −1.244397004(5) | −20.471(2) | 0.000360584(2) |
| 2.1 | −0.6220524398(4) | −1.224388523(5) | −24.692(2) | 0.009388741(2) |
| 2.2 | −0.6207495216(4) | −1.205491499(5) | −29.294(2) | 0.016367066(2) |
| 2.3 | −0.6188329794(9) | −1.18770165(2) | −34.286(3) | 0.021723612(4) |
| 2.4 | −0.6164477460(9) | −1.171001038(2) | −39.678(3) | 0.025789356(4) |
| 2.5 | −0.6137094685(9) | −1.15536276(2) | −45.477(3) | 0.028822469(4) |
| 2.6 | −0.6107108600(9) | −1.14075424(2) | −51.689(3) | 0.031025952(4) |
| 2.7 | −0.6075265366(9) | −1.12713945(2) | −58.318(3) | 0.032560601(4) |
| 2.8 | −0.6042167320(10) | −1.11448046(2) | −65.366(3) | 0.033554645(4) |
| 2.9 | −0.6008301758(10) | −1.10273850(2) | −72.832(3) | 0.034110984(4) |
| 3.0 | −0.5974063394(10) | −1.09187465(2) | −80.715(3) | 0.034312676(4) |
| 3.1 | −0.5939772016(10) | −1.08185032(2) | −89.009(3) | 0.034227124(4) |
| 3.2 | −0.5905686456(10) | −1.07262749(2) | −97.705(3) | 0.033909312(4) |
| 3.3 | −0.587201570(2) | −1.06416893(2) | −106.793(3) | 0.033404307(4) |
| 3.4 | −0.5838927796(5) | −1.056438208(6) | −116.259(2) | 0.032749221(2) |
| 3.5 | −0.5806556998(5) | −1.049399799(6) | −126.0839(10) | 0.031974743(2) |
| 3.6 | −0.5775009564(5) | −1.043019016(6) | −136.2471(10) | 0.031106360(2) |
| 3.7 | −0.5744368457(5) | −1.037262002(7) | −146.7233(9) | 0.030165322(2) |
| 3.8 | −0.5714697181(5) | −1.032095692(7) | −157.4835(9) | 0.029169406(2) |
| 3.9 | −0.5686042934(6) | −1.027487770(7) | −168.4949(8) | 0.028133543(2) |
| 4.0 | −0.565843920(2) | −1.02340663(2) | −179.721(2) | 0.027070302(4) |
| 4.1 | −0.563190794(9) | −1.01982138(10) | −191.5(5) | 0.02599029(2) |
| 4.2 | −0.560646121(9) | −1.01670168(9) | −202.66(5) | 0.02490251(2) |
| 4.3 | −0.558210294(8) | −1.01401798(8) | −215.2(3) | 0.02381456(2) |
| 4.4 | −0.5558829941(7) | −1.011741273(8) | −225.8963(4) | 0.022732890(2) |
| 4.5 | −0.553663320(2) | −1.00984334(2) | −237.5075(5) | 0.021662957(4) |
| 4.6 | −0.5515498565(7) | −1.008296539(9) | −249.0338(2) | 0.020609386(2) |
| 4.7 | −0.54954077(2) | −1.0070741(2) | −260.6(2) | 0.01957606(3) |
| 4.8 | −0.54763386(2) | −1.00614970(9) | −272.23(9) | 0.01856626(2) |
| 4.9 | −0.54582665(2) | −1.0054982(2) | −282.7(2) | 0.01758266(2) |
| 5.0 | −0.544116377(2) | −1.00509521(3) | −293.0299(10) | 0.016627510(4) |

| | | $2^1\Phi_u$ continued | | |
|---|---|---|---|---|
| $R$ | $E$ | $\langle V\rangle$ | $10^6\cdot\langle\nabla_1\cdot\nabla_2\rangle$ | $\mathrm{d}E/\mathrm{d}R$ |
| 5.5 | −0.536911771(3) | −1.00601866(6) | −338.291(8) | 0.012328161(9) |
| 6.0 | −0.531646992(3) | −1.01006475(7) | −365.26(2) | 0.008871540(9) |
| 6.5 | −0.52790539698(8) | −1.0153707881(10) | −368.0816(3) | 0.0062215394(2) |
| 7.0 | −0.52530915845(7) | −1.0207388819(9) | −345.3826(3) | 0.00426849071(10) |
| 7.5 | −0.52354344064(6) | −1.0255139389(7) | −301.2827(2) | 0.00287639231(7) |
| 8.0 | −0.5223615610(2) | −1.029425970(2) | −244.4691(2) | 0.0019121440(2) |
| 8.5 | −0.52157938659(8) | −1.0324476628(10) | −185.03688(7) | 0.00126013063(9) |
| 9.0 | −0.52106500799(6) | −1.0346832263(7) | −131.02771(3) | 0.00082742108(7) |
| 9.5 | −0.52072721979(5) | −1.0362877893(5) | −86.713136(2) | 0.00054385792(5) |
| 10.0 | −0.52050473974(4) | −1.0374166367(4) | −52.97703(2) | 0.00035928428(3) |
| 11.0 | −0.52025843753(3) | −1.0387424313(2) | −11.87991(4) | 0.00016131307(2) |
| 12.0 | −0.52014531294(2) | −1.03937193512(4) | 6.74734(5) | 0.000076557564(2) |
| 13.0 | −0.520090104500(7) | −1.03967832617(3) | 15.02813(7) | 0.000038606372(2) |
| 14.0 | −0.52006198413(8) | −1.0398467946(10) | 18.6572(4) | 0.00001979812(6) |
| 15.0 | −0.5200465445(5) | −1.039907613(4) | 15.1207(10) | 0.0000123649(3) |
| 16.0 | −0.520036053(2) | −1.03992977(2) | 11.994(3) | 0.0000088960(9) |
| 17.0 | −0.520028379(3) | −1.03994471(3) | 10.208(5) | 0.000006590(2) |
| 18.0 | −0.520022648(6) | −1.03995592(5) | 9.064(9) | 0.000004964(4) |
| 19.0 | −0.52001830(2) | −1.03996441(8) | 8.21(2) | 0.000003797(6) |
| 20.0 | −0.52001495(3) | −1.0399709(2) | 7.51(2) | 0.000002946(9) |

TABLE S35. Calculated BO energies, expectation value of potential, $\langle \nabla_1 \cdot \nabla_2 \rangle$, and $\mathrm{d}E/\mathrm{d}R$ of the $3^1\Phi_u$ state in atomic units (hartree). Uncertainties originate purely from extrapolation to the complete basis set limit. United atom values at $R = 0$ are taken from Ref. [1].

| $3^1\Phi_\mathrm{u}$ | | | | |
|---|---|---|---|---|
| $R$ | $E$ | $\langle V \rangle$ | $10^6 \cdot \langle \nabla_1 \cdot \nabla_2 \rangle$ | $\mathrm{d}E/\mathrm{d}R$ |
| 0.0 | −2.0138906838155497(3) | – | 3.482257(7) | – |
| 0.01 | 97.986370681(2) | 95.973258826(10) | 3.4844(4) | −9999.9482535(8) |
| 0.05 | 17.992132738(5) | 15.99569678(5) | 3.502(2) | −399.7713739(7) |
| 0.1 | 8.007867339(8) | 6.05483748(5) | 3.537(8) | −99.6089720(4) |
| 0.15 | 4.697054638(7) | 2.80281698(5) | 3.596(8) | −43.9419486(2) |
| 0.2 | 3.057489402(6) | 1.23022148(4) | 3.659(8) | −24.4237866(2) |
| 0.3 | 1.452739489(5) | −0.23318393(4) | 3.775(9) | −10.46220969(8) |
| 0.4 | 0.685356793(2) | −0.863935186(7) | 0.438582(5) | −5.586621932(10) |
| 0.5 | 0.25112279694(8) | −1.1734362453(5) | 0.509420(10) | −3.3513636783(5) |
| 0.6 | −0.018704726(10) | −1.33211234(8) | 0.59(4) | −2.15783815(10) |
| 0.7 | −0.19651418382(2) | −1.411895858(4) | 0.68862(8) | −1.45552499(2) |
| 0.8 | −0.318369528927(6) | −1.4475561159(5) | 0.79820(4) | −1.013521325(3) |
| 0.9 | −0.404160021197(4) | −1.457557327(2) | 0.92216(2) | −0.72137475971(7) |
| 1.0 | −0.4656759562581(3) | −1.45231525301(2) | 1.06156(2) | −0.520963340496(6) |
| 1.1 | −0.510301631366(2) | −1.437985988285(8) | 1.18(3) | −0.379438841411(4) |
| 1.2 | −0.542864422339(2) | −1.418333458893(6) | 1.391582(2) | −0.277170511847(3) |
| 1.3 | −0.5666306659052(9) | −1.395716919707(5) | 1.58514(3) | −0.201888913766(3) |
| 1.4 | −0.5838737315725(8) | −1.371641152073(5) | 1.799973(9) | −0.145638349234(3) |
| 1.5 | −0.5962135825107(6) | −1.347076214617(4) | 2.038013(4) | −0.103099366397(2) |
| 1.6 | −0.6048277900056(6) | −1.322649813765(4) | 2.301439(2) | −0.070621396096(2) |
| 1.7 | −0.6105870393691(5) | −1.298766421990(4) | 2.62(6) | −0.045642554854(2) |
| 1.8 | −0.6141446252666(5) | −1.275682843380(4) | 2.9144903(5) | −0.026329773804(2) |
| 1.9 | −0.6159970136702(4) | −1.253557138198(4) | 3.2699146(4) | −0.011349005714(2) |
| 2.0 | −0.61652570465490(4) | −1.232480847652(4) | 3.6623987(4) | 0.000285280829(2) |
| 2.1 | −0.6160267167971(3) | −1.212500526066(3) | 4.0958028(3) | 0.009310908347(2) |
| 2.2 | −0.6147317016600(3) | −1.193632299059(3) | 4.5744619(3) | 0.016286865573(2) |
| 2.3 | −0.6128232908220(3) | −1.175871799137(9) | 5.1032447(9) | 0.021641209786(3) |
| 2.4 | −0.6104464008034(3) | −1.159200993845(9) | 5.6876247(9) | 0.025704919901(3) |
| 2.5 | −0.6077166614976(3) | −1.143592899373(9) | 6.3337520(9) | 0.028736169449(3) |
| 2.6 | −0.6047267690572(4) | −1.12901484006(2) | 7.2(2) | 0.030937960792(4) |
| 2.7 | −0.6015513221759(3) | −1.11543069915(2) | 7.839771(2) | 0.032471090816(4) |
| 2.8 | −0.5982505373650(3) | −1.10280246493(2) | 8.716188(2) | 0.033463789215(4) |
| 2.9 | −0.5948731268452(3) | −1.09109128189(2) | 9.687634(2) | 0.034018955793(4) |
| 3.0 | −0.5914585448392(2) | −1.08025815348(2) | 10.765180(2) | 0.034219645400(4) |
| 3.1 | −0.5880387532111(4) | −1.07026439928(2) | 11.961290(2) | 0.034133260368(4) |
| 3.2 | −0.5846396183225(5) | −1.06107193994(2) | 13.289987(2) | 0.033814780219(4) |
| 3.3 | −0.5812820227897(6) | −1.05264346206(2) | 14.767063(2) | 0.033309267732(4) |
| 3.4 | −0.5779827553127(6) | −1.044942500944(9) | 16.6(2) | 0.032653826377(3) |
| 3.5 | −0.574755226648(5) | −1.0379334687(2) | 18.23970(2) | 0.03187913846(5) |
| 3.6 | −0.571610048592(5) | −1.0315816469(2) | 20.27785(2) | 0.03101068064(5) |
| 3.7 | −0.568555504477(6) | −1.0258531606(3) | 22.55017(2) | 0.03006968876(6) |
| 3.8 | −0.565597933313(7) | −1.0207149413(3) | 25.08534(3) | 0.02907392773(6) |
| 3.9 | −0.562742044941(8) | −1.0161346895(3) | 27.91568(3) | 0.02803830779(7) |
| 4.0 | −0.559991179846(9) | −1.012080843(3) | 31.07771(3) | 0.0269753793(6) |
| 4.1 | −0.55734752449(8) | −1.008522542(3) | 34.61275(4) | 0.0258957334(7) |
| 4.2 | −0.55481229045(9) | −1.005429628(3) | 38.56746(4) | 0.0248083221(7) |
| 4.3 | −0.55238586501(10) | −1.002772630(4) | 42.99470(4) | 0.0237207210(8) |
| 4.4 | −0.5500679377(2) | −1.000522775(4) | 47.95445(4) | 0.0226393410(8) |
| 4.5 | −0.5478576076984(7) | −0.9986520110(4) | 53.51492(2) | 0.02156960098(7) |
| 4.6 | −0.545753476395(6) | −0.99713304872(9) | 59.753514(9) | 0.02051606610(2) |
| 4.7 | −0.54375372595(5) | −0.995939392(2) | 66.75866(5) | 0.0194825659(3) |
| 4.8 | −0.54185618856(5) | −0.995045403(2) | 74.63174(5) | 0.0184722863(3) |
| 4.9 | −0.540058406749(7) | −0.9944263622(2) | 83.48892(2) | 0.01748784720(3) |
| 5.0 | −0.538357686699(8) | −0.9940585473(6) | 93.46353(5) | 0.01653136523(10) |

## $3^1\Phi_u$ continued

| $R$ | $E$ | $\langle V\rangle$ | $10^6\cdot\langle\nabla_1\cdot\nabla_2\rangle$ | $\mathrm{d}E/\mathrm{d}R$ |
|---|---|---|---|---|
| 5.5 | −0.531204805490(2) | −0.9952380(5) | 166.477(4) | 0.01221301(9) |
| 6.0 | −0.526010811939(3) | −0.9998754(4) | 306.174(7) | 0.00869103(7) |
| 6.5 | −0.52240182944(3) | −1.0153707881(10) | 594.88348(4) | 0.0062215394(2) |
| 7.0 | −0.520148333856(10) | −1.0183195855(6) | 1204.53779(4) | 0.00313958316(8) |
| 7.5 | −0.519312191208(9) | −1.0359744090(3) | 1677.21594(6) | 0.00035332980(4) |
| 8.0 | −0.51943185407(3) | −1.0430578586(5) | 1260.9617(2) | −0.00052426880(6) |
| 8.5 | −0.51969016206(2) | −1.0432976061(6) | −185.03688(7) | −0.00046085671(6) |
| 9.0 | −0.51987895437(2) | −1.0346832263(7) | 574.26493(3) | 0.00082742108(7) |
| 9.5 | −0.51999344386(5) | −1.0362877893(5) | −86.713136(2) | 0.00054385792(5) |
| 10.0 | −0.52005576247(4) | −1.0374166367(4) | −52.97703(2) | 0.00035928428(3) |
| 11.0 | −0.52009584497(2) | −1.0387424313(2) | −11.87991(4) | 0.00016131307(2) |
| 12.0 | −0.52014531294(2) | −1.03937193512(4) | 6.74734(5) | 0.000076557564(2) |
| 13.0 | −0.52007292869(2) | −1.03967832616(3) | 15.02813(6) | 0.000038606372(2) |
| 14.0 | −0.52005510626(2) | −1.0398467946(10) | 18.6572(4) | 0.00001979812(6) |
| 15.0 | −0.52004009076(4) | −1.039907613(4) | 15.1207(10) | 0.0000123649(3) |
| 16.0 | −0.52002962633(3) | −1.03992977(2) | 10.124(2) | 0.0000088960(9) |
| 17.0 | −0.52002241065(2) | −1.03994236752(7) | 9.16775(2) | 0.000006026693(3) |
| 18.0 | −0.52001727456(2) | −1.03995608058(7) | 8.17076(3) | 0.000004359364(3) |
| 19.0 | −0.520013513811(6) | −1.03996562673(3) | 7.24007(3) | 0.0000032316258(6) |
| 20.0 | −0.520010699923(4) | −1.039983(9) | 3.1(4) | 0.00000213(6) |

TABLE S36. Calculated BO energies, expectation value of potential, $\langle\nabla_1 \cdot \nabla_2\rangle$, and $\mathrm{d}E/\mathrm{d}R$ of the $1^3\Phi_u$ state in atomic units (hartree). Uncertainties originate purely from extrapolation to the complete basis set limit. United atom values at $R = 0$ are taken from Ref. [1].

| $1^3\Phi_\mathrm{u}$ | | | | |
|---|---|---|---|---|
| $R$ | $E$ | $\langle V\rangle$ | $10^6\cdot\langle\nabla_1\cdot\nabla_2\rangle$ | $\mathrm{d}E/\mathrm{d}R$ |
| 0.0 | −2.031255144381749(1) | – | 9.6696396 | – |
| 0.01 | 97.969006203(2) | 95.938529859(2) | 9.67156(6) | −9999.9482549(4) |
| 0.05 | 17.974768311(3) | 2.01380028(2) | 9.71270(7) | −399.7713723(3) |
| 0.1 | 7.990503092(5) | 1.97039361(2) | 9.80968(9) | −99.6089674(2) |
| 0.15 | 4.67969072(2) | 2.76809032(8) | 9.92381(10) | −43.9419408(4) |
| 0.2 | 3.040125940(2) | 1.844629258(6) | 10.02976(10) | −24.42377605(3) |
| 0.3 | 1.435377404(2) | 1.703280494(5) | 10.14943(9) | −10.46219303(2) |
| 0.4 | 0.6679968441(5) | 1.56663896130(4) | 10.07066(7) | −5.586589517(2) |
| 0.5 | 0.2337665253(7) | 1.4418947630(3) | 9.73081(6) | −3.351322581(2) |
| 0.6 | −0.0360590474(9) | 1.33074100864(6) | 9.08366(6) | −2.157803273(2) |
| 0.7 | −0.213860522560(5) | −1.4465478341(2) | 8.09117(5) | −1.4554668414(2) |
| 0.8 | −0.335709638095(4) | −1.4821832003(2) | 6.71962(4) | −1.0134549052(2) |
| 0.9 | −0.421493082622(3) | −1.4921563967(2) | 4.93771(4) | −0.7213002572(2) |
| 1.0 | −0.483001171759(3) | −1.4868833045(2) | 2.71559(5) | −0.5208809610(2) |
| 1.1 | −0.527618224298(3) | −1.4725201371(2) | 0.02428(4) | −0.37934880777(10) |
| 1.2 | −0.560171638950(3) | −1.4528309491(2) | −3.16460(4) | −0.27707305935(9) |
| 1.3 | −0.583927776578(2) | −1.4301751298(2) | −6.87893(3) | −0.20178428970(7) |
| 1.4 | −0.601160031992(2) | −1.40605760125(10) | −11.14611(3) | −0.14552681233(7) |
| 1.5 | −0.613488394794(2) | −1.38144856932(10) | −15.99299(3) | −0.10298118648(6) |
| 1.6 | −0.622090463797(2) | −1.35697589376(10) | −21.44583(2) | −0.07049685385(5) |
| 1.7 | −0.627836952914(2) | −1.33304420660(9) | −27.53013(2) | −0.04551194163(5) |
| 1.8 | −0.631381186472(2) | −1.30991047756(9) | −34.27049(2) | −0.02619339145(5) |
| 1.9 | −0.633219661150(2) | −1.28773293859(9) | −41.69038(2) | −0.01120716647(4) |
| 2.0 | −0.633733908758(2) | −1.26660330845(9) | −49.81196(2) | 0.00043225453(4) |
| 2.1 | −0.633219980617(2) | −1.24656832474(9) | −58.655803(10) | 0.00946268405(4) |
| 2.2 | −0.631909562031(2) | −1.22764430184(9) | −68.240617(8) | 0.01644310101(4) |
| 2.3 | −0.629985319280(2) | −1.2098270663(3) | −78.58301(5) | 0.02180155315(9) |
| 2.4 | −0.627592204528(2) | −1.1930987845(3) | −89.69697(5) | 0.02586901024(9) |
| 2.5 | −0.624845884209(2) | −1.1774326759(3) | −101.59377(4) | 0.02890363701(9) |
| 2.6 | −0.621839091869(2) | −1.1627962722(3) | −114.28146(4) | 0.03110842751(9) |
| 2.7 | −0.618646464398(2) | −1.1491536673(3) | −127.76446(4) | 0.03264417094(9) |
| 2.8 | −0.615328257241(2) | −1.1364670626(3) | −142.04318(4) | 0.03363908996(9) |
| 2.9 | −0.611933222213(3) | −1.1246978177(3) | −157.11360(4) | 0.03419607819(9) |
| 3.0 | −0.608500853706(3) | −1.1138071518(3) | −172.96681(4) | 0.03439818522(9) |
| 3.1 | −0.605063154225(3) | −1.103756599(3) | −189.5908(2) | 0.0343128096(7) |
| 3.2 | −0.601646031126(3) | −1.094508298(6) | −206.962(2) | 0.033994926(2) |
| 3.3 | −0.598270408238(3) | −1.086025140(6) | −225.055(3) | 0.033489599(2) |
| 3.4 | −0.594953115536(3) | −1.078270869(5) | −243.837(2) | 0.032833930(2) |
| 3.5 | −0.591707604938(3) | −1.071210094(5) | −263.269(2) | 0.032058605(2) |
| 3.6 | −0.588544529082(3) | −1.064808288(5) | −283.304(2) | 0.031189103(2) |
| 3.7 | −0.585472211591(3) | −1.059031753(5) | −303.887(2) | 0.030246668(2) |
| 3.8 | −0.582497030953(3) | −1.053847582(5) | −324.956(2) | 0.029249074(2) |
| 3.9 | −0.579623735368(3) | −1.049223619(5) | −346.439(2) | 0.0282112440(10) |
| 4.0 | −0.576855702214(3) | −1.0451284205(5) | −368.25590(7) | 0.02714574600(10) |
| 4.1 | −0.57419515294(4) | −1.0415312252(5) | −390.32413(8) | 0.0260631904(2) |
| 4.2 | −0.57164333192(2) | −1.0384019300(2) | −412.54621(2) | 0.02497255567(5) |
| 4.3 | −0.56920065625(2) | −1.0357110825(2) | −434.81947(2) | 0.02388144883(4) |
| 4.4 | −0.56686684183(2) | −1.0334298809(2) | −457.03355(2) | 0.02279631882(4) |
| 4.5 | −0.564641010184(4) | −1.0315301862(5) | −479.07127(8) | 0.02172262982(10) |
| 4.6 | −0.56252177965(4) | −1.0299845444(5) | −500.80885(8) | 0.02066500324(10) |
| 4.7 | −0.56050734359(2) | −1.0287662175(2) | −522.11708(2) | 0.01962733397(4) |
| 4.8 | −0.55859553818(2) | −1.0278492219(2) | −542.86231(2) | 0.01861288635(4) |
| 4.9 | −0.55678390128(2) | −1.0272083706(2) | −562.90703(2) | 0.01762437388(4) |
| 5.0 | −0.555069724117(5) | −1.026819321(2) | −582.1119(4) | 0.0166640254(4) |

$1^3\Phi_u$ continued

| $R$ | $E$ | $\langle V \rangle$ | $10^6 \cdot \langle \nabla_1 \cdot \nabla_2 \rangle$ | $\mathrm{d}E/\mathrm{d}R$ |
|---|---|---|---|---|
| 5.5 | −0.547853992970(6) | −1.027863799(4) | −660.6650(10) | 0.0123353067(6) |
| 6.0 | −0.542593703654(8) | −1.032109356(6) | −698.702(2) | 0.0088463419(8) |
| 6.5 | −0.538872390465(3) | −1.03766187147(4) | −686.344169(10) | 0.006166601455(5) |
| 7.0 | −0.536309297103(3) | −1.04326900128(3) | −624.861878(9) | 0.004192798989(4) |
| 7.5 | −0.534583952898(3) | −1.04822186664(3) | −527.566535(8) | 0.002792805221(3) |
| 8.0 | −0.533443284961(3) | −1.05222624251(3) | −414.648359(6) | 0.001832540926(3) |
| 8.5 | −0.532698291425(2) | −1.05526652980(3) | −304.971616(5) | 0.001191770947(3) |
| 9.0 | −0.532214718070(2) | −1.05747589429(2) | −210.525555(5) | 0.000772615761(2) |
| 9.5 | −0.531901082632(2) | −1.05903547971(2) | −135.817619(4) | 0.000501756374(2) |
| 10.0 | −0.531696913839(2) | −1.06011634734(2) | −80.239065(5) | 0.000327748034(2) |
| 11.0 | −0.531474229405(2) | −1.061361485032(10) | −13.764467(4) | 0.0001442703435(8) |
| 12.0 | −0.5313737090811(7) | −1.061936285721(7) | 15.380349(3) | 0.0000675943701(5) |
| 13.0 | −0.5313249268428(5) | −1.062202572792(4) | 26.038869(2) | 0.0000344062226(2) |
| 14.0 | −0.5312990548842(4) | −1.062329276477(3) | 28.4058044(6) | 0.00001920237798(10) |
| 15.0 | −0.5312840217927(3) | −1.0623928030517(7) | 27.38279543(2) | 0.000011682702246(7) |
| 16.0 | −0.5312745608524(3) | −1.0624271611879(7) | 25.1657628(6) | 0.00000762253225(7) |
| 17.0 | −0.5312682290794(2) | −1.062447456584(2) | 22.681118(2) | 0.0000052353867(2) |
| 18.0 | −0.5312638010996(3) | −1.062460500634(6) | 20.291101(2) | 0.0000037278647(4) |
| 19.0 | −0.5312606076799(4) | −1.062469478818(9) | 18.118121(3) | 0.0000027229758(5) |
| 20.0 | −0.5312582531696(7) | −1.06247597261(2) | 16.187408(4) | 0.0000020266862(8) |

TABLE S37. Calculated BO energies, expectation value of potential, $\langle \nabla_1 \cdot \nabla_2 \rangle$, and $\mathrm{d}E/\mathrm{d}R$ of the $2^3\Phi_u$ state in atomic units (hartree). Uncertainties originate purely from extrapolation to the complete basis set limit. United atom values at $R = 0$ are taken from Ref. [1].

| $2^3\Phi_\mathrm{u}$ | | | | |
|---|---|---|---|---|
| $R$ | $E$ | $\langle V \rangle$ | $10^6 \cdot \langle \nabla_1 \cdot \nabla_2 \rangle$ | $\mathrm{d}E/\mathrm{d}R$ |
| 0.0 | −2.0200029371587427(5) | − | 5.4064900(5) | − |
| 0.01 | 97.9802584074(3) | 95.961034275(3) | 5.4068(4) | −9999.9482540(2) |
| 0.05 | 17.986020475(4) | 15.98347227(3) | 5.427(3) | −399.7713735(4) |
| 0.1 | 8.001755135(4) | 6.04261318(3) | 5.477(7) | −99.6089711(3) |
| 0.15 | 4.690942521(4) | 2.79059307(3) | 5.557(3) | −43.9419465(2) |
| 0.2 | 3.051377424(6) | 1.21799813(2) | 5.623(7) | −24.4237837(2) |
| 0.3 | 1.446627913(3) | −0.24540561(2) | 5.746(2) | −10.46220480(4) |
| 0.4 | 0.679245966(2) | −0.876150310(10) | 5.72(3) | −5.58660560(2) |
| 0.5 | 0.2450138252(6) | −1.185643805(5) | 5.6545(7) | −3.351342910(8) |
| 0.6 | −0.0248139931(5) | −1.344324670(5) | 5.394(2) | −2.157827806(6) |
| 0.7 | −0.2026181282(4) | −1.424083121(4) | 4.961(2) | −1.455495521(5) |
| 0.8 | −0.3244703148(7) | −1.45973073(2) | 4.333(4) | −1.01348763(2) |
| 0.9 | −0.4102572302(4) | −1.469717699(4) | 3.509(2) | −0.721336932(4) |
| 1.0 | −0.4717691800(7) | −1.464459840(8) | 2.455(3) | −0.520921480(6) |
| 1.1 | −0.5163904720(3) | −1.450113310(4) | 1.168(2) | −0.379393060(3) |
| 1.2 | −0.5489484936(7) | −1.430442098(8) | −0.375(3) | −0.277120926(5) |
| 1.3 | −0.5727095934(3) | −1.407805526(4) | −2.182(2) | −0.201835645(3) |
| 1.4 | −0.5899471534(6) | −1.383708444(8) | −4.274(3) | −0.145581527(5) |
| 1.5 | −0.6022811499(6) | −1.359120983(7) | −6.660(3) | −0.103039122(4) |
| 1.6 | −0.6108891676(6) | −1.334670924(7) | −9.355(3) | −0.070557868(4) |
| 1.7 | −0.6166419058(6) | −1.310762816(8) | −12.373(3) | −0.045575885(4) |
| 1.8 | −0.6201926735(3) | −1.287653541(4) | −15.724(2) | −0.026260108(2) |
| 1.9 | −0.6220379519(6) | −1.265501245(8) | −19.428(3) | −0.011276496(4) |
| 2.0 | −0.6225592559(3) | −1.244397549(4) | −23.487(2) | 0.000360481(2) |
| 2.1 | −0.6220526202(6) | −1.224389096(8) | −27.921(3) | 0.009388640(3) |
| 2.2 | −0.6207497119(3) | −1.205492096(4) | −32.731(2) | 0.016366967(2) |
| 2.3 | −0.6188331794(6) | −1.187702272(8) | −37.936(3) | 0.021723516(3) |
| 2.4 | −0.6164479554(6) | −1.171001680(8) | −43.535(3) | 0.025789263(3) |
| 2.5 | −0.6137096870(6) | −1.155363425(8) | −49.539(3) | 0.028822380(3) |
| 2.6 | −0.6107110872(7) | −1.140754921(8) | −55.951(3) | 0.031025867(3) |
| 2.7 | −0.6075267721(7) | −1.127140140(8) | −62.775(3) | 0.032560520(3) |
| 2.8 | −0.6042169753(7) | −1.114481158(9) | −70.012(4) | 0.033554569(3) |
| 2.9 | −0.6008304265(7) | −1.102739204(9) | −77.661(4) | 0.034110913(3) |
| 3.0 | −0.5974065969(7) | −1.091875364(9) | −85.718(4) | 0.034312610(3) |
| 3.1 | −0.5939774655(7) | −1.081851035(9) | −94.178(4) | 0.034227063(3) |
| 3.2 | −0.5905689153(8) | −1.072628210(10) | −103.032(4) | 0.033909256(3) |
| 3.3 | −0.5872018451(8) | −1.064169640(10) | −112.269(4) | 0.033404258(3) |
| 3.4 | −0.5838930593(8) | −1.056438918(2) | −121.872(4) | 0.032749177(3) |
| 3.5 | −0.5806559835(8) | −1.04940050(2) | −131.825(4) | 0.031974704(3) |
| 3.6 | −0.5775012437(8) | −1.04301971(2) | −142.105(4) | 0.031106327(3) |
| 3.7 | −0.5744371360(9) | −1.03726268(2) | −152.687(5) | 0.030165294(3) |
| 3.8 | −0.5714700109(9) | −1.03209639(5) | −163.55(2) | 0.029169378(9) |
| 3.9 | −0.5686045881(10) | −1.02748842(2) | −174.638(5) | 0.028133526(3) |
| 4.0 | −0.5658442158(5) | −1.023407263(7) | −185.933(2) | 0.027070292(2) |
| 4.1 | −0.5631910865(10) | −1.01982196(2) | −197.396(5) | 0.025990295(3) |
| 4.2 | −0.5606464145(6) | −1.016702252(7) | −208.979(8) | 0.024902518(2) |
| 4.3 | −0.5582105871(4) | −1.014018524(5) | −220.73(6) | 0.0238145697(10) |
| 4.4 | −0.5558832901(4) | −1.011741823(6) | −232.44(9) | 0.0227328993(10) |
| 4.5 | −0.5536636149(7) | −1.009843861(9) | −243.912(2) | 0.021662971(2) |
| 4.6 | −0.551550150(2) | −1.00829704(2) | −255.448(6) | 0.020609403(4) |
| 4.7 | −0.5495410583(6) | −1.007074497(8) | −266.8173(3) | 0.019576089(2) |
| 4.8 | −0.5476341474(5) | −1.006150123(6) | −278.3(2) | 0.0185662857(10) |
| 4.9 | −0.5458269267(5) | −1.005498634(7) | −289.1(2) | 0.017582698(2) |
| 5.0 | −0.5441166596(5) | −1.005095601(7) | −299.38(2) | 0.016627544(2) |

| $2^3\Phi_u$ continued | | | | |
|---|---|---|---|---|
| $R$ | $E$ | $\langle V\rangle$ | $10^6\cdot\langle\nabla_1\cdot\nabla_2\rangle$ | $\mathrm{d}E/\mathrm{d}R$ |
| 5.5 | −0.536912033(2) | −1.00601892(6) | −344.34(3) | 0.012328209(8) |
| 6.0 | −0.531647227(2) | −1.01006487(6) | −370.84(3) | 0.008871597(8) |
| 6.5 | −0.52790560250(6) | −1.0153707981(9) | −373.0523(2) | 0.0062216011(2) |
| 7.0 | −0.52530933295(5) | −1.0207387992(7) | −349.71273(7) | 0.00426855239(8) |
| 7.5 | −0.5235435851(2) | −1.025513793(2) | −304.9681(5) | 0.0028764503(2) |
| 8.0 | −0.52236167791(9) | −1.029425791(2) | −247.5454(4) | 0.0019121957(2) |
| 8.5 | −0.52157947961(7) | −1.0324474750(9) | −187.5679(3) | 0.00126017461(8) |
| 9.0 | −0.52106508099(5) | −1.0346830467(6) | −133.0902(2) | 0.00082745726(6) |
| 9.5 | −0.52072727651(4) | −1.0362876264(5) | −88.3840(2) | 0.00054388701(4) |
| 10.0 | −0.52050478347(6) | −1.037416494(2) | −54.32612(7) | 0.00035930737(5) |
| 11.0 | −0.52025846285(2) | −1.0387423234(2) | −12.75342(8) | 0.00016132748(2) |
| 12.0 | −0.52014532668(2) | −1.03937185144(4) | 6.19403(7) | 0.000076566827(2) |
| 13.0 | −0.52009011055(4) | −1.0396782570(2) | 14.7125(4) | 0.000038612626(3) |
| 14.0 | −0.52006198708(8) | −1.0398468167(10) | 18.5230(4) | 0.00001979696(6) |
| 15.0 | −0.5200465490(5) | −1.039907633(4) | 15.0051(9) | 0.0000123642(3) |
| 16.0 | −0.520036057(2) | −1.03992977(2) | 11.888(3) | 0.0000088965(9) |
| 17.0 | −0.520028383(3) | −1.03994471(3) | 10.119(5) | 0.000006591(2) |
| 18.0 | −0.52002264616(2) | −1.0399558723(2) | 9.00165(8) | 0.000004967778(5) |
| 19.0 | −0.52001830(2) | −1.03996441(8) | 8.15(2) | 0.000003797(6) |
| 20.0 | −0.52001496(3) | −1.0399709(2) | 7.469(10) | 0.000002946(9) |

TABLE S38. Calculated BO energies, expectation value of potential, $\langle\nabla_1 \cdot \nabla_2\rangle$, and $\mathrm{d}E/\mathrm{d}R$ of the $3^3\Phi_u$ state in atomic units (hartree). Uncertainties originate purely from extrapolation to the complete basis set limit. United atom values at $R = 0$ are taken from Ref. [1].

| $3^3\Phi_\mathrm{u}$ | | | | |
|---|---|---|---|---|
| $R$ | $E$ | $\langle V\rangle$ | $10^6 \cdot \langle\nabla_1 \cdot \nabla_2\rangle$ | $\mathrm{d}E/\mathrm{d}R$ |
| 0.0 | −2.0138906838155497(3) | − | 3.2684586(8) | − |
| 0.01 | 97.986370665(2) | 95.973258795(9) | 3.265(2) | −9999.9482535(6) |
| 0.05 | 17.992132720(6) | 15.99569675(4) | 3.273(5) | −399.7713739(6) |
| 0.1 | 8.007867323(8) | 6.05483744(5) | 3.29(2) | −99.6089720(4) |
| 0.15 | 4.697054619(8) | 2.80281694(5) | 3.33(2) | −43.9419486(2) |
| 0.2 | 3.057489384(6) | 1.23022144(4) | 3.38(2) | −24.4237867(2) |
| 0.3 | 1.452739469(4) | −0.23318398(3) | 3.45(2) | −10.46220973(7) |
| 0.4 | 0.6853567941(10) | −0.863935186(7) | 0.438586(7) | −5.58662193(2) |
| 0.5 | 0.25112279694(8) | −1.1734362453(5) | 0.50942(8) | −3.3513636783(5) |
| 0.6 | −0.01870476(2) | −1.33211242(9) | 0.58(6) | −2.1578382(2) |
| 0.7 | −0.19651418382(2) | −1.411895858(4) | 0.68861(8) | −1.45552499(2) |
| 0.8 | −0.318369528927(6) | −1.4475561159(5) | 0.79820(4) | −1.013521325(3) |
| 0.9 | −0.404160021198(4) | −1.457557327(2) | 0.92216(2) | −0.72137475971(7) |
| 1.0 | −0.4656759562583(3) | −1.45231525302(2) | 1.0615524(5) | −0.520963340497(6) |
| 1.1 | −0.510301631367(2) | −1.437985988287(8) | 1.2175647(2) | −0.379438841412(4) |
| 1.2 | −0.542864422339(2) | −1.418333458895(6) | 1.3915802(3) | −0.277170511848(3) |
| 1.3 | −0.5666306659057(9) | −1.395716919708(5) | 1.585137(3) | −0.201888913767(3) |
| 1.4 | −0.5838737315730(8) | −1.371641152075(5) | 1.799965(2) | −0.145638349235(3) |
| 1.5 | −0.5962135825113(6) | −1.347076214620(4) | 2.0380027(8) | −0.103099366398(2) |
| 1.6 | −0.6048277900063(6) | −1.322649813769(4) | 2.3014257(5) | −0.070621396098(2) |
| 1.7 | −0.6105870393700(5) | −1.298766421995(4) | 2.5926711(5) | −0.045642554856(2) |
| 1.8 | −0.6141446252677(5) | −1.275682843386(4) | 2.9144716(4) | −0.026329773806(2) |
| 1.9 | −0.6159970136714(4) | −1.253557138204(4) | 3.2698923(4) | −0.011349005716(2) |
| 2.0 | −0.61652570465639(4) | −1.232480847660(4) | 3.6623722(4) | 0.000285280827(2) |
| 2.1 | −0.6160267167988(3) | −1.212500526075(3) | 4.0957715(4) | 0.009310908344(2) |
| 2.2 | −0.6147317016620(3) | −1.193632299070(3) | 4.5744249(4) | 0.016286865570(2) |
| 2.3 | −0.6128232908244(3) | −1.175871799151(9) | 5.1032010(10) | 0.021641209782(3) |
| 2.4 | −0.6104464008062(3) | −1.159200993861(9) | 5.6875736(10) | 0.025704919897(3) |
| 2.5 | −0.6077166615009(3) | −1.143592899391(9) | 6.3336922(10) | 0.028736169445(3) |
| 2.6 | −0.6047267690609(4) | −1.12901484008(2) | 7.048472(2) | 0.030937960787(4) |
| 2.7 | −0.6015513221802(3) | −1.11543069918(2) | 7.839690(2) | 0.032471090809(4) |
| 2.8 | −0.5982505373699(4) | −1.10280246496(2) | 8.716095(2) | 0.033463789208(4) |
| 2.9 | −0.5948731268509(3) | −1.09109128193(2) | 9.687525(2) | 0.034018955785(4) |
| 3.0 | −0.5914585448457(4) | −1.08025815352(2) | 10.765055(2) | 0.034219645392(4) |
| 3.1 | −0.5880387532185(4) | −1.07026439933(2) | 11.961146(3) | 0.034133260358(4) |
| 3.2 | −0.5846396183309(5) | −1.06107194000(2) | 13.289822(3) | 0.033814780208(4) |
| 3.3 | −0.5812820227994(6) | −1.05264346212(2) | 14.766873(3) | 0.033309267719(4) |
| 3.4 | −0.5779827553235(6) | −1.044942501012(8) | 16.410081(2) | 0.032653826363(3) |
| 3.5 | −0.574755226661(5) | −1.0379334688(2) | 18.23945(2) | 0.03187913844(5) |
| 3.6 | −0.571610048607(5) | −1.0315816470(2) | 20.27757(3) | 0.03101068062(5) |
| 3.7 | −0.568555504493(6) | −1.0258531607(3) | 22.54985(3) | 0.03006968874(6) |
| 3.8 | −0.565597933331(7) | −1.0207149414(3) | 25.08496(3) | 0.02907392771(6) |
| 3.9 | −0.562742044961(8) | −1.0161346896(3) | 27.91526(4) | 0.02803830777(7) |
| 4.0 | −0.559991179869(9) | −1.012080843(3) | 31.07722(4) | 0.0269753793(6) |
| 4.1 | −0.55734752451(8) | −1.008522542(3) | 34.61219(4) | 0.0258957333(7) |
| 4.2 | −0.55481229048(9) | −1.005429628(3) | 38.56682(5) | 0.0248083220(7) |
| 4.3 | −0.55238586505(10) | −1.002772630(4) | 42.99398(5) | 0.0237207210(8) |
| 4.4 | −0.5500679377(2) | −1.000522775(4) | 47.95364(6) | 0.0226393409(8) |
| 4.5 | −0.547857607740(5) | −0.9986520113(4) | 53.51402(3) | 0.02156960094(7) |
| 4.6 | −0.54575347645(3) | −0.9971330492(4) | 59.75248(3) | 0.02051606602(7) |
| 4.7 | −0.54375372600(5) | −0.995939393(2) | 66.75750(6) | 0.0194825658(3) |
| 4.8 | −0.54185618862(5) | −0.995045403(2) | 74.63044(7) | 0.0184722863(3) |
| 4.9 | −0.54005840683(7) | −0.994426364(2) | 83.48732(8) | 0.0174878470(4) |
| 5.0 | −0.538357686766(7) | −0.9940585477(6) | 93.46193(6) | 0.01653136516(10) |

| $3^3\Phi_u$ continued | | | | |
|---|---|---|---|---|
| $R$ | $E$ | $\langle V \rangle$ | $10^6 \cdot \langle \nabla_1 \cdot \nabla_2 \rangle$ | $\mathrm{d}E/\mathrm{d}R$ |
| 5.5 | −0.531204805589(2) | −1.00601892(6) | 166.474(5) | 0.012328209(8) |
| 6.0 | −0.526010812058(2) | −1.01006487(6) | 306.170(8) | 0.008871597(8) |
| 6.5 | −0.52240182955(3) | −1.0153707981(9) | 594.87904(4) | 0.0062216011(2) |
| 7.0 | −0.520148334675(9) | −1.0183196182(6) | 1204.51984(4) | 0.00313957873(8) |
| 7.5 | −0.519312197820(6) | −1.0359745500(2) | 1677.077636(7) | 0.00035331276(2) |
| 8.0 | −0.51943186802(2) | −1.0430579754(4) | 1260.66730(2) | −0.00052427992(4) |
| 8.5 | −0.51969018011(2) | −1.0432976917(4) | 847.78109(5) | −0.00046086253(5) |
| 9.0 | −0.51987897450(2) | −1.0346830467(6) | −133.0902(2) | 0.00082745726(6) |
| 9.5 | −0.51999346483(2) | −1.0362876264(5) | −135.81770(9) | 0.00054388701(4) |
| 10.0 | −0.520055783461(10) | −1.0409764964(2) | 267.236170(9) | −0.00008649295(2) |
| 11.0 | −0.520095864738(9) | −1.0402801749(2) | 125.174264(8) | −0.000008040489(2) |
| 12.0 | −0.520090005097(10) | −1.03937185144(4) | 59.402272(9) | 0.000076566827(2) |
| 13.0 | −0.52007294527(2) | −1.0399104045(2) | 28.392146(9) | 0.00001811431(2) |
| 14.0 | −0.52005511963(3) | −1.0398707162(2) | 13.27996(5) | 0.000017108789(8) |
| 15.0 | −0.52004009809(2) | −1.03989101360(3) | 10.62611(2) | 0.0000126121714(4) |
| 16.0 | −0.52002963058(7) | −1.0399216683(7) | 9.936(2) | 0.00000859955(4) |
| 17.0 | −0.52002241327(3) | −1.0399423525(2) | 9.0324(3) | 0.000006027885(7) |
| 18.0 | −0.52001727626(4) | −1.03995607103(5) | 8.069(2) | 0.00000436007(2) |
| 19.0 | −0.52001351494(3) | −1.0399656206(3) | 7.1692(4) | 0.00000323207(2) |
| 20.0 | −0.520010700677(3) | −1.0399725802(4) | 6.35214(7) | 0.0000024410739(5) |

[1] G. Drake, in *Springer Handbook of Atomic, Molecular, and Optical Physics*, edited by D. Gordon (Springer New York, New York, NY, 2006), pp. 199–219.
